# Supplementary material for: The 2021 outburst of the recurrent nova RS Ophiuchi observed in X-rays by the Neil Gehrels Swift Observatory: a comparative study
Source: arXiv:2205.03232 ancillary file (2022-05-06)
Supplement: Supplementary file 1 [file table.pdf]

Table 1: Fits to the XRT spectra before (model consisting of two absorbed APEC components) and during (including an additional BB) the SSS phases in 2006 and 2021, as plotted in Fig. 11 of the manuscript. The first column lists the mid-point of the spectrum in days since the optical peak of the eruption, while the second column provides the excess absorption. Columns three to five list the temperatures of the BB and APEC components, while columns six and seven show the observed flux over 0.3–10 keV for the BB and combined APEC components, respectively. The final column gives the Cash statistic and number of degrees of freedom. Where only a single APEC temperature is listed, the other component was not statistically required.

| $T_{\text{mid}}$<br>(day) | $N_{\text{H}}$<br>( $10^{22} \text{ cm}^{-2}$ ) | $kT_{\text{BB}}$<br>(eV) | APEC $kT_{\text{cool}}$<br>(keV) | APEC $kT_{\text{hot}}$<br>(keV) | BB Flux<br>( $\text{erg cm}^{-2} \text{ s}^{-1}$ ) | APEC Flux<br>( $\text{erg cm}^{-2} \text{ s}^{-1}$ ) | Cstat/dof    |
|---------------------------|-------------------------------------------------|--------------------------|----------------------------------|---------------------------------|----------------------------------------------------|------------------------------------------------------|--------------|
| <b>2006 eruption</b>      |                                                 |                          |                                  |                                 |                                                    |                                                      |              |
| 3.178                     | $6.77^{+0.40}_{-0.38}$                          | —                        | $0.168^{+0.023}_{-0.028}$        | $8.449^{+0.637}_{-0.576}$       | —                                                  | $1.30^{+0.02}_{-0.02} \times 10^{-9}$                | 903.6 / 799  |
| 5.033                     | $2.47^{+0.10}_{-0.09}$                          | —                        | $0.248^{+0.017}_{-0.024}$        | $7.407^{+0.312}_{-0.310}$       | —                                                  | $2.01^{+0.02}_{-0.02} \times 10^{-9}$                | 1175.1 / 854 |
| 8.183                     | $1.68^{+0.10}_{-0.10}$                          | —                        | $0.280^{+0.017}_{-0.017}$        | $5.964^{+0.335}_{-0.268}$       | —                                                  | $1.11^{+0.01}_{-0.01} \times 10^{-9}$                | 1007.5 / 781 |
| 10.99                     | $1.75^{+0.16}_{-0.20}$                          | —                        | $0.192^{+0.041}_{-0.028}$        | $2.976^{+0.199}_{-0.165}$       | —                                                  | $6.50^{+0.17}_{-0.18} \times 10^{-10}$               | 655.4 / 602  |
| 11.057                    | $1.55^{+0.19}_{-0.20}$                          | —                        | $0.263^{+0.039}_{-0.054}$        | $3.208^{+0.294}_{-0.251}$       | —                                                  | $6.97^{+0.23}_{-0.21} \times 10^{-10}$               | 563.1 / 574  |
| 11.124                    | $2.07^{+0.02}_{-0.08}$                          | —                        | $0.138^{+0.011}_{-0.007}$        | $2.688^{+0.093}_{-0.082}$       | —                                                  | $6.79^{+0.19}_{-0.12} \times 10^{-10}$               | 574.4 / 585  |
| 13.605                    | $1.56^{+0.10}_{-0.11}$                          | —                        | $0.200^{+0.019}_{-0.012}$        | $2.535^{+0.101}_{-0.074}$       | —                                                  | $4.82^{+0.08}_{-0.08} \times 10^{-10}$               | 749.4 / 659  |
| 15.616                    | $1.54^{+0.06}_{-0.06}$                          | —                        | $0.621^{+0.020}_{-0.058}$        | $2.782^{+0.109}_{-0.096}$       | —                                                  | $3.89^{+0.06}_{-0.06} \times 10^{-10}$               | 890.9 / 639  |
| 18.176                    | $1.54^{+0.11}_{-0.13}$                          | —                        | $0.800^{+0.044}_{-0.038}$        | $2.533^{+0.256}_{-0.203}$       | —                                                  | $2.31^{+0.09}_{-0.04} \times 10^{-10}$               | 408.5 / 437  |
| 18.229                    | $1.50^{+0.16}_{-0.18}$                          | —                        | $0.844^{+0.064}_{-0.070}$        | $2.427^{+0.630}_{-0.380}$       | —                                                  | $2.29^{+0.08}_{-0.10} \times 10^{-10}$               | 257.0 / 311  |
| 18.239                    | $1.54^{+0.11}_{-0.13}$                          | —                        | $0.665^{+0.056}_{-0.051}$        | $2.597^{+0.289}_{-0.212}$       | —                                                  | $2.89^{+0.10}_{-0.10} \times 10^{-10}$               | 447.0 / 461  |
| 25.998                    | $1.37^{+0.04}_{-0.05}$                          | $28.1^{+1.6}_{-0.8}$     | $0.672^{+0.040}_{-0.015}$        | $2.047^{+0.156}_{-0.127}$       | $1.11^{+0.06}_{-0.06} \times 10^{-11}$             | $1.70^{+0.03}_{-0.03} \times 10^{-10}$               | 665.9 / 499  |
| 29.01                     | $0.94^{+0.03}_{-0.02}$                          | $18.1^{+0.3}_{-0.4}$     | $0.701^{+0.015}_{-0.015}$        | $1.569^{+0.047}_{-0.059}$       | $2.74^{+0.02}_{-0.02} \times 10^{-10}$             | $1.48^{+0.02}_{-0.02} \times 10^{-10}$               | 715.8 / 467  |
| 29.886                    | $0.65^{+0.03}_{-0.04}$                          | $25.1^{+1.0}_{-0.6}$     | $0.707^{+0.038}_{-0.016}$        | $1.602^{+0.056}_{-0.038}$       | $8.73^{+0.13}_{-0.13} \times 10^{-11}$             | $1.30^{+0.02}_{-0.02} \times 10^{-10}$               | 836.0 / 432  |
| 31.02                     | $0.77^{+0.06}_{-0.06}$                          | $18.7^{+1.3}_{-0.9}$     | $0.628^{+0.014}_{-0.014}$        | $1.573^{+0.042}_{-0.042}$       | $4.68^{+0.09}_{-0.10} \times 10^{-11}$             | $1.30^{+0.02}_{-0.02} \times 10^{-10}$               | 818.6 / 439  |
| 32.024                    | $0.95^{+0.03}_{-0.01}$                          | $19.0^{+0.2}_{-0.2}$     | $0.663^{+0.014}_{-0.014}$        | $1.480^{+0.057}_{-0.077}$       | $3.71^{+0.02}_{-0.02} \times 10^{-10}$             | $1.26^{+0.02}_{-0.02} \times 10^{-10}$               | 796.3 / 426  |
| 32.821                    | $0.78^{+0.03}_{-0.03}$                          | $20.6^{+0.5}_{-0.5}$     | $0.738^{+0.065}_{-0.098}$        | $1.417^{+0.233}_{-0.159}$       | $1.27^{+0.01}_{-0.01} \times 10^{-9}$              | $9.64^{+0.50}_{-0.48} \times 10^{-11}$               | 248.9 / 233  |
| 32.907                    | $0.76^{+0.02}_{-0.02}$                          | $27.9^{+0.5}_{-0.3}$     | $0.557^{+0.067}_{-0.066}$        | $1.381^{+0.081}_{-0.077}$       | $1.75^{+0.01}_{-0.01} \times 10^{-9}$              | $1.10^{+0.04}_{-0.04} \times 10^{-10}$               | 356.4 / 271  |
| 32.956                    | $0.74^{+0.02}_{-0.02}$                          | $28.0^{+0.4}_{-0.4}$     | $0.742^{+0.092}_{-0.095}$        | $1.384^{+0.183}_{-0.141}$       | $1.95^{+0.01}_{-0.01} \times 10^{-9}$              | $9.40^{+0.44}_{-0.43} \times 10^{-11}$               | 267.9 / 254  |
| 32.973                    | $0.78^{+0.02}_{-0.02}$                          | $28.2^{+0.4}_{-0.4}$     | $0.851^{+0.053}_{-0.049}$        | $1.826^{+0.495}_{-0.285}$       | $1.79^{+0.01}_{-0.01} \times 10^{-9}$              | $9.72^{+0.53}_{-0.48} \times 10^{-11}$               | 285.3 / 260  |
| 33.032                    | $0.62^{+0.01}_{-0.01}$                          | $28.3^{+0.2}_{-0.3}$     | $0.784^{+0.038}_{-0.048}$        | $1.513^{+0.079}_{-0.081}$       | $1.85^{+0.01}_{-0.01} \times 10^{-9}$              | $1.03^{+0.03}_{-0.03} \times 10^{-10}$               | 602.4 / 319  |
| 33.107                    | $1.00^{+0.02}_{-0.03}$                          | $21.4^{+0.4}_{-0.3}$     | $0.898^{+0.029}_{-0.029}$        | —                               | $1.86^{+0.01}_{-0.01} \times 10^{-9}$              | $1.00^{+0.06}_{-0.06} \times 10^{-10}$               | 308.2 / 244  |
| 33.17                     | $0.99^{+0.05}_{-0.07}$                          | $18.4^{+0.9}_{-0.7}$     | $0.507^{+0.108}_{-0.142}$        | $1.344^{+0.277}_{-0.162}$       | $1.37^{+0.03}_{-0.03} \times 10^{-9}$              | $9.59^{+0.96}_{-0.83} \times 10^{-11}$               | 122.9 / 159  |
| 33.178                    | $1.18^{+0.04}_{-0.03}$                          | $19.3^{+0.4}_{-0.3}$     | $0.576^{+0.064}_{-0.062}$        | $1.090^{+0.125}_{-0.092}$       | $1.57^{+0.01}_{-0.01} \times 10^{-9}$              | $8.35^{+0.40}_{-0.37} \times 10^{-11}$               | 218.1 / 223  |
| 33.242                    | $1.11^{+0.02}_{-0.03}$                          | $19.7^{+0.4}_{-0.2}$     | $0.605^{+0.129}_{-0.120}$        | $0.954^{+0.076}_{-0.053}$       | $1.64^{+0.01}_{-0.01} \times 10^{-9}$              | $9.40^{+0.32}_{-0.31} \times 10^{-11}$               | 306.0 / 278  |
| 33.309                    | $0.70^{+0.06}_{-0.07}$                          | $19.9^{+1.4}_{-1.3}$     | $0.656^{+0.056}_{-0.064}$        | $1.382^{+0.075}_{-0.072}$       | $2.66^{+0.06}_{-0.06} \times 10^{-10}$             | $9.90^{+0.33}_{-0.33} \times 10^{-11}$               | 292.9 / 286  |
| 33.376                    | $1.57^{+0.11}_{-0.13}$                          | $19.3^{+2.1}_{-1.2}$     | $0.243^{+0.040}_{-0.024}$        | $0.984^{+0.088}_{-0.082}$       | $3.16^{+0.32}_{-0.33} \times 10^{-11}$             | $8.90^{+0.34}_{-0.33} \times 10^{-11}$               | 278.5 / 277  |
| 33.429                    | $1.98^{+0.35}_{-0.31}$                          | $18.9^{+2.4}_{-3.2}$     | $0.675^{+0.120}_{-0.030}$        | —                               | $2.83^{+0.82}_{-0.76} \times 10^{-11}$             | $9.04^{+1.26}_{-1.14} \times 10^{-11}$               | 90.2 / 118   |
| 33.441                    | $1.41^{+0.13}_{-0.13}$                          | $15.9^{+3.3}_{-3.7}$     | $0.226^{+0.030}_{-0.025}$        | $1.192^{+0.093}_{-0.084}$       | $1.49^{+0.29}_{-0.28} \times 10^{-11}$             | $1.02^{+0.04}_{-0.04} \times 10^{-10}$               | 242.0 / 284  |
| 33.563                    | $0.87^{+0.12}_{-0.08}$                          | $16.6^{+1.3}_{-1.6}$     | $0.556^{+0.072}_{-0.095}$        | $2.699^{+2.732}_{-0.723}$       | $4.03^{+0.14}_{-0.14} \times 10^{-10}$             | $9.78^{+1.06}_{-0.85} \times 10^{-11}$               | 134.2 / 177  |
| 33.632                    | $0.84^{+0.05}_{-0.06}$                          | $18.7^{+0.9}_{-0.8}$     | $0.787^{+0.049}_{-0.059}$        | $2.424^{+1.587}_{-0.600}$       | $8.58^{+0.15}_{-0.15} \times 10^{-10}$             | $9.90^{+0.76}_{-0.69} \times 10^{-11}$               | 192.3 / 212  |
| 33.697                    | $0.78^{+0.02}_{-0.02}$                          | $25.0^{+0.3}_{-0.3}$     | $0.921^{+0.039}_{-0.051}$        | $1.708^{+0.283}_{-0.227}$       | $1.84^{+0.01}_{-0.01} \times 10^{-9}$              | $9.71^{+0.37}_{-0.37} \times 10^{-11}$               | 401.3 / 292  |
| 33.768                    | $0.65^{+0.02}_{-0.02}$                          | $29.9^{+0.4}_{-0.4}$     | $0.677^{+0.090}_{-0.088}$        | $1.281^{+0.105}_{-0.082}$       | $2.07^{+0.02}_{-0.02} \times 10^{-9}$              | $8.36^{+0.41}_{-0.40} \times 10^{-11}$               | 318.6 / 234  |
| 33.838                    | $0.67^{+0.01}_{-0.01}$                          | $31.8^{+0.3}_{-0.3}$     | $0.985^{+0.080}_{-0.158}$        | $1.558^{+0.292}_{-0.226}$       | $2.39^{+0.01}_{-0.01} \times 10^{-9}$              | $8.71^{+0.35}_{-0.34} \times 10^{-11}$               | 363.2 / 301  |
| 33.907                    | $0.79^{+0.02}_{-0.02}$                          | $20.4^{+0.5}_{-0.3}$     | $0.706^{+0.032}_{-0.033}$        | $1.576^{+0.146}_{-0.121}$       | $8.95^{+0.07}_{-0.07} \times 10^{-10}$             | $9.33^{+0.28}_{-0.28} \times 10^{-11}$               | 311.7 / 309  |
| 33.973                    | $0.80^{+0.04}_{-0.04}$                          | $18.0^{+0.8}_{-0.6}$     | $0.559^{+0.034}_{-0.036}$        | $1.492^{+0.104}_{-0.089}$       | $3.87^{+0.05}_{-0.05} \times 10^{-10}$             | $9.31^{+0.26}_{-0.26} \times 10^{-11}$               | 392.4 / 313  |
| 34.04                     | $0.82^{+0.02}_{-0.02}$                          | $20.6^{+0.3}_{-0.3}$     | $0.784^{+0.036}_{-0.089}$        | $1.414^{+0.203}_{-0.200}$       | $9.47^{+0.07}_{-0.07} \times 10^{-10}$             | $9.43^{+0.27}_{-0.25} \times 10^{-11}$               | 337.5 / 333  |
| 34.107                    | $0.86^{+0.01}_{-0.02}$                          | $22.1^{+0.2}_{-0.2}$     | $0.846^{+0.022}_{-0.022}$        | $2.010^{+0.455}_{-0.272}$       | $1.93^{+0.01}_{-0.01} \times 10^{-9}$              | $9.70^{+0.28}_{-0.27} \times 10^{-11}$               | 503.8 / 337  |
| 34.166                    | $0.71^{+0.01}_{-0.02}$                          | $26.4^{+0.3}_{-0.3}$     | $0.950^{+0.040}_{-0.046}$        | $1.805^{+0.462}_{-0.314}$       | $2.78^{+0.02}_{-0.02} \times 10^{-9}$              | $9.62^{+0.45}_{-0.44} \times 10^{-11}$               | 466.1 / 264  |
| 34.18                     | $0.80^{+0.01}_{-0.02}$                          | $28.4^{+0.3}_{-0.3}$     | —                                | $1.036^{+0.019}_{-0.036}$       | $3.05^{+0.02}_{-0.02} \times 10^{-9}$              | $8.67^{+0.29}_{-0.32} \times 10^{-11}$               | 283.5 / 269  |
| 34.707                    | $0.64^{+0.04}_{-0.03}$                          | $27.8^{+0.8}_{-0.7}$     | $0.932^{+0.064}_{-0.070}$        | —                               | $1.50^{+0.02}_{-0.02} \times 10^{-9}$              | $8.14^{+0.87}_{-0.78} \times 10^{-11}$               | 174.2 / 175  |
| 35.925                    | $0.74^{+0.05}_{-0.07}$                          | $22.2^{+1.5}_{-0.9}$     | $0.552^{+0.095}_{-0.107}$        | $1.221^{+0.135}_{-0.106}$       | $6.38^{+0.14}_{-0.14} \times 10^{-10}$             | $7.89^{+0.60}_{-0.59} \times 10^{-11}$               | 155.6 / 187  |
| 35.979                    | $0.72^{+0.03}_{-0.02}$                          | $24.0^{+0.5}_{-0.5}$     | $0.634^{+0.046}_{-0.042}$        | $1.333^{+0.088}_{-0.066}$       | $5.80^{+0.05}_{-0.05} \times 10^{-10}$             | $7.40^{+0.21}_{-0.22} \times 10^{-11}$               | 405.0 / 304  |
| 36.049                    | $0.75^{+0.03}_{-0.03}$                          | $20.2^{+0.6}_{-0.5}$     | $0.741^{+0.031}_{-0.040}$        | $1.611^{+0.202}_{-0.156}$       | $7.01^{+0.07}_{-0.07} \times 10^{-10}$             | $8.66^{+0.28}_{-0.27} \times 10^{-11}$               | 340.7 / 296  |
| 36.113                    | $0.89^{+0.02}_{-0.02}$                          | $22.6^{+0.3}_{-0.3}$     | $0.581^{+0.040}_{-0.042}$        | $1.166^{+0.043}_{-0.049}$       | $8.51^{+0.06}_{-0.06} \times 10^{-10}$             | $8.80^{+0.20}_{-0.21} \times 10^{-11}$               | 332.3 / 329  |
| Continued on next page    |                                                 |                          |                                  |                                 |                                                    |                                                      |              |

Table 1 – continued from previous page

| $T_{\text{mid}}$<br>(day) | $N_{\text{H}}$<br>( $10^{22} \text{ cm}^{-2}$ ) | $kT_{\text{BB}}$<br>(eV) | APEC $kT_{\text{cool}}$<br>(keV) | APEC $kT_{\text{hot}}$<br>(keV) | BB Flux<br>( $\text{erg cm}^{-2} \text{ s}^{-1}$ ) | APEC Flux<br>( $\text{erg cm}^{-2} \text{ s}^{-1}$ ) | Cstat/dof   |
|---------------------------|-------------------------------------------------|--------------------------|----------------------------------|---------------------------------|----------------------------------------------------|------------------------------------------------------|-------------|
| 36.168                    | $0.67^{+0.06}_{-0.02}$                          | $23.5^{+0.8}_{-1.1}$     | $0.660^{+0.116}_{-0.127}$        | $1.240^{+0.174}_{-0.121}$       | $6.68^{+0.12}_{-0.12} \times 10^{-10}$             | $8.07^{+0.46}_{-0.46} \times 10^{-11}$               | 210.8 / 205 |
| 36.185                    | $0.56^{+0.02}_{-0.02}$                          | $27.6^{+0.6}_{-0.6}$     | $0.671^{+0.046}_{-0.044}$        | $1.498^{+0.094}_{-0.078}$       | $6.16^{+0.06}_{-0.06} \times 10^{-10}$             | $8.91^{+0.28}_{-0.27} \times 10^{-11}$               | 287.3 / 303 |
| 36.247                    | $0.40^{+0.02}_{-0.02}$                          | $38.4^{+0.7}_{-0.7}$     | $0.541^{+0.038}_{-0.043}$        | $1.711^{+0.084}_{-0.074}$       | $4.96^{+0.05}_{-0.05} \times 10^{-10}$             | $9.78^{+0.29}_{-0.27} \times 10^{-11}$               | 461.7 / 346 |
| 36.314                    | $0.62^{+0.02}_{-0.02}$                          | $26.3^{+0.5}_{-0.5}$     | $0.748^{+0.027}_{-0.028}$        | $1.598^{+0.101}_{-0.100}$       | $5.43^{+0.05}_{-0.05} \times 10^{-10}$             | $8.29^{+0.22}_{-0.22} \times 10^{-11}$               | 421.1 / 319 |
| 36.367                    | $0.95^{+0.06}_{-0.02}$                          | $20.1^{+1.0}_{-1.0}$     | $0.741^{+0.082}_{-0.072}$        | —                               | $9.22^{+0.28}_{-0.28} \times 10^{-10}$             | $6.32^{+0.80}_{-0.81} \times 10^{-11}$               | 120.1 / 118 |
| 36.387                    | $0.63^{+0.02}_{-0.02}$                          | $24.4^{+0.5}_{-0.4}$     | $0.775^{+0.038}_{-0.050}$        | $1.651^{+0.188}_{-0.156}$       | $8.48^{+0.07}_{-0.07} \times 10^{-10}$             | $7.03^{+0.28}_{-0.27} \times 10^{-11}$               | 317.3 / 271 |
| 36.436                    | $0.80^{+0.04}_{-0.07}$                          | $19.8^{+1.1}_{-0.7}$     | $0.563^{+0.098}_{-0.101}$        | $1.060^{+0.117}_{-0.097}$       | $7.45^{+0.13}_{-0.13} \times 10^{-10}$             | $7.89^{+0.45}_{-0.43} \times 10^{-11}$               | 185.6 / 202 |
| 36.46                     | $0.93^{+0.06}_{-0.08}$                          | $19.5^{+1.3}_{-1.0}$     | $0.730^{+0.098}_{-0.107}$        | $1.143^{+1.604}_{-0.580}$       | $5.90^{+0.16}_{-0.16} \times 10^{-10}$             | $7.09^{+0.84}_{-0.77} \times 10^{-11}$               | 160.1 / 169 |
| 36.506                    | $0.87^{+0.04}_{-0.04}$                          | $17.8^{+1.3}_{-1.4}$     | $0.681^{+0.073}_{-0.076}$        | $1.553^{+0.454}_{-0.245}$       | $5.55^{+0.13}_{-0.13} \times 10^{-10}$             | $7.46^{+0.58}_{-0.55} \times 10^{-11}$               | 205.1 / 184 |
| 36.785                    | $0.74^{+0.05}_{-0.06}$                          | $19.7^{+1.2}_{-1.3}$     | $0.616^{+0.063}_{-0.060}$        | $1.226^{+0.142}_{-0.109}$       | $4.52^{+0.09}_{-0.09} \times 10^{-10}$             | $7.33^{+0.38}_{-0.37} \times 10^{-11}$               | 236.7 / 217 |
| 36.851                    | $0.51^{+0.03}_{-0.05}$                          | $26.7^{+1.4}_{-0.9}$     | $0.560^{+0.156}_{-0.103}$        | $1.310^{+0.117}_{-0.104}$       | $5.05^{+0.10}_{-0.10} \times 10^{-10}$             | $8.20^{+0.52}_{-0.42} \times 10^{-11}$               | 264.1 / 210 |
| 36.917                    | $0.36^{+0.02}_{-0.02}$                          | $41.7^{+0.9}_{-1.0}$     | $0.482^{+0.099}_{-0.099}$        | $1.600^{+0.126}_{-0.116}$       | $8.74^{+0.13}_{-0.13} \times 10^{-10}$             | $7.69^{+0.53}_{-0.61} \times 10^{-11}$               | 242.9 / 212 |
| 36.985                    | $0.38^{+0.03}_{-0.03}$                          | $43.2^{+1.3}_{-1.4}$     | $0.432^{+0.065}_{-0.059}$        | $1.526^{+0.256}_{-0.183}$       | $8.04^{+0.11}_{-0.14} \times 10^{-10}$             | $8.86^{+0.99}_{-0.72} \times 10^{-11}$               | 254.5 / 222 |
| 37.051                    | $0.33^{+0.03}_{-0.02}$                          | $45.0^{+1.0}_{-1.1}$     | $0.529^{+0.495}_{-0.313}$        | $1.607^{+0.106}_{-0.105}$       | $1.09^{+0.01}_{-0.02} \times 10^{-9}$              | $7.04^{+0.75}_{-0.72} \times 10^{-11}$               | 263.7 / 220 |
| 37.123                    | $0.53^{+0.01}_{-0.01}$                          | $37.9^{+0.4}_{-0.2}$     | $0.436^{+0.041}_{-0.026}$        | $1.454^{+0.081}_{-0.066}$       | $1.65^{+0.01}_{-0.01} \times 10^{-9}$              | $7.39^{+0.16}_{-0.25} \times 10^{-11}$               | 466.7 / 275 |
| 37.259                    | $0.64^{+0.02}_{-0.02}$                          | $33.7^{+0.4}_{-0.4}$     | $0.721^{+0.081}_{-0.073}$        | $1.386^{+0.110}_{-0.086}$       | $2.04^{+0.01}_{-0.01} \times 10^{-9}$              | $7.70^{+0.36}_{-0.34} \times 10^{-11}$               | 293.9 / 258 |
| 37.395                    | $0.66^{+0.02}_{-0.03}$                          | $30.3^{+0.6}_{-0.5}$     | $0.829^{+0.092}_{-0.162}$        | $1.758^{+0.324}_{-0.256}$       | $1.55^{+0.01}_{-0.01} \times 10^{-9}$              | $7.54^{+0.48}_{-0.46} \times 10^{-11}$               | 281.7 / 241 |
| 37.442                    | $0.71^{+0.03}_{-0.03}$                          | $27.8^{+0.7}_{-0.7}$     | $0.901^{+0.075}_{-0.117}$        | $2.041^{+3.688}_{-0.776}$       | $1.59^{+0.02}_{-0.02} \times 10^{-9}$              | $7.55^{+0.79}_{-0.77} \times 10^{-11}$               | 177.9 / 186 |
| 37.465                    | $0.79^{+0.05}_{-0.03}$                          | $23.0^{+0.6}_{-0.9}$     | $0.698^{+0.169}_{-0.187}$        | —                               | $1.29^{+0.02}_{-0.02} \times 10^{-9}$              | $7.22^{+0.52}_{-0.51} \times 10^{-11}$               | 153.0 / 178 |
| 37.794                    | $0.64^{+0.01}_{-0.01}$                          | $35.2^{+0.1}_{-0.5}$     | —                                | $1.209^{+0.057}_{-0.121}$       | $3.52^{+0.03}_{-0.03} \times 10^{-9}$              | $7.43^{+0.44}_{-0.47} \times 10^{-11}$               | 250.5 / 196 |
| 38.123                    | $0.86^{+0.01}_{-0.01}$                          | $27.5^{+0.2}_{-0.2}$     | $0.653^{+0.111}_{-0.101}$        | $1.021^{+0.043}_{-0.036}$       | $2.93^{+0.01}_{-0.01} \times 10^{-9}$              | $7.40^{+0.18}_{-0.19} \times 10^{-11}$               | 529.0 / 297 |
| 38.18                     | $0.71^{+0.02}_{-0.02}$                          | $23.8^{+0.4}_{-0.4}$     | $0.803^{+0.049}_{-0.044}$        | $2.611^{+3.925}_{-0.793}$       | $2.00^{+0.02}_{-0.02} \times 10^{-9}$              | $6.94^{+0.44}_{-0.40} \times 10^{-11}$               | 273.6 / 216 |
| 38.262                    | $0.83^{+0.02}_{-0.03}$                          | $22.4^{+0.6}_{-0.2}$     | $0.539^{+0.692}_{-0.316}$        | $0.909^{+7.658}_{-0.031}$       | $1.65^{+0.01}_{-0.02} \times 10^{-9}$              | $7.26^{+0.37}_{-0.36} \times 10^{-11}$               | 220.1 / 211 |
| 38.329                    | $0.90^{+0.02}_{-0.01}$                          | $22.8^{+0.4}_{-0.4}$     | $0.875^{+0.033}_{-0.036}$        | —                               | $2.24^{+0.02}_{-0.02} \times 10^{-9}$              | $7.69^{+0.52}_{-0.49} \times 10^{-11}$               | 322.5 / 218 |
| 38.399                    | $1.08^{+0.03}_{-0.03}$                          | $25.3^{+0.4}_{-0.4}$     | $0.456^{+0.191}_{-0.178}$        | $0.963^{+0.109}_{-0.071}$       | $2.63^{+0.02}_{-0.02} \times 10^{-9}$              | $6.91^{+0.36}_{-0.35} \times 10^{-11}$               | 248.9 / 214 |
| 38.446                    | $0.50^{+0.02}_{-0.03}$                          | $35.2^{+0.7}_{-0.3}$     | $0.140^{+0.567}_{-0.140}$        | $1.447^{+0.167}_{-0.154}$       | $2.43^{+0.03}_{-0.03} \times 10^{-9}$              | $5.83^{+1.11}_{-0.67} \times 10^{-11}$               | 151.3 / 142 |
| 38.514                    | $0.27^{+0.03}_{-0.02}$                          | $50.2^{+1.1}_{-1.2}$     | —                                | $1.650^{+2.412}_{-0.176}$       | $9.02^{+0.16}_{-0.16} \times 10^{-10}$             | $6.31^{+0.59}_{-0.54} \times 10^{-11}$               | 194.1 / 188 |
| 38.582                    | $0.34^{+0.15}_{-0.16}$                          | $38.0^{+8.4}_{-5.6}$     | $0.757^{+0.088}_{-0.092}$        | $1.648^{+0.460}_{-0.300}$       | $1.16^{+0.10}_{-0.08} \times 10^{-10}$             | $6.77^{+0.52}_{-0.49} \times 10^{-11}$               | 232.1 / 205 |
| 38.648                    | $0.20^{+0.09}_{-0.07}$                          | $46.7^{+4.8}_{-4.8}$     | $0.850^{+0.074}_{-0.092}$        | $1.718^{+0.247}_{-0.211}$       | $1.46^{+0.08}_{-0.09} \times 10^{-10}$             | $7.09^{+0.50}_{-0.51} \times 10^{-11}$               | 195.6 / 201 |
| 38.716                    | $0.43^{+0.03}_{-0.03}$                          | $33.9^{+1.2}_{-1.0}$     | $0.511^{+0.084}_{-0.080}$        | $1.762^{+0.228}_{-0.172}$       | $7.08^{+0.13}_{-0.12} \times 10^{-10}$             | $7.65^{+0.52}_{-0.53} \times 10^{-11}$               | 192.1 / 206 |
| 38.998                    | $0.28^{+0.02}_{-0.02}$                          | $45.9^{+1.0}_{-1.3}$     | $0.906^{+0.288}_{-0.375}$        | $1.395^{+0.191}_{-0.102}$       | $8.60^{+0.13}_{-0.13} \times 10^{-10}$             | $5.80^{+0.46}_{-0.42} \times 10^{-11}$               | 226.9 / 197 |
| 39.065                    | $0.16^{+0.06}_{-0.03}$                          | $53.7^{+1.7}_{-4.3}$     | $0.455^{+0.110}_{-0.099}$        | $1.511^{+0.117}_{-0.096}$       | $2.49^{+0.10}_{-0.10} \times 10^{-10}$             | $7.82^{+0.77}_{-0.73} \times 10^{-11}$               | 215.0 / 201 |
| 39.132                    | $0.21^{+0.07}_{-0.06}$                          | $54.8^{+5.2}_{-4.3}$     | $0.314^{+0.089}_{-0.070}$        | $1.610^{+0.189}_{-0.139}$       | $1.74^{+0.10}_{-0.13} \times 10^{-10}$             | $8.97^{+1.28}_{-0.97} \times 10^{-11}$               | 209.9 / 202 |
| 39.188                    | $0.09^{+0.06}_{-0.03}$                          | $61.3^{+1.1}_{-8.1}$     | $0.150^{+0.559}_{-0.150}$        | —                               | $6.52^{+0.58}_{-0.80} \times 10^{-10}$             | $7.90^{+5.59}_{-5.10} \times 10^{-11}$               | 72.6 / 54   |
| 39.194                    | $0.20^{+0.02}_{-0.01}$                          | $54.7^{+0.9}_{-1.4}$     | $0.433^{+0.033}_{-0.038}$        | $1.107^{+0.131}_{-0.113}$       | $8.56^{+0.10}_{-0.12} \times 10^{-10}$             | $9.19^{+0.41}_{-0.91} \times 10^{-11}$               | 405.6 / 233 |
| 39.261                    | $0.23^{+0.02}_{-0.01}$                          | $54.1^{+1.0}_{-1.1}$     | $0.435^{+0.057}_{-0.039}$        | $1.619^{+0.120}_{-0.100}$       | $9.56^{+0.10}_{-0.22} \times 10^{-10}$             | $8.19^{+0.51}_{-0.60} \times 10^{-11}$               | 370.3 / 229 |
| 39.473                    | $0.40^{+0.04}_{-0.04}$                          | $46.0^{+1.0}_{-2.3}$     | —                                | $1.403^{+2.268}_{-0.647}$       | $7.71^{+0.19}_{-0.19} \times 10^{-10}$             | $6.49^{+0.60}_{-0.78} \times 10^{-11}$               | 185.5 / 156 |
| 39.255                    | $0.35^{+0.13}_{-0.12}$                          | $46.7^{+4.1}_{-4.3}$     | $0.408^{+0.604}_{-0.196}$        | —                               | $6.54^{+0.55}_{-0.60} \times 10^{-10}$             | $1.46^{+0.90}_{-0.71} \times 10^{-10}$               | 52.3 / 67   |
| 39.401                    | $0.14^{+0.03}_{-0.01}$                          | $62.4^{+0.2}_{-5.0}$     | —                                | $2.642^{+1.473}_{-0.616}$       | $7.39^{+0.24}_{-0.41} \times 10^{-10}$             | $5.97^{+1.73}_{-1.61} \times 10^{-11}$               | 149.7 / 110 |
| 39.515                    | $0.38^{+0.05}_{-0.09}$                          | $49.2^{+3.2}_{-2.6}$     | —                                | $1.331^{+0.787}_{-0.412}$       | $1.90^{+0.09}_{-0.09} \times 10^{-9}$              | $5.01^{+3.24}_{-2.38} \times 10^{-11}$               | 84.3 / 65   |
| 39.652                    | $0.20^{+0.01}_{-0.02}$                          | $54.1^{+1.1}_{-0.9}$     | —                                | $1.713^{+0.176}_{-0.111}$       | $1.19^{+0.02}_{-0.02} \times 10^{-9}$              | $5.90^{+0.85}_{-0.55} \times 10^{-11}$               | 244.8 / 164 |
| 39.786                    | $0.22^{+0.01}_{-0.01}$                          | $51.9^{+0.9}_{-0.3}$     | —                                | $1.527^{+0.075}_{-0.105}$       | $1.55^{+0.02}_{-0.02} \times 10^{-9}$              | $5.75^{+0.67}_{-0.40} \times 10^{-11}$               | 315.7 / 175 |
| 39.853                    | $0.25^{+0.01}_{-0.01}$                          | $51.5^{+0.8}_{-0.1}$     | —                                | $1.537^{+0.137}_{-0.107}$       | $1.50^{+0.02}_{-0.02} \times 10^{-9}$              | $6.18^{+0.62}_{-1.02} \times 10^{-11}$               | 294.2 / 182 |
| 40.121                    | $0.34^{+0.01}_{-0.01}$                          | $48.3^{+0.1}_{-0.1}$     | $0.426^{+0.374}_{-0.278}$        | $1.613^{+0.158}_{-0.147}$       | $1.71^{+0.02}_{-0.02} \times 10^{-9}$              | $5.13^{+0.82}_{-0.52} \times 10^{-11}$               | 241.7 / 185 |
| 40.19                     | $0.23^{+0.02}_{-0.01}$                          | $55.7^{+0.8}_{-1.1}$     | $0.441^{+0.054}_{-0.046}$        | $1.815^{+0.139}_{-0.125}$       | $9.62^{+0.08}_{-0.13} \times 10^{-10}$             | $6.37^{+0.54}_{-0.30} \times 10^{-11}$               | 441.3 / 246 |
| 40.258                    | $0.31^{+0.01}_{-0.01}$                          | $52.7^{+0.7}_{-0.1}$     | —                                | $1.516^{+0.070}_{-0.076}$       | $1.08^{+0.01}_{-0.01} \times 10^{-9}$              | $5.75^{+0.42}_{-0.26} \times 10^{-11}$               | 479.2 / 229 |
| 40.728                    | $0.20^{+0.02}_{-0.02}$                          | $58.0^{+1.3}_{-1.1}$     | $0.433^{+0.041}_{-0.029}$        | $1.796^{+0.105}_{-0.114}$       | $3.97^{+0.07}_{-0.10} \times 10^{-9}$              | $7.90^{+0.47}_{-0.40} \times 10^{-11}$               | 452.2 / 255 |
| 42.796                    | $0.49^{+0.06}_{-0.03}$                          | $44.2^{+0.8}_{-1.1}$     | —                                | $1.427^{+1.721}_{-0.579}$       | $2.51^{+0.07}_{-0.07} \times 10^{-9}$              | $5.11^{+1.48}_{-1.27} \times 10^{-11}$               | 109.3 / 89  |
| 42.997                    | $0.59^{+0.02}_{-0.05}$                          | $41.9^{+0.9}_{-2.2}$     | $0.435^{+0.663}_{-0.290}$        | —                               | $3.14^{+0.06}_{-0.06} \times 10^{-9}$              | $4.43^{+1.89}_{-1.70} \times 10^{-11}$               | 99.3 / 94   |
| 43.064                    | $0.50^{+0.05}_{-0.07}$                          | $41.0^{+2.2}_{-1.3}$     | —                                | $1.388^{+0.305}_{-0.190}$       | $2.44^{+0.08}_{-0.08} \times 10^{-9}$              | $5.10^{+1.40}_{-1.49} \times 10^{-11}$               | 99.9 / 81   |
| 43.14                     | $0.37^{+0.02}_{-0.02}$                          | $40.9^{+0.7}_{-1.0}$     | —                                | $1.258^{+0.149}_{-0.129}$       | $1.53^{+0.02}_{-0.02} \times 10^{-9}$              | $5.05^{+0.46}_{-0.43} \times 10^{-11}$               | 206.8 / 178 |
| 43.204                    | $0.68^{+0.04}_{-0.12}$                          | $38.6^{+4.0}_{-1.3}$     | $0.870^{+0.529}_{-0.870}$        | —                               | $2.74^{+0.11}_{-0.11} \times 10^{-9}$              | $1.40^{+1.30}_{-0.52} \times 10^{-10}$               | 37.0 / 65   |
| 43.603                    | $0.53^{+0.03}_{-0.02}$                          | $35.8^{+0.8}_{-0.7}$     | —                                | $1.097^{+0.101}_{-0.102}$       | $1.27^{+0.02}_{-0.01} \times 10^{-9}$              | $5.51^{+0.38}_{-0.37} \times 10^{-11}$               | 211.2 / 207 |
| 43.67                     | $0.57^{+0.01}_{-0.03}$                          | $36.4^{+1.0}_{-0.3}$     | —                                | $1.238^{+0.087}_{-0.059}$       | $2.24^{+0.02}_{-0.02} \times 10^{-9}$              | $5.52^{+0.36}_{-0.36} \times 10^{-11}$               | 221.5 / 200 |
| 43.807                    | $0.54^{+0.01}_{-0.01}$                          | $40.8^{+0.4}_{-0.4}$     | $0.460^{+0.054}_{-0.056}$        | $1.433^{+0.076}_{-0.078}$       | $1.78^{+0.01}_{-0.02} \times 10^{-9}$              | $5.62^{+0.35}_{-0.32} \times 10^{-11}$               | 362.1 / 231 |
| 43.874                    | $0.46^{+0.01}_{-0.02}$                          | $44.6^{+0.5}_{-0.5}$     | $0.466^{+0.042}_{-0.131}$        | $1.512^{+0.087}_{-0.080}$       | $1.76^{+0.02}_{-0.01} \times 10^{-9}$              | $6.05^{+0.39}_{-0.39} \times 10^{-11}$               | 487.4 / 234 |
| 43.941                    | $0.54^{+0.01}_{-0.01}$                          | $39.6^{+0.3}_{-0.1}$     | $0.457^{+0.131}_{-0.106}$        | $1.286^{+0.080}_{-0.052}$       | $2.33^{+0.01}_{-0.02} \times 10^{-9}$              | $4.82^{+0.32}_{-0.27} \times 10^{-11}$               | 404.4 / 227 |

Continued on next page

Table 1 – continued from previous page

| $T_{\text{mid}}$<br>(day) | $N_{\text{H}}$<br>( $10^{22} \text{ cm}^{-2}$ ) | $kT_{\text{BB}}$<br>(eV) | APEC $kT_{\text{cool}}$<br>(keV) | APEC $kT_{\text{hot}}$<br>(keV) | BB Flux<br>( $\text{erg cm}^{-2} \text{ s}^{-1}$ ) | APEC Flux<br>( $\text{erg cm}^{-2} \text{ s}^{-1}$ ) | Cstat/dof    |
|---------------------------|-------------------------------------------------|--------------------------|----------------------------------|---------------------------------|----------------------------------------------------|------------------------------------------------------|--------------|
| 44.008                    | $0.37^{+0.01}_{-0.01}$                          | $47.7^{+0.5}_{-0.3}$     | —                                | $1.453^{+0.069}_{-0.061}$       | $1.42^{+0.01}_{-0.01} \times 10^{-9}$              | $4.96^{+0.19}_{-0.35} \times 10^{-11}$               | 575.4 / 234  |
| 44.142                    | $0.57^{+0.01}_{-0.01}$                          | $41.4^{+0.1}_{-0.1}$     | —                                | $1.450^{+0.046}_{-0.045}$       | $2.77^{+0.02}_{-0.02} \times 10^{-9}$              | $4.97^{+0.27}_{-0.24} \times 10^{-11}$               | 586.4 / 235  |
| 44.209                    | $0.54^{+0.01}_{-0.01}$                          | $42.6^{+0.1}_{-0.2}$     | —                                | $1.366^{+0.060}_{-0.069}$       | $2.83^{+0.02}_{-0.02} \times 10^{-9}$              | $4.15^{+0.34}_{-0.31} \times 10^{-11}$               | 442.1 / 190  |
| 44.813                    | $0.66^{+0.01}_{-0.02}$                          | $34.9^{+0.5}_{-0.3}$     | —                                | $1.241^{+0.060}_{-0.048}$       | $3.36^{+0.02}_{-0.02} \times 10^{-9}$              | $4.85^{+0.36}_{-0.28} \times 10^{-11}$               | 315.3 / 207  |
| 44.944                    | $0.53^{+0.01}_{-0.01}$                          | $33.4^{+0.3}_{-0.4}$     | —                                | $1.019^{+0.055}_{-0.045}$       | $2.85^{+0.02}_{-0.02} \times 10^{-9}$              | $3.76^{+0.29}_{-0.23} \times 10^{-11}$               | 343.9 / 181  |
| 45.012                    | $0.67^{+0.01}_{-0.02}$                          | $38.5^{+0.3}_{-0.2}$     | —                                | $1.373^{+0.097}_{-0.085}$       | $2.82^{+0.02}_{-0.02} \times 10^{-9}$              | $3.95^{+0.39}_{-0.31} \times 10^{-11}$               | 443.3 / 198  |
| 45.079                    | $0.62^{+0.01}_{-0.01}$                          | $40.0^{+0.2}_{-0.2}$     | —                                | $1.455^{+0.277}_{-0.567}$       | $3.97^{+0.02}_{-0.02} \times 10^{-9}$              | $4.10^{+0.42}_{-0.29} \times 10^{-11}$               | 789.4 / 194  |
| 45.214                    | $0.74^{+0.02}_{-0.01}$                          | $38.3^{+0.4}_{-0.3}$     | $0.457^{+0.830}_{-0.457}$        | $1.247^{+0.150}_{-0.124}$       | $4.29^{+0.04}_{-0.04} \times 10^{-9}$              | $4.04^{+0.55}_{-0.43} \times 10^{-11}$               | 286.6 / 141  |
| 46.149                    | $0.63^{+0.01}_{-0.01}$                          | $40.5^{+0.2}_{-0.1}$     | —                                | $1.369^{+0.076}_{-0.047}$       | $3.67^{+0.03}_{-0.03} \times 10^{-9}$              | $3.97^{+0.45}_{-0.19} \times 10^{-11}$               | 596.2 / 206  |
| 45.676                    | $0.70^{+0.01}_{-0.01}$                          | $37.9^{+0.4}_{-0.3}$     | $0.457^{+0.095}_{-0.112}$        | $1.385^{+0.437}_{-0.188}$       | $3.91^{+0.04}_{-0.05} \times 10^{-9}$              | $4.06^{+0.81}_{-0.55} \times 10^{-11}$               | 172.3 / 126  |
| 45.815                    | $0.66^{+0.01}_{-0.01}$                          | $39.7^{+0.2}_{-0.3}$     | —                                | $1.371^{+0.044}_{-0.047}$       | $3.84^{+0.02}_{-0.02} \times 10^{-9}$              | $5.14^{+0.18}_{-0.49} \times 10^{-11}$               | 222.8 / 141  |
| 46.015                    | $0.76^{+0.01}_{-0.01}$                          | $37.2^{+0.2}_{-0.2}$     | $0.458^{+0.040}_{-0.030}$        | $1.314^{+0.083}_{-0.062}$       | $3.75^{+0.02}_{-0.02} \times 10^{-9}$              | $4.24^{+0.36}_{-0.23} \times 10^{-11}$               | 664.7 / 221  |
| 46.082                    | $0.71^{+0.01}_{-0.01}$                          | $39.1^{+0.2}_{-0.2}$     | —                                | $1.380^{+0.105}_{-0.039}$       | $3.81^{+0.02}_{-0.02} \times 10^{-9}$              | $4.44^{+0.27}_{-0.29} \times 10^{-11}$               | 612.4 / 214  |
| 46.55                     | $0.76^{+0.01}_{-0.01}$                          | $38.1^{+0.3}_{-0.3}$     | $0.461^{+0.069}_{-0.144}$        | $1.292^{+0.087}_{-0.071}$       | $4.10^{+0.02}_{-0.03} \times 10^{-9}$              | $4.17^{+0.45}_{-0.28} \times 10^{-11}$               | 510.6 / 181  |
| 47.087                    | $0.74^{+0.01}_{-0.01}$                          | $38.9^{+0.3}_{-0.3}$     | $0.478^{+0.031}_{-0.042}$        | $1.366^{+0.080}_{-0.066}$       | $4.18^{+0.02}_{-0.02} \times 10^{-9}$              | $4.95^{+0.27}_{-0.29} \times 10^{-11}$               | 923.2 / 210  |
| 47.154                    | $0.71^{+0.01}_{-0.01}$                          | $39.7^{+0.2}_{-0.3}$     | $0.458^{+0.050}_{-0.032}$        | $1.447^{+0.098}_{-0.083}$       | $4.25^{+0.02}_{-0.02} \times 10^{-9}$              | $4.48^{+0.30}_{-0.28} \times 10^{-11}$               | 705.5 / 203  |
| 47.555                    | $0.69^{+0.01}_{-0.01}$                          | $39.1^{+0.3}_{-0.2}$     | —                                | $1.370^{+0.125}_{-0.091}$       | $4.48^{+0.03}_{-0.04} \times 10^{-9}$              | $3.63^{+0.49}_{-0.39} \times 10^{-11}$               | 372.5 / 156  |
| 47.756                    | $0.71^{+0.01}_{-0.01}$                          | $38.4^{+0.1}_{-0.2}$     | $0.482^{+0.054}_{-0.071}$        | $1.331^{+0.076}_{-0.063}$       | $3.74^{+0.02}_{-0.02} \times 10^{-9}$              | $3.83^{+0.26}_{-0.26} \times 10^{-11}$               | 581.7 / 195  |
| 47.957                    | $0.64^{+0.01}_{-0.01}$                          | $40.5^{+0.2}_{-0.1}$     | $0.455^{+0.035}_{-0.044}$        | $1.366^{+0.121}_{-0.049}$       | $4.48^{+0.02}_{-0.03} \times 10^{-9}$              | $4.35^{+0.27}_{-0.46} \times 10^{-11}$               | 941.0 / 199  |
| 48.161                    | $0.68^{+0.02}_{-0.01}$                          | $39.7^{+0.4}_{-0.3}$     | $0.450^{+0.046}_{-0.055}$        | $1.366^{+0.174}_{-0.104}$       | $3.86^{+0.03}_{-0.03} \times 10^{-9}$              | $4.17^{+0.40}_{-0.36} \times 10^{-11}$               | 331.9 / 169  |
| 48.233                    | $0.66^{+0.01}_{-0.01}$                          | $39.1^{+0.3}_{-0.1}$     | —                                | $1.247^{+0.071}_{-0.060}$       | $3.72^{+0.02}_{-0.02} \times 10^{-9}$              | $3.90^{+0.29}_{-0.29} \times 10^{-11}$               | 489.4 / 181  |
| 48.024                    | $0.68^{+0.01}_{-0.01}$                          | $39.5^{+0.3}_{-0.2}$     | $0.471^{+0.842}_{-0.471}$        | $1.304^{+0.076}_{-0.044}$       | $4.47^{+0.02}_{-0.03} \times 10^{-9}$              | $4.43^{+0.32}_{-0.30} \times 10^{-11}$               | 722.0 / 201  |
| 48.558                    | $0.68^{+0.01}_{-0.01}$                          | $38.4^{+0.3}_{-0.3}$     | $0.455^{+0.063}_{-0.182}$        | $1.289^{+0.084}_{-0.073}$       | $3.72^{+0.02}_{-0.02} \times 10^{-9}$              | $3.70^{+0.23}_{-0.38} \times 10^{-11}$               | 510.6 / 185  |
| 48.693                    | $0.62^{+0.01}_{-0.01}$                          | $39.9^{+0.2}_{-0.1}$     | $1.322^{+0.074}_{-0.054}$        | —                               | $3.87^{+0.02}_{-0.02} \times 10^{-9}$              | $3.39^{+0.24}_{-0.27} \times 10^{-11}$               | 848.3 / 190  |
| 49.028                    | $0.61^{+0.01}_{-0.01}$                          | $41.0^{+0.2}_{-0.1}$     | $0.437^{+0.513}_{-0.298}$        | $1.307^{+0.078}_{-0.037}$       | $3.98^{+0.02}_{-0.02} \times 10^{-9}$              | $4.69^{+0.28}_{-0.28} \times 10^{-11}$               | 764.1 / 209  |
| 49.168                    | $0.62^{+0.01}_{-0.01}$                          | $40.6^{+0.1}_{-0.1}$     | $0.457^{+0.042}_{-0.053}$        | $1.294^{+0.133}_{-0.058}$       | $3.58^{+0.02}_{-0.03} \times 10^{-9}$              | $3.36^{+0.21}_{-0.27} \times 10^{-11}$               | 606.7 / 197  |
| 49.494                    | $0.69^{+0.01}_{-0.02}$                          | $39.8^{+0.4}_{-0.2}$     | $0.458^{+0.068}_{-0.059}$        | $1.362^{+0.143}_{-0.111}$       | $4.61^{+0.03}_{-0.04} \times 10^{-9}$              | $4.29^{+0.54}_{-0.55} \times 10^{-11}$               | 403.0 / 158  |
| 49.827                    | $0.72^{+0.05}_{-0.02}$                          | $39.6^{+0.8}_{-0.8}$     | $0.469^{+0.997}_{-0.469}$        | —                               | $4.51^{+0.11}_{-0.11} \times 10^{-9}$              | $4.62^{+0.20}_{-1.55} \times 10^{-11}$               | 85.8 / 80    |
| 49.893                    | $0.77^{+0.04}_{-0.03}$                          | $38.2^{+0.3}_{-0.2}$     | —                                | $1.294^{+0.525}_{-0.353}$       | $4.41^{+0.08}_{-0.09} \times 10^{-9}$              | $4.07^{+0.96}_{-1.09} \times 10^{-11}$               | 109.2 / 84   |
| 50.169                    | $0.67^{+0.01}_{-0.02}$                          | $39.8^{+0.3}_{-0.4}$     | $0.433^{+0.090}_{-0.285}$        | $1.284^{+0.168}_{-0.115}$       | $5.08^{+0.04}_{-0.03} \times 10^{-9}$              | $3.69^{+0.47}_{-0.56} \times 10^{-11}$               | 385.7 / 135  |
| 50.499                    | $0.59^{+0.01}_{-0.01}$                          | $41.6^{+0.2}_{-0.2}$     | —                                | $1.404^{+0.134}_{-0.107}$       | $4.27^{+0.03}_{-0.03} \times 10^{-9}$              | $2.70^{+0.49}_{-0.29} \times 10^{-11}$               | 448.7 / 168  |
| 50.637                    | $0.68^{+0.01}_{-0.01}$                          | $39.6^{+0.1}_{-0.1}$     | $0.461^{+0.147}_{-0.048}$        | $1.361^{+0.059}_{-0.074}$       | $4.00^{+0.02}_{-0.02} \times 10^{-9}$              | $3.99^{+0.24}_{-0.23} \times 10^{-11}$               | 735.0 / 207  |
| 50.769                    | $0.66^{+0.01}_{-0.01}$                          | $40.5^{+0.3}_{-0.3}$     | $0.460^{+0.036}_{-0.032}$        | $1.367^{+0.175}_{-0.076}$       | $4.18^{+0.02}_{-0.03} \times 10^{-9}$              | $3.73^{+0.36}_{-0.24} \times 10^{-11}$               | 591.6 / 187  |
| 50.836                    | $0.75^{+0.01}_{-0.01}$                          | $39.1^{+0.4}_{-0.3}$     | $0.461^{+0.047}_{-0.033}$        | $1.366^{+0.172}_{-0.072}$       | $4.22^{+0.02}_{-0.03} \times 10^{-9}$              | $4.48^{+0.25}_{-0.48} \times 10^{-11}$               | 546.2 / 181  |
| 50.903                    | $0.68^{+0.01}_{-0.01}$                          | $39.9^{+0.1}_{-0.2}$     | $0.458^{+0.092}_{-0.308}$        | $1.356^{+0.081}_{-0.080}$       | $4.65^{+0.02}_{-0.03} \times 10^{-9}$              | $3.22^{+0.28}_{-0.24} \times 10^{-11}$               | 791.7 / 187  |
| 50.97                     | $0.74^{+0.01}_{-0.01}$                          | $39.2^{+0.4}_{-0.3}$     | $0.458^{+0.041}_{-0.036}$        | $1.380^{+0.254}_{-0.103}$       | $4.14^{+0.02}_{-0.02} \times 10^{-9}$              | $3.54^{+0.24}_{-0.51} \times 10^{-11}$               | 519.7 / 183  |
| 51.037                    | $0.79^{+0.01}_{-0.01}$                          | $38.5^{+0.2}_{-0.2}$     | $0.459^{+0.037}_{-0.035}$        | $1.425^{+0.185}_{-0.129}$       | $4.56^{+0.02}_{-0.03} \times 10^{-9}$              | $3.33^{+0.21}_{-0.21} \times 10^{-11}$               | 661.7 / 180  |
| 51.572                    | $0.77^{+0.01}_{-0.01}$                          | $39.2^{+0.3}_{-0.5}$     | $0.457^{+0.036}_{-0.043}$        | $1.358^{+0.128}_{-0.111}$       | $4.94^{+0.03}_{-0.03} \times 10^{-9}$              | $4.87^{+0.34}_{-0.61} \times 10^{-11}$               | 534.5 / 183  |
| 51.638                    | $0.57^{+0.01}_{-0.02}$                          | $42.5^{+0.5}_{-0.2}$     | —                                | $1.456^{+0.101}_{-0.092}$       | $5.16^{+0.03}_{-0.03} \times 10^{-9}$              | $4.00^{+0.41}_{-0.44} \times 10^{-11}$               | 641.7 / 177  |
| 51.772                    | $0.69^{+0.01}_{-0.01}$                          | $40.1^{+0.4}_{-0.3}$     | $0.482^{+0.035}_{-0.045}$        | $1.493^{+0.371}_{-0.205}$       | $4.61^{+0.03}_{-0.03} \times 10^{-9}$              | $4.53^{+0.43}_{-0.35} \times 10^{-11}$               | 459.1 / 179  |
| 51.84                     | $0.71^{+0.01}_{-0.02}$                          | $40.2^{+0.4}_{-0.3}$     | $0.484^{+0.045}_{-0.058}$        | $1.380^{+0.222}_{-0.124}$       | $4.94^{+0.03}_{-0.04} \times 10^{-9}$              | $3.09^{+0.56}_{-0.26} \times 10^{-11}$               | 427.9 / 172  |
| 51.906                    | $0.70^{+0.01}_{-0.01}$                          | $39.9^{+0.2}_{-0.3}$     | $0.461^{+0.043}_{-0.038}$        | $1.362^{+0.154}_{-0.117}$       | $4.86^{+0.03}_{-0.03} \times 10^{-9}$              | $4.42^{+0.29}_{-0.45} \times 10^{-11}$               | 583.7 / 184  |
| 52.041                    | $0.68^{+0.01}_{-0.01}$                          | $39.3^{+0.3}_{-0.3}$     | $0.434^{+0.047}_{-0.037}$        | $1.369^{+0.199}_{-0.100}$       | $4.71^{+0.03}_{-0.03} \times 10^{-9}$              | $3.18^{+0.45}_{-0.22} \times 10^{-11}$               | 556.8 / 173  |
| 52.11                     | $0.60^{+0.01}_{-0.01}$                          | $41.4^{+0.1}_{-0.1}$     | —                                | $1.331^{+0.071}_{-0.067}$       | $4.93^{+0.03}_{-0.03} \times 10^{-9}$              | $3.29^{+0.41}_{-0.22} \times 10^{-11}$               | 817.8 / 176  |
| 52.254                    | $0.65^{+0.01}_{-0.01}$                          | $40.2^{+0.3}_{-0.2}$     | $0.457^{+0.044}_{-0.037}$        | $1.331^{+0.060}_{-0.059}$       | $4.12^{+0.01}_{-0.02} \times 10^{-9}$              | $3.51^{+0.31}_{-0.14} \times 10^{-11}$               | 1317.9 / 216 |
| 52.322                    | $0.64^{+0.01}_{-0.01}$                          | $40.8^{+0.1}_{-0.1}$     | $0.490^{+0.063}_{-0.084}$        | $1.368^{+0.097}_{-0.057}$       | $4.46^{+0.02}_{-0.02} \times 10^{-9}$              | $3.68^{+0.33}_{-0.20} \times 10^{-11}$               | 1046.7 / 197 |
| 52.393                    | $0.62^{+0.01}_{-0.01}$                          | $41.6^{+0.3}_{-0.3}$     | $0.459^{+0.046}_{-0.032}$        | $1.419^{+0.138}_{-0.098}$       | $4.42^{+0.02}_{-0.04} \times 10^{-9}$              | $4.05^{+0.30}_{-0.29} \times 10^{-11}$               | 816.0 / 187  |
| 52.461                    | $0.73^{+0.01}_{-0.01}$                          | $39.8^{+0.3}_{-0.3}$     | $0.457^{+0.026}_{-0.046}$        | $1.444^{+0.226}_{-0.176}$       | $4.33^{+0.02}_{-0.03} \times 10^{-9}$              | $4.14^{+0.25}_{-0.42} \times 10^{-11}$               | 553.1 / 176  |
| 52.576                    | $0.63^{+0.01}_{-0.01}$                          | $41.6^{+0.2}_{-0.1}$     | —                                | $1.336^{+0.077}_{-0.071}$       | $4.41^{+0.03}_{-0.03} \times 10^{-9}$              | $4.08^{+0.41}_{-0.37} \times 10^{-11}$               | 489.5 / 182  |
| 52.648                    | $0.66^{+0.01}_{-0.01}$                          | $40.4^{+0.4}_{-0.2}$     | $0.480^{+0.018}_{-0.038}$        | $1.440^{+0.091}_{-0.112}$       | $4.52^{+0.02}_{-0.02} \times 10^{-9}$              | $4.22^{+0.40}_{-0.18} \times 10^{-11}$               | 1062.2 / 216 |
| 52.916                    | $0.55^{+0.01}_{-0.01}$                          | $42.7^{+0.4}_{-0.2}$     | $0.456^{+0.051}_{-0.181}$        | $1.365^{+0.081}_{-0.053}$       | $4.59^{+0.01}_{-0.03} \times 10^{-9}$              | $3.70^{+0.28}_{-0.20} \times 10^{-11}$               | 968.4 / 210  |
| 52.983                    | $0.58^{+0.01}_{-0.01}$                          | $42.0^{+0.3}_{-0.2}$     | $0.439^{+0.036}_{-0.024}$        | $1.356^{+0.053}_{-0.086}$       | $4.08^{+0.02}_{-0.01} \times 10^{-9}$              | $3.62^{+0.24}_{-0.25} \times 10^{-11}$               | 1147.4 / 227 |
| 53.119                    | $0.59^{+0.01}_{-0.01}$                          | $41.8^{+0.1}_{-0.1}$     | $0.456^{+0.034}_{-0.052}$        | $1.374^{+0.110}_{-0.049}$       | $3.61^{+0.02}_{-0.03} \times 10^{-9}$              | $2.78^{+0.18}_{-0.16} \times 10^{-11}$               | 1092.3 / 213 |
| 53.187                    | $0.70^{+0.04}_{-0.04}$                          | $39.6^{+1.2}_{-1.2}$     | $0.448^{+1.052}_{-0.312}$        | —                               | $4.48^{+0.15}_{-0.15} \times 10^{-9}$              | $4.58^{+7.97}_{-2.18} \times 10^{-11}$               | 76.2 / 61    |
| 53.581                    | $0.60^{+0.01}_{-0.01}$                          | $41.1^{+0.3}_{-0.3}$     | $0.458^{+0.059}_{-0.045}$        | $1.370^{+0.147}_{-0.060}$       | $4.46^{+0.03}_{-0.03} \times 10^{-9}$              | $3.14^{+0.44}_{-0.27} \times 10^{-11}$               | 495.7 / 163  |
| 53.598                    | $0.55^{+0.01}_{-0.01}$                          | $42.7^{+0.3}_{-0.3}$     | $0.485^{+0.062}_{-0.063}$        | $1.436^{+0.129}_{-0.127}$       | $3.27^{+0.02}_{-0.02} \times 10^{-9}$              | $2.55^{+0.28}_{-0.29} \times 10^{-11}$               | 522.8 / 169  |
| 53.652                    | $0.52^{+0.01}_{-0.01}$                          | $43.3^{+0.1}_{-0.2}$     | —                                | $1.347^{+0.048}_{-0.060}$       | $4.64^{+0.02}_{-0.02} \times 10^{-9}$              | $3.73^{+0.28}_{-0.19} \times 10^{-11}$               | 1074.0 / 208 |

Continued on next page

Table 1 – continued from previous page

| $T_{\text{mid}}$<br>(day) | $N_{\text{H}}$<br>( $10^{22} \text{ cm}^{-2}$ ) | $kT_{\text{BB}}$<br>(eV) | APEC $kT_{\text{cool}}$<br>(keV) | APEC $kT_{\text{hot}}$<br>(keV) | BB Flux<br>( $\text{erg cm}^{-2} \text{ s}^{-1}$ ) | APEC Flux<br>( $\text{erg cm}^{-2} \text{ s}^{-1}$ ) | Cstat/dof    |
|---------------------------|-------------------------------------------------|--------------------------|----------------------------------|---------------------------------|----------------------------------------------------|------------------------------------------------------|--------------|
| 53.719                    | $0.62^{+0.01}_{-0.01}$                          | $41.4^{+0.2}_{-0.3}$     | $0.472^{+0.030}_{-0.028}$        | $1.435^{+0.167}_{-0.142}$       | $5.93^{+0.03}_{-0.03} \times 10^{-9}$              | $6.04^{+0.53}_{-0.27} \times 10^{-11}$               | 740.6 / 189  |
| 53.786                    | $0.62^{+0.01}_{-0.01}$                          | $41.1^{+0.3}_{-0.2}$     | $0.457^{+0.021}_{-0.029}$        | $1.387^{+0.095}_{-0.080}$       | $4.61^{+0.03}_{-0.02} \times 10^{-9}$              | $4.55^{+0.27}_{-0.23} \times 10^{-11}$               | 900.8 / 208  |
| 53.921                    | $0.67^{+0.01}_{-0.01}$                          | $39.7^{+0.3}_{-0.2}$     | $0.458^{+0.026}_{-0.032}$        | $1.432^{+0.111}_{-0.093}$       | $4.61^{+0.02}_{-0.02} \times 10^{-9}$              | $4.35^{+0.20}_{-0.35} \times 10^{-11}$               | 906.2 / 209  |
| 53.26                     | $0.68^{+0.01}_{-0.01}$                          | $40.5^{+0.4}_{-0.2}$     | $0.466^{+0.039}_{-0.034}$        | $1.446^{+0.098}_{-0.089}$       | $4.15^{+0.02}_{-0.02} \times 10^{-9}$              | $3.44^{+0.20}_{-0.20} \times 10^{-11}$               | 856.3 / 214  |
| 53.329                    | $0.64^{+0.01}_{-0.01}$                          | $41.0^{+0.3}_{-0.3}$     | $0.458^{+0.049}_{-0.041}$        | $1.357^{+0.072}_{-0.090}$       | $3.63^{+0.02}_{-0.02} \times 10^{-9}$              | $3.33^{+0.18}_{-0.26} \times 10^{-11}$               | 550.3 / 204  |
| 53.396                    | $0.63^{+0.01}_{-0.01}$                          | $41.7^{+0.4}_{-0.3}$     | $0.455^{+0.028}_{-0.036}$        | $1.490^{+0.310}_{-0.142}$       | $3.92^{+0.02}_{-0.02} \times 10^{-9}$              | $4.05^{+0.27}_{-0.39} \times 10^{-11}$               | 597.7 / 186  |
| 53.465                    | $0.75^{+0.01}_{-0.01}$                          | $39.1^{+0.2}_{-0.3}$     | $0.480^{+0.029}_{-0.050}$        | $1.441^{+0.288}_{-0.446}$       | $3.47^{+0.02}_{-0.02} \times 10^{-9}$              | $3.29^{+0.37}_{-0.21} \times 10^{-11}$               | 415.1 / 178  |
| 53.512                    | $0.64^{+0.01}_{-0.01}$                          | $41.2^{+0.1}_{-0.2}$     | $0.480^{+0.265}_{-0.095}$        | $1.423^{+0.200}_{-0.132}$       | $5.04^{+0.03}_{-0.04} \times 10^{-9}$              | $4.11^{+0.51}_{-0.39} \times 10^{-11}$               | 494.3 / 164  |
| 53.533                    | $0.81^{+0.02}_{-0.02}$                          | $39.5^{+0.4}_{-0.4}$     | $0.457^{+0.038}_{-0.042}$        | $1.531^{+1.018}_{-0.277}$       | $4.03^{+0.02}_{-0.04} \times 10^{-9}$              | $4.00^{+0.45}_{-0.30} \times 10^{-11}$               | 434.4 / 155  |
| 54.199                    | $0.56^{+0.01}_{-0.01}$                          | $42.9^{+0.3}_{-0.3}$     | $0.458^{+0.042}_{-0.169}$        | $1.371^{+0.102}_{-0.068}$       | $4.45^{+0.02}_{-0.03} \times 10^{-9}$              | $3.49^{+0.292}_{-0.28} \times 10^{-11}$              | 676.2 / 187  |
| 54.265                    | $0.63^{+0.01}_{-0.01}$                          | $41.3^{+0.3}_{-0.3}$     | $0.484^{+0.031}_{-0.049}$        | $1.511^{+0.136}_{-0.127}$       | $4.44^{+0.02}_{-0.03} \times 10^{-9}$              | $3.55^{+0.18}_{-0.37} \times 10^{-11}$               | 412.1 / 165  |
| 54.537                    | $0.72^{+0.01}_{-0.01}$                          | $39.8^{+0.3}_{-0.3}$     | $0.484^{+0.035}_{-0.059}$        | $1.452^{+0.217}_{-0.137}$       | $3.66^{+0.04}_{-0.02} \times 10^{-9}$              | $3.78^{+0.43}_{-0.37} \times 10^{-11}$               | 1064.2 / 176 |
| 54.59                     | $0.64^{+0.01}_{-0.01}$                          | $40.5^{+0.2}_{-0.3}$     | $0.466^{+0.059}_{-0.044}$        | $1.444^{+0.109}_{-0.097}$       | $4.18^{+0.02}_{-0.03} \times 10^{-9}$              | $3.02^{+0.23}_{-0.20} \times 10^{-11}$               | 747.0 / 213  |
| 54.667                    | $0.64^{+0.01}_{-0.01}$                          | $40.1^{+0.1}_{-0.1}$     | $0.469^{+0.052}_{-0.071}$        | $1.387^{+0.126}_{-0.067}$       | $4.44^{+0.02}_{-0.02} \times 10^{-9}$              | $3.31^{+0.29}_{-0.22} \times 10^{-11}$               | 1085.0 / 189 |
| 54.724                    | $0.66^{+0.01}_{-0.01}$                          | $39.8^{+0.3}_{-0.3}$     | $0.457^{+0.039}_{-0.042}$        | $1.401^{+0.100}_{-0.074}$       | $3.73^{+0.01}_{-0.02} \times 10^{-9}$              | $2.86^{+0.21}_{-0.22} \times 10^{-11}$               | 651.3 / 194  |
| 54.871                    | $0.66^{+0.01}_{-0.01}$                          | $39.4^{+0.2}_{-0.3}$     | $0.456^{+0.045}_{-0.056}$        | $1.443^{+0.208}_{-0.125}$       | $4.03^{+0.02}_{-0.03} \times 10^{-9}$              | $3.42^{+0.36}_{-0.50} \times 10^{-11}$               | 302.2 / 170  |
| 54.924                    | $0.59^{+0.01}_{-0.01}$                          | $41.4^{+0.2}_{-0.2}$     | $0.457^{+0.038}_{-0.176}$        | $1.362^{+0.073}_{-0.081}$       | $4.08^{+0.02}_{-0.02} \times 10^{-9}$              | $2.49^{+0.25}_{-0.25} \times 10^{-11}$               | 366.0 / 167  |
| 54.991                    | $0.65^{+0.01}_{-0.01}$                          | $40.1^{+0.1}_{-0.1}$     | $0.470^{+0.058}_{-0.058}$        | $1.355^{+0.086}_{-0.071}$       | $4.37^{+0.02}_{-0.02} \times 10^{-9}$              | $3.11^{+0.24}_{-0.18} \times 10^{-11}$               | 653.7 / 198  |
| 55.13                     | $0.54^{+0.01}_{-0.01}$                          | $42.5^{+0.2}_{-0.2}$     | $0.456^{+0.042}_{-0.206}$        | $1.298^{+0.081}_{-0.042}$       | $4.06^{+0.02}_{-0.03} \times 10^{-9}$              | $3.01^{+0.19}_{-0.23} \times 10^{-11}$               | 349.5 / 156  |
| 55.2                      | $0.74^{+0.01}_{-0.02}$                          | $39.2^{+0.3}_{-0.2}$     | $0.484^{+0.029}_{-0.033}$        | $1.447^{+0.203}_{-0.145}$       | $4.32^{+0.02}_{-0.02} \times 10^{-9}$              | $3.70^{+0.26}_{-0.23} \times 10^{-11}$               | 697.5 / 199  |
| 55.406                    | $0.70^{+0.01}_{-0.02}$                          | $40.0^{+0.3}_{-0.3}$     | $0.456^{+0.047}_{-0.048}$        | $1.552^{+0.287}_{-0.192}$       | $4.25^{+0.02}_{-0.03} \times 10^{-9}$              | $3.09^{+0.29}_{-0.31} \times 10^{-11}$               | 688.8 / 199  |
| 55.474                    | $0.80^{+0.01}_{-0.01}$                          | $38.8^{+0.3}_{-0.3}$     | $0.458^{+0.041}_{-0.067}$        | $1.440^{+0.298}_{-0.448}$       | $4.21^{+0.02}_{-0.03} \times 10^{-9}$              | $3.38^{+0.29}_{-0.35} \times 10^{-11}$               | 592.9 / 202  |
| 55.594                    | $0.65^{+0.01}_{-0.01}$                          | $41.2^{+0.4}_{-0.1}$     | $0.462^{+0.045}_{-0.030}$        | $1.370^{+0.162}_{-0.081}$       | $4.09^{+0.02}_{-0.02} \times 10^{-9}$              | $3.70^{+0.17}_{-0.49} \times 10^{-11}$               | 607.9 / 205  |
| 55.677                    | $0.71^{+0.02}_{-0.02}$                          | $39.7^{+0.5}_{-0.4}$     | $0.455^{+0.073}_{-0.080}$        | $1.540^{+1.095}_{-0.571}$       | $4.15^{+0.03}_{-0.05} \times 10^{-9}$              | $2.67^{+0.65}_{-0.28} \times 10^{-11}$               | 215.5 / 127  |
| 55.728                    | $0.61^{+0.01}_{-0.01}$                          | $41.9^{+0.3}_{-0.3}$     | $0.457^{+0.046}_{-0.032}$        | $1.414^{+0.158}_{-0.102}$       | $4.30^{+0.02}_{-0.02} \times 10^{-9}$              | $3.03^{+0.22}_{-0.20} \times 10^{-11}$               | 867.1 / 197  |
| 55.805                    | $0.75^{+0.02}_{-0.01}$                          | $39.6^{+0.2}_{-0.3}$     | $0.459^{+0.044}_{-0.031}$        | $1.376^{+0.186}_{-0.098}$       | $4.49^{+0.02}_{-0.03} \times 10^{-9}$              | $2.78^{+0.41}_{-0.29} \times 10^{-11}$               | 668.1 / 186  |
| 55.861                    | $0.74^{+0.01}_{-0.01}$                          | $39.7^{+0.2}_{-0.2}$     | $0.458^{+0.029}_{-0.030}$        | $1.455^{+0.359}_{-0.162}$       | $4.24^{+0.02}_{-0.02} \times 10^{-9}$              | $4.09^{+0.28}_{-0.35} \times 10^{-11}$               | 510.6 / 191  |
| 55.929                    | $0.58^{+0.01}_{-0.01}$                          | $42.0^{+0.5}_{-0.1}$     | $0.456^{+0.034}_{-0.043}$        | $1.369^{+0.126}_{-0.086}$       | $4.58^{+0.02}_{-0.02} \times 10^{-9}$              | $3.00^{+0.21}_{-0.21} \times 10^{-11}$               | 957.2 / 200  |
| 55.995                    | $0.75^{+0.01}_{-0.01}$                          | $39.7^{+0.3}_{-0.2}$     | $0.476^{+0.027}_{-0.034}$        | $1.358^{+0.191}_{-0.163}$       | $4.59^{+0.02}_{-0.02} \times 10^{-9}$              | $3.60^{+0.25}_{-0.21} \times 10^{-11}$               | 638.3 / 207  |
| 56.063                    | $0.58^{+0.01}_{-0.01}$                          | $42.2^{+0.3}_{-0.3}$     | $0.458^{+0.056}_{-0.042}$        | $1.369^{+0.134}_{-0.061}$       | $3.96^{+0.02}_{-0.02} \times 10^{-9}$              | $3.04^{+0.21}_{-0.20} \times 10^{-11}$               | 868.6 / 194  |
| 56.134                    | $0.59^{+0.01}_{-0.01}$                          | $42.1^{+0.2}_{-0.2}$     | $0.462^{+0.064}_{-0.051}$        | $1.301^{+0.133}_{-0.061}$       | $3.97^{+0.02}_{-0.02} \times 10^{-9}$              | $2.90^{+0.20}_{-0.21} \times 10^{-11}$               | 711.8 / 194  |
| 56.205                    | $0.60^{+0.01}_{-0.01}$                          | $41.9^{+0.4}_{-0.2}$     | $0.437^{+0.059}_{-0.042}$        | $1.365^{+0.070}_{-0.088}$       | $4.08^{+0.02}_{-0.02} \times 10^{-9}$              | $2.95^{+0.31}_{-0.14} \times 10^{-11}$               | 698.9 / 185  |
| 56.274                    | $0.64^{+0.01}_{-0.01}$                          | $42.0^{+0.3}_{-0.1}$     | $0.485^{+0.040}_{-0.021}$        | $1.435^{+0.209}_{-0.146}$       | $4.36^{+0.01}_{-0.02} \times 10^{-9}$              | $3.44^{+0.38}_{-0.23} \times 10^{-11}$               | 567.9 / 188  |
| 56.342                    | $0.70^{+0.01}_{-0.01}$                          | $40.3^{+0.3}_{-0.3}$     | $0.458^{+0.044}_{-0.030}$        | $1.537^{+0.248}_{-0.170}$       | $4.32^{+0.02}_{-0.02} \times 10^{-9}$              | $3.24^{+0.40}_{-0.19} \times 10^{-11}$               | 454.9 / 161  |
| 56.411                    | $0.65^{+0.01}_{-0.02}$                          | $40.9^{+0.4}_{-0.3}$     | $0.458^{+0.049}_{-0.070}$        | $1.362^{+0.284}_{-0.421}$       | $4.56^{+0.03}_{-0.03} \times 10^{-9}$              | $2.86^{+0.36}_{-0.24} \times 10^{-11}$               | 353.8 / 160  |
| 56.478                    | $0.65^{+0.01}_{-0.01}$                          | $40.7^{+0.1}_{-0.1}$     | $0.458^{+0.048}_{-0.064}$        | $1.281^{+0.132}_{-0.112}$       | $4.00^{+0.02}_{-0.02} \times 10^{-9}$              | $3.40^{+0.34}_{-0.27} \times 10^{-11}$               | 394.8 / 148  |
| 56.542                    | $0.66^{+0.01}_{-0.01}$                          | $40.5^{+0.4}_{-0.2}$     | $0.457^{+0.044}_{-0.038}$        | $1.482^{+0.185}_{-0.129}$       | $4.01^{+0.02}_{-0.02} \times 10^{-9}$              | $2.84^{+0.27}_{-0.18} \times 10^{-11}$               | 515.0 / 198  |
| 56.604                    | $0.62^{+0.01}_{-0.01}$                          | $40.7^{+0.4}_{-0.1}$     | $0.456^{+0.045}_{-0.049}$        | $1.329^{+0.095}_{-0.072}$       | $3.83^{+0.02}_{-0.02} \times 10^{-9}$              | $2.73^{+0.16}_{-0.22} \times 10^{-11}$               | 715.5 / 191  |
| 56.671                    | $0.68^{+0.01}_{-0.01}$                          | $39.6^{+0.3}_{-0.3}$     | $0.459^{+0.036}_{-0.029}$        | $1.445^{+0.126}_{-0.118}$       | $3.82^{+0.02}_{-0.02} \times 10^{-9}$              | $3.37^{+0.16}_{-0.39} \times 10^{-11}$               | 643.8 / 191  |
| 56.74                     | $0.71^{+0.01}_{-0.01}$                          | $39.4^{+0.2}_{-0.1}$     | $0.455^{+0.033}_{-0.053}$        | $1.451^{+0.196}_{-0.089}$       | $4.28^{+0.02}_{-0.02} \times 10^{-9}$              | $3.78^{+0.36}_{-0.27} \times 10^{-11}$               | 527.8 / 191  |
| 56.806                    | $0.69^{+0.01}_{-0.02}$                          | $39.6^{+0.4}_{-0.2}$     | $0.452^{+0.041}_{-0.042}$        | $1.350^{+0.143}_{-0.100}$       | $4.34^{+0.02}_{-0.02} \times 10^{-9}$              | $3.32^{+0.39}_{-0.20} \times 10^{-11}$               | 486.4 / 183  |
| 56.875                    | $0.54^{+0.01}_{-0.01}$                          | $42.5^{+0.1}_{-0.2}$     | $0.159^{+1.297}_{-0.159}$        | $1.262^{+0.471}_{-1.107}$       | $4.72^{+0.03}_{-0.04} \times 10^{-9}$              | $2.57^{+0.43}_{-0.34} \times 10^{-11}$               | 405.3 / 147  |
| 56.934                    | $0.61^{+0.01}_{-0.01}$                          | $41.1^{+0.2}_{-0.2}$     | $0.453^{+0.037}_{-0.044}$        | $1.369^{+0.129}_{-0.077}$       | $4.24^{+0.02}_{-0.02} \times 10^{-9}$              | $3.03^{+0.21}_{-0.31} \times 10^{-11}$               | 743.5 / 208  |
| 57.068                    | $0.71^{+0.01}_{-0.02}$                          | $39.6^{+0.3}_{-0.2}$     | $0.462^{+0.045}_{-0.045}$        | $1.384^{+0.160}_{-0.112}$       | $4.01^{+0.02}_{-0.02} \times 10^{-9}$              | $3.03^{+0.24}_{-0.20} \times 10^{-11}$               | 703.6 / 191  |
| 57.138                    | $0.67^{+0.01}_{-0.01}$                          | $40.2^{+0.3}_{-0.2}$     | $0.434^{+0.031}_{-0.017}$        | $1.301^{+0.158}_{-0.086}$       | $4.14^{+0.01}_{-0.02} \times 10^{-9}$              | $3.34^{+0.18}_{-0.27} \times 10^{-11}$               | 781.0 / 192  |
| 58.281                    | $0.59^{+0.01}_{-0.01}$                          | $41.0^{+0.2}_{-0.2}$     | $0.454^{+0.068}_{-0.077}$        | $1.377^{+0.193}_{-0.102}$       | $4.28^{+0.02}_{-0.03} \times 10^{-9}$              | $1.92^{+0.21}_{-0.31} \times 10^{-11}$               | 592.8 / 168  |
| 58.812                    | $0.63^{+0.01}_{-0.01}$                          | $39.8^{+0.4}_{-0.2}$     | $0.481^{+0.115}_{-0.051}$        | $1.366^{+0.125}_{-0.076}$       | $3.40^{+0.01}_{-0.02} \times 10^{-9}$              | $2.05^{+0.23}_{-0.13} \times 10^{-11}$               | 737.4 / 189  |
| 59.542                    | $0.68^{+0.01}_{-0.02}$                          | $38.9^{+0.4}_{-0.2}$     | $0.459^{+0.038}_{-0.028}$        | $1.366^{+0.222}_{-0.137}$       | $4.12^{+0.02}_{-0.03} \times 10^{-9}$              | $3.12^{+0.33}_{-0.19} \times 10^{-11}$               | 444.1 / 173  |
| 61.293                    | $0.54^{+0.01}_{-0.01}$                          | $42.3^{+0.4}_{-0.3}$     | $0.457^{+0.056}_{-0.054}$        | $1.542^{+0.300}_{-0.207}$       | $3.48^{+0.02}_{-0.02} \times 10^{-9}$              | $2.01^{+0.27}_{-0.21} \times 10^{-11}$               | 432.9 / 159  |
| 61.358                    | $0.61^{+0.01}_{-0.01}$                          | $41.4^{+0.3}_{-0.4}$     | $0.451^{+0.049}_{-0.050}$        | —                               | $3.58^{+0.02}_{-0.02} \times 10^{-9}$              | $2.78^{+0.34}_{-0.27} \times 10^{-11}$               | 210.1 / 145  |
| 61.83                     | $0.58^{+0.01}_{-0.01}$                          | $40.6^{+0.2}_{-0.3}$     | $0.427^{+0.097}_{-0.082}$        | $1.316^{+0.363}_{-0.137}$       | $4.03^{+0.03}_{-0.04} \times 10^{-9}$              | $2.65^{+0.49}_{-0.34} \times 10^{-11}$               | 225.6 / 142  |
| 61.897                    | $0.62^{+0.01}_{-0.01}$                          | $40.2^{+0.7}_{-0.2}$     | $0.473^{+0.043}_{-0.069}$        | $1.294^{+1.411}_{-0.732}$       | $3.33^{+0.02}_{-0.03} \times 10^{-9}$              | $2.42^{+0.29}_{-0.29} \times 10^{-11}$               | 291.6 / 141  |
| 62.231                    | $0.56^{+0.01}_{-0.01}$                          | $41.8^{+0.3}_{-0.1}$     | $0.459^{+0.068}_{-0.062}$        | $1.286^{+0.151}_{-0.131}$       | $3.79^{+0.02}_{-0.03} \times 10^{-9}$              | $2.80^{+0.50}_{-0.40} \times 10^{-11}$               | 368.4 / 139  |
| 62.298                    | $0.57^{+0.01}_{-0.01}$                          | $42.3^{+0.3}_{-0.4}$     | $0.458^{+0.069}_{-0.060}$        | $1.437^{+0.203}_{-0.154}$       | $3.95^{+0.02}_{-0.03} \times 10^{-9}$              | $2.31^{+0.41}_{-0.18} \times 10^{-11}$               | 300.9 / 155  |
| 62.836                    | $0.58^{+0.01}_{-0.02}$                          | $41.2^{+0.6}_{-0.3}$     | $0.434^{+0.066}_{-0.057}$        | $1.294^{+0.305}_{-0.139}$       | $3.84^{+0.03}_{-0.03} \times 10^{-9}$              | $2.62^{+0.41}_{-0.20} \times 10^{-11}$               | 234.6 / 151  |
| 62.902                    | $0.60^{+0.01}_{-0.01}$                          | $40.6^{+0.4}_{-0.4}$     | $0.449^{+0.069}_{-0.069}$        | $1.368^{+0.265}_{-0.157}$       | $3.44^{+0.02}_{-0.03} \times 10^{-9}$              | $2.33^{+0.27}_{-0.27} \times 10^{-11}$               | 246.5 / 135  |
| 63.169                    | $0.56^{+0.02}_{-0.01}$                          | $41.9^{+0.4}_{-0.5}$     | $0.402^{+0.220}_{-0.253}$        | $1.216^{+0.432}_{-0.152}$       | $3.39^{+0.03}_{-0.03} \times 10^{-9}$              | $1.74^{+0.46}_{-0.26} \times 10^{-11}$               | 143.0 / 118  |

Continued on next page



Table 1 – continued from previous page

| $T_{\text{mid}}$<br>(day) | $N_{\text{H}}$<br>( $10^{22} \text{ cm}^{-2}$ ) | $kT_{\text{BB}}$<br>(eV) | APEC $kT_{\text{cool}}$<br>(keV) | APEC $kT_{\text{hot}}$<br>(keV) | BB Flux<br>( $\text{erg cm}^{-2} \text{ s}^{-1}$ ) | APEC Flux<br>( $\text{erg cm}^{-2} \text{ s}^{-1}$ ) | Cstat/dof    |
|---------------------------|-------------------------------------------------|--------------------------|----------------------------------|---------------------------------|----------------------------------------------------|------------------------------------------------------|--------------|
| 63.238                    | $0.59^{+0.01}_{-0.02}$                          | $40.8^{+0.4}_{-0.5}$     | $0.460^{+0.077}_{-0.064}$        | $1.295^{+0.241}_{-0.342}$       | $3.67^{+0.03}_{-0.03} \times 10^{-9}$              | $2.53^{+0.27}_{-0.57} \times 10^{-11}$               | 196.1 / 128  |
| 63.839                    | $0.64^{+0.01}_{-0.01}$                          | $39.2^{+0.2}_{-0.3}$     | $0.454^{+0.160}_{-0.076}$        | $1.363^{+0.511}_{-0.231}$       | $3.42^{+0.02}_{-0.02} \times 10^{-9}$              | $1.55^{+0.30}_{-0.21} \times 10^{-11}$               | 212.8 / 135  |
| 63.906                    | $0.56^{+0.01}_{-0.01}$                          | $41.2^{+0.3}_{-0.2}$     | $0.434^{+0.060}_{-0.058}$        | $1.359^{+0.198}_{-0.129}$       | $3.62^{+0.02}_{-0.03} \times 10^{-9}$              | $2.92^{+0.34}_{-0.32} \times 10^{-11}$               | 305.5 / 146  |
| 64.178                    | $0.61^{+0.01}_{-0.02}$                          | $40.5^{+0.6}_{-0.2}$     | $0.416^{+0.200}_{-0.217}$        | —                               | $3.43^{+0.02}_{-0.03} \times 10^{-9}$              | $2.86^{+0.67}_{-0.31} \times 10^{-11}$               | 172.0 / 144  |
| 64.241                    | $0.54^{+0.01}_{-0.01}$                          | $41.2^{+0.3}_{-0.2}$     | $0.447^{+0.026}_{-0.055}$        | $1.211^{+0.488}_{-0.418}$       | $4.09^{+0.03}_{-0.03} \times 10^{-9}$              | $4.88^{+0.67}_{-0.46} \times 10^{-11}$               | 196.5 / 132  |
| 65.783                    | $0.59^{+0.01}_{-0.02}$                          | $40.6^{+0.5}_{-0.3}$     | $0.455^{+0.061}_{-0.057}$        | $1.635^{+0.227}_{-0.608}$       | $2.99^{+0.02}_{-0.02} \times 10^{-9}$              | $2.64^{+0.25}_{-0.32} \times 10^{-11}$               | 190.5 / 156  |
| 65.848                    | $0.59^{+0.01}_{-0.01}$                          | $40.4^{+0.5}_{-0.3}$     | $0.453^{+0.040}_{-0.052}$        | $1.148^{+0.134}_{-0.086}$       | $3.02^{+0.02}_{-0.02} \times 10^{-9}$              | $2.86^{+0.21}_{-0.30} \times 10^{-11}$               | 248.3 / 160  |
| 65.918                    | $0.64^{+0.01}_{-0.01}$                          | $39.9^{+0.3}_{-0.3}$     | $0.458^{+0.040}_{-0.034}$        | —                               | $3.19^{+0.02}_{-0.02} \times 10^{-9}$              | $1.96^{+0.25}_{-0.20} \times 10^{-11}$               | 263.8 / 158  |
| 66.788                    | $0.57^{+0.02}_{-0.01}$                          | $40.7^{+0.4}_{-0.5}$     | $0.457^{+0.076}_{-0.143}$        | $1.384^{+0.165}_{-0.168}$       | $3.13^{+0.02}_{-0.02} \times 10^{-9}$              | $2.10^{+0.27}_{-0.25E} \times 10^{-11}$              | 168.0 / 147  |
| 66.856                    | $0.57^{+0.01}_{-0.01}$                          | $40.4^{+0.2}_{-0.2}$     | $0.480^{+0.062}_{-0.030}$        | $1.356^{+0.380}_{-0.446}$       | $3.23^{+0.02}_{-0.02} \times 10^{-9}$              | $3.09^{+0.47}_{-0.20E} \times 10^{-11}$              | 177.2 / 154  |
| 66.922                    | $0.59^{+0.01}_{-0.01}$                          | $40.0^{+0.4}_{-0.2}$     | $0.432^{+0.069}_{-0.068}$        | $1.231^{+0.406}_{-0.346}$       | $3.21^{+0.02}_{-0.03} \times 10^{-9}$              | $2.50^{+0.46}_{-0.27E} \times 10^{-11}$              | 194.8 / 138  |
| 66.99                     | $0.59^{+0.01}_{-0.01}$                          | $40.2^{+0.4}_{-0.4}$     | $0.433^{+0.068}_{-0.050}$        | $1.640^{+0.390}_{-0.493}$       | $3.26^{+0.02}_{-0.02} \times 10^{-9}$              | $2.83^{+0.39}_{-0.28E} \times 10^{-11}$              | 178.2 / 147  |
| 67.178                    | $0.56^{+0.01}_{-0.02}$                          | $40.1^{+0.5}_{-0.3}$     | $0.423^{+0.099}_{-0.098}$        | $1.363^{+0.493}_{-0.568}$       | $3.12^{+0.02}_{-0.03} \times 10^{-9}$              | $2.48^{+0.23}_{-0.44E} \times 10^{-11}$              | 195.5 / 130  |
| 68.323                    | $0.58^{+0.01}_{-0.01}$                          | $39.6^{+0.4}_{-0.2}$     | $0.434^{+0.044}_{-0.039}$        | $1.358^{+0.198}_{-0.142}$       | $2.88^{+0.01}_{-0.01} \times 10^{-9}$              | $2.62^{+0.22}_{-0.19E} \times 10^{-11}$              | 347.6 / 196  |
| 68.39                     | $0.54^{+0.01}_{-0.01}$                          | $40.5^{+0.4}_{-0.2}$     | $0.439^{+0.041}_{-0.049}$        | $1.206^{+0.131}_{-0.115}$       | $2.70^{+0.01}_{-0.01} \times 10^{-9}$              | $2.47^{+0.22}_{-0.18E} \times 10^{-11}$              | 286.1 / 183  |
| 69.327                    | $0.48^{+0.01}_{-0.01}$                          | $41.5^{+0.4}_{-0.3}$     | $0.500^{+0.060}_{-0.091}$        | $1.234^{+0.263}_{-0.142}$       | $2.66^{+0.01}_{-0.01} \times 10^{-9}$              | $2.07^{+0.18}_{-0.23E} \times 10^{-11}$              | 296.6 / 168  |
| 69.394                    | $0.56^{+0.01}_{-0.01}$                          | $39.4^{+0.2}_{-0.1}$     | $0.456^{+0.023}_{-0.043}$        | —                               | $2.66^{+0.02}_{-0.01} \times 10^{-9}$              | $2.55^{+0.16}_{-0.22} \times 10^{-11}$               | 195.7 / 164  |
| 70.264                    | $0.51^{+0.01}_{-0.01}$                          | $40.6^{+0.4}_{-0.3}$     | $0.466^{+0.064}_{-0.044}$        | $1.326^{+0.250}_{-0.183}$       | $2.56^{+0.01}_{-0.01} \times 10^{-9}$              | $1.97^{+0.16}_{-0.27} \times 10^{-11}$               | 300.2 / 176  |
| 70.331                    | $0.63^{+0.01}_{-0.01}$                          | $38.2^{+0.3}_{-0.3}$     | $0.479^{+0.036}_{-0.077}$        | —                               | $2.56^{+0.02}_{-0.02} \times 10^{-9}$              | $2.47^{+0.19}_{-0.19} \times 10^{-11}$               | 251.5 / 168  |
| 72.011                    | $0.55^{+0.01}_{-0.01}$                          | $39.0^{+0.5}_{-0.5}$     | $0.450^{+0.077}_{-0.099}$        | $1.218^{+0.217}_{-0.150}$       | $2.20^{+0.02}_{-0.02} \times 10^{-9}$              | $1.55^{+0.19}_{-0.26} \times 10^{-11}$               | 179.7 / 146  |
| 72.079                    | $0.67^{+0.01}_{-0.02}$                          | $36.9^{+0.5}_{-0.3}$     | $0.433^{+0.045}_{-0.060}$        | —                               | $2.16^{+0.01}_{-0.01} \times 10^{-9}$              | $2.31^{+0.21}_{-0.23} \times 10^{-11}$               | 199.7 / 149  |
| 72.146                    | $0.53^{+0.01}_{-0.01}$                          | $39.6^{+0.2}_{-0.4}$     | $0.485^{+0.081}_{-0.055}$        | $1.227^{+0.873}_{-0.848}$       | $2.13^{+0.01}_{-0.01} \times 10^{-9}$              | $1.92^{+0.26}_{-0.17} \times 10^{-11}$               | 182.6 / 150  |
| 72.953                    | $0.66^{+0.04}_{-0.03}$                          | $36.8^{+0.5}_{-0.9}$     | $0.572^{+0.313}_{-0.422}$        | —                               | $2.14^{+0.03}_{-0.03} \times 10^{-9}$              | $1.89^{+0.50}_{-0.47} \times 10^{-11}$               | 55.7 / 66    |
| 73.016                    | $0.56^{+0.01}_{-0.01}$                          | $38.8^{+0.5}_{-0.2}$     | $0.545^{+0.084}_{-0.058}$        | $1.445^{+0.459}_{-0.248}$       | $2.22^{+0.02}_{-0.02} \times 10^{-9}$              | $1.43^{+0.27}_{-0.14} \times 10^{-11}$               | 186.2 / 150  |
| 73.083                    | $0.60^{+0.01}_{-0.01}$                          | $37.6^{+0.2}_{-0.4}$     | $0.405^{+0.031}_{-0.030}$        | —                               | $2.21^{+0.02}_{-0.02} \times 10^{-9}$              | $1.64^{+0.17}_{-0.19} \times 10^{-11}$               | 142.9 / 140  |
| 73.885                    | $0.57^{+0.03}_{-0.02}$                          | $37.5^{+0.7}_{-0.8}$     | $0.291^{+0.149}_{-0.085}$        | —                               | $2.29^{+0.02}_{-0.03} \times 10^{-9}$              | $2.58^{+0.19}_{-0.66} \times 10^{-11}$               | 102.6 / 115  |
| 73.952                    | $0.53^{+0.02}_{-0.02}$                          | $38.3^{+0.6}_{-0.4}$     | $0.394^{+0.123}_{-0.080}$        | —                               | $2.17^{+0.02}_{-0.02} \times 10^{-9}$              | $2.67^{+0.61}_{-0.29} \times 10^{-11}$               | 130.3 / 124  |
| 74.021                    | $0.52^{+0.01}_{-0.01}$                          | $38.7^{+0.3}_{-1.1}$     | $0.374^{+0.095}_{-0.179}$        | —                               | $2.25^{+0.02}_{-0.03} \times 10^{-9}$              | $1.63^{+0.51}_{-0.27} \times 10^{-11}$               | 157.5 / 110  |
| 74.084                    | $0.59^{+0.02}_{-0.02}$                          | $37.0^{+0.4}_{-0.7}$     | $0.457^{+0.604}_{-0.457}$        | $0.868^{+0.181}_{-0.200}$       | $1.94^{+0.02}_{-0.02} \times 10^{-9}$              | $1.90^{+0.41}_{-0.20} \times 10^{-11}$               | 115.0 / 125  |
| 74.148                    | $0.60^{+0.02}_{-0.02}$                          | $36.7^{+0.5}_{-0.5}$     | $0.333^{+0.055}_{-0.041}$        | —                               | $1.99^{+0.01}_{-0.01} \times 10^{-9}$              | $2.78^{+0.37}_{-0.37} \times 10^{-11}$               | 170.3 / 136  |
| 74.828                    | $0.57^{+0.03}_{-0.03}$                          | $36.4^{+0.8}_{-0.8}$     | $0.468^{+0.147}_{-0.132}$        | —                               | $1.71^{+0.02}_{-0.02} \times 10^{-9}$              | $2.49^{+0.83}_{-0.75} \times 10^{-11}$               | 140.8 / 113  |
| 74.887                    | $0.65^{+0.01}_{-0.01}$                          | $35.1^{+0.4}_{-0.3}$     | $0.313^{+0.034}_{-0.037}$        | $2.845^{+3.060}_{-2.845}$       | $1.79^{+0.01}_{-0.01} \times 10^{-9}$              | $2.18^{+0.19}_{-0.26} \times 10^{-11}$               | 227.8 / 166  |
| 76.895                    | $0.67^{+0.01}_{-0.02}$                          | $33.8^{+0.5}_{-0.3}$     | $0.372^{+0.089}_{-0.059}$        | —                               | $1.83^{+0.01}_{-0.01} \times 10^{-9}$              | $2.13^{+0.22}_{-0.26} \times 10^{-11}$               | 343.6 / 154  |
| 76.961                    | $0.52^{+0.01}_{-0.02}$                          | $35.9^{+0.4}_{-0.4}$     | $0.478^{+0.115}_{-0.099}$        | —                               | $1.77^{+0.01}_{-0.01} \times 10^{-9}$              | $1.86^{+0.21}_{-0.20} \times 10^{-11}$               | 235.3 / 139  |
| 77.028                    | $0.46^{+0.01}_{-0.01}$                          | $37.4^{+0.5}_{-0.2}$     | $0.394^{+0.104}_{-0.072}$        | $1.016^{+0.286}_{-0.181}$       | $1.73^{+0.01}_{-0.01} \times 10^{-9}$              | $1.39^{+0.41}_{-0.17} \times 10^{-11}$               | 216.5 / 127  |
| 78.826                    | $0.66^{+0.02}_{-0.02}$                          | $32.5^{+0.6}_{-0.5}$     | $0.604^{+0.126}_{-0.099}$        | —                               | $1.33^{+0.01}_{-0.01} \times 10^{-9}$              | $2.19^{+0.26}_{-0.19} \times 10^{-11}$               | 236.8 / 142  |
| 80.176                    | $0.63^{+0.03}_{-0.03}$                          | $31.9^{+0.7}_{-0.7}$     | $0.370^{+0.103}_{-0.080}$        | $0.968^{+0.164}_{-0.161}$       | $1.21^{+0.01}_{-0.01} \times 10^{-9}$              | $1.85^{+0.22}_{-0.22} \times 10^{-11}$               | 138.3 / 121  |
| 80.236                    | $0.63^{+0.02}_{-0.02}$                          | $32.2^{+0.4}_{-0.5}$     | —                                | $0.690^{+0.085}_{-0.065}$       | $1.21^{+0.01}_{-0.01} \times 10^{-9}$              | $1.62^{+0.34}_{-0.21} \times 10^{-11}$               | 283.6 / 148  |
| 80.299                    | $0.56^{+0.04}_{-0.02}$                          | $32.5^{+0.5}_{-0.8}$     | —                                | $0.717^{+0.138}_{-0.152}$       | $1.28^{+0.02}_{-0.02} \times 10^{-9}$              | $1.96^{+0.57}_{-0.32} \times 10^{-11}$               | 179.6 / 117  |
| <b>2021 eruption</b>      |                                                 |                          |                                  |                                 |                                                    |                                                      |              |
| 0.371                     | $21.84^{+2.25}_{-1.91}$                         | —                        | $0.354^{+0.052}_{-0.043}$        | $5.805^{+0.616}_{-0.767}$       | —                                                  | $4.75^{+0.13}_{-0.15} \times 10^{-10}$               | 626.9 / 673  |
| 0.415                     | $28.11^{+4.45}_{-3.61}$                         | —                        | $0.277^{+0.075}_{-0.025}$        | $5.733^{+1.159}_{-1.515}$       | —                                                  | $5.86^{+0.48}_{-0.37} \times 10^{-10}$               | 295.6 / 421  |
| 1.229                     | $8.89^{+0.48}_{-0.45}$                          | —                        | $0.164^{+0.025}_{-0.032}$        | $6.219^{+0.600}_{-0.516}$       | —                                                  | $7.27^{+0.15}_{-0.14} \times 10^{-10}$               | 769.1 / 778  |
| 2.892                     | $8.57^{+0.36}_{-0.38}$                          | —                        | $0.186^{+0.011}_{-0.008}$        | $8.149^{+0.652}_{-0.435}$       | —                                                  | $1.09^{+0.02}_{-0.01} \times 10^{-9}$                | 956.3 / 834  |
| 4.01                      | $3.84^{+0.18}_{-0.13}$                          | —                        | $0.125^{+0.000}_{-0.125}$        | $12.570^{+1.331}_{-1.573}$      | —                                                  | $1.27^{+0.01}_{-0.01} \times 10^{-9}$                | 1023.9 / 835 |
| 4.21                      | $4.07^{+0.37}_{-0.35}$                          | —                        | $0.133^{+0.029}_{-0.133}$        | $8.166^{+0.900}_{-0.816}$       | —                                                  | $7.26^{+0.22}_{-0.15} \times 10^{-10}$               | 635.0 / 657  |
| 5.675                     | $3.00^{+0.17}_{-0.20}$                          | —                        | $0.177^{+0.037}_{-0.021}$        | $20.620^{+11.181}_{-4.377}$     | —                                                  | $1.22^{+0.04}_{-0.02} \times 10^{-9}$                | 792.0 / 802  |
| 5.682                     | $3.89^{+0.05}_{-0.04}$                          | —                        | $0.147^{+0.013}_{-0.013}$        | $7.780^{+0.561}_{-0.487}$       | —                                                  | $9.32^{+0.14}_{-0.21} \times 10^{-10}$               | 706.4 / 713  |
| 6.605                     | $2.85^{+0.11}_{-0.15}$                          | —                        | $0.150^{+0.018}_{-0.011}$        | $9.238^{+0.794}_{-0.761}$       | —                                                  | $1.07^{+0.01}_{-0.02} \times 10^{-9}$                | 851.8 / 762  |
| 6.612                     | $2.41^{+0.33}_{-0.32}$                          | —                        | $0.263^{+0.053}_{-0.068}$        | $12.296^{+4.614}_{-2.572}$      | —                                                  | $1.01^{+0.03}_{-0.03} \times 10^{-9}$                | 687.9 / 717  |
| 9.988                     | $1.72^{+0.12}_{-0.13}$                          | —                        | $0.739^{+0.046}_{-0.047}$        | $4.662^{+0.365}_{-0.406}$       | —                                                  | $6.17^{+0.17}_{-0.16} \times 10^{-10}$               | 669.6 / 646  |
| 9.995                     | $2.14^{+0.15}_{-0.17}$                          | —                        | $0.800^{+0.068}_{-0.074}$        | $3.787^{+0.219}_{-0.219}$       | —                                                  | $6.23^{+0.13}_{-0.16} \times 10^{-10}$               | 676.9 / 710  |
| 10.519                    | $1.75^{+0.12}_{-0.14}$                          | —                        | $0.708^{+0.063}_{-0.076}$        | $3.640^{+0.220}_{-0.197}$       | —                                                  | $3.33^{+0.07}_{-0.04} \times 10^{-10}$               | 601.3 / 628  |
| 10.526                    | $1.67^{+0.12}_{-0.12}$                          | —                        | $0.670^{+0.059}_{-0.079}$        | $4.335^{+0.285}_{-0.242}$       | —                                                  | $5.82^{+0.18}_{-0.18} \times 10^{-10}$               | 767.8 / 653  |
| 11.846                    | $1.66^{+0.12}_{-0.13}$                          | —                        | $0.740^{+0.049}_{-0.060}$        | $3.631^{+0.238}_{-0.205}$       | —                                                  | $4.94^{+0.12}_{-0.12} \times 10^{-10}$               | 590.8 / 620  |
| 11.853                    | $1.97^{+0.14}_{-0.16}$                          | —                        | $0.714^{+0.050}_{-0.061}$        | $3.635^{+0.403}_{-0.295}$       | —                                                  | $3.72^{+0.13}_{-0.11} \times 10^{-10}$               | 522.8 / 562  |
| 12.576                    | $1.59^{+0.12}_{-0.14}$                          | —                        | $0.694^{+0.044}_{-0.048}$        | $3.398^{+0.222}_{-0.192}$       | —                                                  | $4.47^{+0.10}_{-0.12} \times 10^{-10}$               | 674.6 / 586  |

Continued on next page

Table 1 – continued from previous page

| $T_{\text{mid}}$<br>(day) | $N_{\text{H}}$<br>( $10^{22} \text{ cm}^{-2}$ ) | $kT_{\text{BB}}$<br>(eV) | APEC $kT_{\text{cool}}$<br>(keV) | APEC $kT_{\text{hot}}$<br>(keV) | BB Flux<br>( $\text{erg cm}^{-2} \text{ s}^{-1}$ ) | APEC Flux<br>( $\text{erg cm}^{-2} \text{ s}^{-1}$ ) | Cstat/dof   |
|---------------------------|-------------------------------------------------|--------------------------|----------------------------------|---------------------------------|----------------------------------------------------|------------------------------------------------------|-------------|
| 12.583                    | $1.66^{+0.10}_{-0.10}$                          | —                        | $0.743^{+0.040}_{-0.047}$        | $3.172^{+0.157}_{-0.140}$       | —                                                  | $4.68^{+0.11}_{-0.07} \times 10^{-10}$               | 643.5 / 622 |
| 13.571                    | $1.76^{+0.10}_{-0.10}$                          | —                        | $0.792^{+0.032}_{-0.036}$        | $2.892^{+0.208}_{-0.164}$       | —                                                  | $3.82^{+0.10}_{-0.09} \times 10^{-10}$               | 555.5 / 544 |
| 13.578                    | $1.78^{+0.09}_{-0.10}$                          | —                        | $0.655^{+0.051}_{-0.063}$        | $2.807^{+0.146}_{-0.136}$       | —                                                  | $4.45^{+0.10}_{-0.09} \times 10^{-10}$               | 619.5 / 599 |
| 14.7                      | $1.67^{+0.09}_{-0.11}$                          | —                        | $0.658^{+0.041}_{-0.041}$        | $2.623^{+0.156}_{-0.131}$       | —                                                  | $2.78^{+0.06}_{-0.05} \times 10^{-10}$               | 563.7 / 544 |
| 14.707                    | $1.77^{+0.12}_{-0.15}$                          | —                        | $0.755^{+0.047}_{-0.050}$        | $2.706^{+0.343}_{-0.247}$       | —                                                  | $3.62^{+0.12}_{-0.12} \times 10^{-10}$               | 462.4 / 488 |
| 15.629                    | $1.77^{+0.08}_{-0.09}$                          | —                        | $0.772^{+0.032}_{-0.042}$        | $2.799^{+0.285}_{-0.220}$       | —                                                  | $3.35^{+0.08}_{-0.09} \times 10^{-10}$               | 559.4 / 522 |
| 15.636                    | $1.52^{+0.09}_{-0.10}$                          | —                        | $0.656^{+0.036}_{-0.045}$        | $2.403^{+0.129}_{-0.111}$       | —                                                  | $3.43^{+0.07}_{-0.07} \times 10^{-10}$               | 578.7 / 553 |
| 16.557                    | $1.85^{+0.17}_{-0.19}$                          | —                        | $0.659^{+0.124}_{-0.141}$        | $1.964^{+0.505}_{-0.259}$       | —                                                  | $2.38^{+0.10}_{-0.14} \times 10^{-10}$               | 246.7 / 284 |
| 16.562                    | $1.51^{+0.08}_{-0.09}$                          | —                        | $0.744^{+0.029}_{-0.032}$        | $2.474^{+0.147}_{-0.114}$       | —                                                  | $3.39^{+0.07}_{-0.07} \times 10^{-10}$               | 618.5 / 551 |
| 17.552                    | $1.51^{+0.12}_{-0.15}$                          | —                        | $0.723^{+0.045}_{-0.051}$        | $2.427^{+0.416}_{-0.285}$       | —                                                  | $2.75^{+0.13}_{-0.11} \times 10^{-10}$               | 295.1 / 347 |
| 17.559                    | $1.48^{+0.10}_{-0.13}$                          | —                        | $0.710^{+0.044}_{-0.042}$        | $2.160^{+0.130}_{-0.130}$       | —                                                  | $1.98^{+0.05}_{-0.04} \times 10^{-10}$               | 490.6 / 467 |
| 18.681                    | $1.47^{+0.13}_{-0.15}$                          | —                        | $0.667^{+0.066}_{-0.071}$        | $2.201^{+0.416}_{-0.247}$       | —                                                  | $2.68^{+0.11}_{-0.11} \times 10^{-10}$               | 371.7 / 354 |
| 18.688                    | $1.50^{+0.09}_{-0.09}$                          | —                        | $0.618^{+0.041}_{-0.045}$        | $2.304^{+0.243}_{-0.157}$       | —                                                  | $2.28^{+0.07}_{-0.05} \times 10^{-10}$               | 414.6 / 444 |
| 19.478                    | $1.25^{+0.06}_{-0.29}$                          | —                        | $0.144^{+0.013}_{-0.009}$        | $1.600^{+0.112}_{-0.099}$       | —                                                  | $1.98^{+0.15}_{-0.14} \times 10^{-10}$               | 168.7 / 213 |
| 19.484                    | $1.40^{+0.06}_{-0.07}$                          | —                        | $0.625^{+0.036}_{-0.043}$        | $2.029^{+0.096}_{-0.085}$       | —                                                  | $2.61^{+0.05}_{-0.04} \times 10^{-10}$               | 707.0 / 528 |
| 20.605                    | $1.57^{+0.09}_{-0.13}$                          | $24.4^{+4.0}_{-1.5}$     | $0.779^{+0.042}_{-0.044}$        | $2.382^{+0.620}_{-0.379}$       | $1.24^{+0.15}_{-0.15} \times 10^{-11}$             | $2.34^{+0.09}_{-0.08} \times 10^{-10}$               | 372.5 / 368 |
| 20.613                    | $1.56^{+0.06}_{-0.08}$                          | $24.0^{+2.3}_{-0.8}$     | $0.747^{+0.033}_{-0.023}$        | $1.995^{+0.176}_{-0.137}$       | $1.11^{+0.08}_{-0.08} \times 10^{-11}$             | $2.68^{+0.05}_{-0.05} \times 10^{-10}$               | 500.6 / 510 |
| 21.734                    | $1.45^{+0.12}_{-0.13}$                          | $31.8^{+10.9}_{-4.2}$    | $0.662^{+0.050}_{-0.046}$        | $2.052^{+0.442}_{-0.254}$       | $0.67^{+0.20}_{-0.16} \times 10^{-11}$             | $2.15^{+0.09}_{-0.09} \times 10^{-10}$               | 287.7 / 312 |
| 21.741                    | $1.43^{+0.07}_{-0.07}$                          | $44.0^{+7.4}_{-2.5}$     | $0.795^{+0.044}_{-0.024}$        | $2.013^{+0.178}_{-0.155}$       | $1.14^{+0.14}_{-0.11} \times 10^{-11}$             | $2.27^{+0.04}_{-0.04} \times 10^{-10}$               | 474.3 / 473 |
| 22.533                    | $1.35^{+0.08}_{-0.09}$                          | $29.8^{+5.5}_{-2.7}$     | $0.705^{+0.058}_{-0.087}$        | $2.075^{+0.364}_{-0.214}$       | $0.68^{+0.11}_{-0.10} \times 10^{-11}$             | $2.04^{+0.03}_{-0.07} \times 10^{-10}$               | 284.6 / 314 |
| 23.126                    | $1.42^{+0.08}_{-0.08}$                          | $36.6^{+8.7}_{-3.0}$     | $0.746^{+0.040}_{-0.037}$        | $2.073^{+0.273}_{-0.219}$       | $0.84^{+0.19}_{-0.14} \times 10^{-11}$             | $2.08^{+0.05}_{-0.06} \times 10^{-10}$               | 258.5 / 304 |
| 23.66                     | $1.38^{+0.07}_{-0.08}$                          | $32.6^{+5.7}_{-2.8}$     | $0.693^{+0.034}_{-0.044}$        | $2.065^{+0.290}_{-0.206}$       | $0.88^{+0.12}_{-0.12} \times 10^{-11}$             | $2.02^{+0.06}_{-0.05} \times 10^{-10}$               | 422.4 / 389 |
| 23.666                    | $1.44^{+0.08}_{-0.11}$                          | $28.7^{+4.1}_{-1.6}$     | $0.790^{+0.034}_{-0.035}$        | $2.146^{+0.491}_{-0.328}$       | $0.99^{+0.12}_{-0.12} \times 10^{-11}$             | $2.03^{+0.04}_{-0.05} \times 10^{-10}$               | 426.1 / 378 |
| 23.999                    | $1.41^{+0.08}_{-0.08}$                          | $31.5^{+6.4}_{-2.3}$     | $0.644^{+0.045}_{-0.031}$        | $2.402^{+0.633}_{-0.329}$       | $1.03^{+0.18}_{-0.17} \times 10^{-11}$             | $2.64^{+0.07}_{-0.08} \times 10^{-10}$               | 378.7 / 401 |
| 24.788                    | $1.58^{+0.07}_{-0.07}$                          | $33.7^{+1.8}_{-1.8}$     | $0.672^{+0.036}_{-0.031}$        | $1.770^{+0.329}_{-0.237}$       | $1.10^{+0.13}_{-0.12} \times 10^{-11}$             | $1.78^{+0.05}_{-0.04} \times 10^{-10}$               | 356.7 / 364 |
| 24.796                    | $1.51^{+0.06}_{-0.06}$                          | $32.9^{+5.1}_{-2.6}$     | $0.660^{+0.040}_{-0.047}$        | $1.892^{+0.223}_{-0.165}$       | $0.85^{+0.10}_{-0.12} \times 10^{-11}$             | $1.88^{+0.04}_{-0.04} \times 10^{-10}$               | 488.6 / 417 |
| 25.12                     | $1.40^{+0.06}_{-0.07}$                          | $33.6^{+4.7}_{-2.1}$     | $0.719^{+0.029}_{-0.030}$        | $2.430^{+0.560}_{-0.316}$       | $1.54^{+0.38}_{-0.19} \times 10^{-11}$             | $1.78^{+0.06}_{-0.04} \times 10^{-10}$               | 353.1 / 385 |
| 25.128                    | $1.41^{+0.06}_{-0.08}$                          | $31.0^{+3.1}_{-1.2}$     | $0.748^{+0.041}_{-0.035}$        | $1.847^{+0.349}_{-0.248}$       | $1.29^{+0.10}_{-0.10} \times 10^{-11}$             | $1.81^{+0.04}_{-0.04} \times 10^{-10}$               | 417.5 / 399 |
| 25.908                    | $1.25^{+0.08}_{-0.09}$                          | $21.0^{+3.1}_{-1.6}$     | $0.691^{+0.030}_{-0.035}$        | $1.809^{+0.205}_{-0.155}$       | $1.66^{+0.12}_{-0.12} \times 10^{-11}$             | $1.73^{+0.05}_{-0.05} \times 10^{-10}$               | 364.4 / 350 |
| 25.913                    | $1.29^{+0.07}_{-0.09}$                          | $28.2^{+3.5}_{-1.2}$     | $0.733^{+0.037}_{-0.038}$        | $1.542^{+0.169}_{-0.133}$       | $1.47^{+0.13}_{-0.13} \times 10^{-11}$             | $1.72^{+0.04}_{-0.05} \times 10^{-10}$               | 320.5 / 348 |
| 26.303                    | $1.07^{+0.07}_{-0.11}$                          | $19.4^{+0.7}_{-0.8}$     | $0.573^{+0.046}_{-0.047}$        | $1.414^{+0.068}_{-0.054}$       | $8.70^{+0.23}_{-0.24} \times 10^{-11}$             | $1.69^{+0.04}_{-0.04} \times 10^{-10}$               | 390.7 / 361 |
| 26.309                    | $1.05^{+0.01}_{-0.04}$                          | $15.0^{+1.9}_{-0.8}$     | $0.797^{+0.035}_{-0.051}$        | $1.902^{+0.082}_{-0.104}$       | $7.94^{+0.26}_{-0.26} \times 10^{-11}$             | $1.80^{+0.05}_{-0.04} \times 10^{-10}$               | 407.3 / 342 |
| 26.714                    | $1.35^{+0.07}_{-0.08}$                          | $24.9^{+2.6}_{-1.3}$     | $0.740^{+0.029}_{-0.039}$        | $1.690^{+0.368}_{-0.258}$       | $1.83^{+0.13}_{-0.13} \times 10^{-11}$             | $1.53^{+0.04}_{-0.04} \times 10^{-10}$               | 390.8 / 322 |
| 27.307                    | $1.18^{+0.09}_{-0.11}$                          | $33.3^{+5.9}_{-2.5}$     | $0.656^{+0.054}_{-0.070}$        | $1.619^{+0.395}_{-0.224}$       | $1.62^{+0.24}_{-0.19} \times 10^{-11}$             | $1.58^{+0.06}_{-0.05} \times 10^{-10}$               | 244.3 / 286 |
| 27.314                    | $1.39^{+0.07}_{-0.10}$                          | $25.1^{+3.1}_{-1.1}$     | $0.589^{+0.040}_{-0.037}$        | $1.767^{+0.342}_{-0.256}$       | $1.30^{+0.12}_{-0.11} \times 10^{-11}$             | $1.69^{+0.05}_{-0.04} \times 10^{-10}$               | 354.3 / 354 |
| 27.907                    | $1.31^{+0.07}_{-0.08}$                          | $30.9^{+4.0}_{-1.8}$     | $0.589^{+0.051}_{-0.054}$        | $1.822^{+0.364}_{-0.228}$       | $1.31^{+0.14}_{-0.15} \times 10^{-11}$             | $1.50^{+0.05}_{-0.05} \times 10^{-10}$               | 292.0 / 317 |
| 28.036                    | $1.35^{+0.06}_{-0.07}$                          | $33.4^{+1.8}_{-1.8}$     | $0.637^{+0.042}_{-0.036}$        | $1.937^{+0.391}_{-0.267}$       | $1.37^{+0.15}_{-0.13} \times 10^{-11}$             | $1.44^{+0.05}_{-0.04} \times 10^{-10}$               | 333.9 / 338 |
| 28.043                    | $1.27^{+0.09}_{-0.12}$                          | $31.7^{+7.8}_{-2.4}$     | $0.597^{+0.104}_{-0.066}$        | $1.627^{+0.468}_{-0.285}$       | $0.95^{+0.15}_{-0.16} \times 10^{-11}$             | $1.44^{+0.06}_{-0.05} \times 10^{-10}$               | 271.6 / 320 |
| 28.908                    | $1.09^{+0.08}_{-0.09}$                          | $28.5^{+3.9}_{-1.9}$     | $0.632^{+0.034}_{-0.035}$        | $1.601^{+0.153}_{-0.121}$       | $1.42^{+0.14}_{-0.12} \times 10^{-11}$             | $1.41^{+0.03}_{-0.04} \times 10^{-10}$               | 321.9 / 331 |
| 29.162                    | $1.31^{+0.06}_{-0.10}$                          | $26.4^{+3.1}_{-1.0}$     | $0.635^{+0.044}_{-0.040}$        | $1.999^{+0.559}_{-0.307}$       | $1.89^{+0.15}_{-0.14} \times 10^{-11}$             | $1.44^{+0.04}_{-0.04} \times 10^{-10}$               | 296.8 / 311 |
| 29.169                    | $1.33^{+0.08}_{-0.08}$                          | $25.2^{+2.7}_{-1.3}$     | $0.586^{+0.037}_{-0.038}$        | $1.728^{+0.339}_{-0.186}$       | $2.05^{+0.16}_{-0.16} \times 10^{-11}$             | $1.62^{+0.05}_{-0.04} \times 10^{-10}$               | 287.8 / 317 |
| 29.693                    | $1.32^{+0.07}_{-0.08}$                          | $28.4^{+4.1}_{-1.7}$     | $0.600^{+0.058}_{-0.040}$        | $1.389^{+0.369}_{-0.210}$       | $1.13^{+0.13}_{-0.13} \times 10^{-11}$             | $1.31^{+0.03}_{-0.04} \times 10^{-10}$               | 347.8 / 305 |
| 29.699                    | $1.06^{+0.09}_{-0.14}$                          | $31.9^{+5.8}_{-2.0}$     | $0.660^{+0.049}_{-0.048}$        | $1.558^{+0.223}_{-0.154}$       | $1.24^{+0.15}_{-0.15} \times 10^{-11}$             | $1.31^{+0.04}_{-0.04} \times 10^{-10}$               | 275.1 / 279 |
| 30.288                    | $0.64^{+0.06}_{-0.05}$                          | $27.6^{+2.4}_{-1.2}$     | $0.786^{+0.042}_{-0.052}$        | $1.522^{+0.081}_{-0.080}$       | $1.86^{+0.03}_{-0.03} \times 10^{-10}$             | $1.34^{+0.03}_{-0.03} \times 10^{-10}$               | 373.0 / 333 |
| 30.296                    | $0.53^{+0.07}_{-0.09}$                          | $30.1^{+4.5}_{-1.7}$     | $0.713^{+0.145}_{-0.106}$        | $1.415^{+0.149}_{-0.073}$       | $1.71^{+0.05}_{-0.04} \times 10^{-10}$             | $1.17^{+0.05}_{-0.04} \times 10^{-10}$               | 317.8 / 270 |
| 30.749                    | $0.67^{+0.13}_{-0.19}$                          | $25.5^{+7.7}_{-3.0}$     | $0.714^{+0.068}_{-0.075}$        | $1.424^{+0.149}_{-0.110}$       | $6.91^{+0.36}_{-0.36} \times 10^{-11}$             | $1.24^{+0.06}_{-0.05} \times 10^{-10}$               | 247.1 / 242 |
| 30.754                    | $1.00^{+0.10}_{-0.10}$                          | $22.9^{+2.3}_{-1.3}$     | $0.643^{+0.041}_{-0.044}$        | $1.332^{+0.060}_{-0.062}$       | $5.83^{+0.18}_{-0.18} \times 10^{-11}$             | $1.27^{+0.03}_{-0.03} \times 10^{-10}$               | 345.0 / 310 |
| 30.815                    | $1.38^{+0.14}_{-0.09}$                          | $26.0^{+3.2}_{-2.0}$     | $0.596^{+0.057}_{-0.070}$        | $1.346^{+0.117}_{-0.125}$       | $2.67^{+0.20}_{-0.20} \times 10^{-11}$             | $1.32^{+0.05}_{-0.05} \times 10^{-10}$               | 294.3 / 270 |
| 30.82                     | $1.27^{+0.08}_{-0.12}$                          | $26.2^{+3.5}_{-1.3}$     | $0.580^{+0.087}_{-0.077}$        | $1.060^{+0.130}_{-0.098}$       | $1.91^{+0.17}_{-0.16} \times 10^{-11}$             | $1.09^{+0.04}_{-0.04} \times 10^{-10}$               | 278.6 / 279 |
| 31.75                     | $0.98^{+0.17}_{-0.22}$                          | $25.2^{+3.9}_{-1.7}$     | $0.613^{+0.054}_{-0.058}$        | $1.478^{+0.205}_{-0.138}$       | $5.62^{+0.31}_{-0.35} \times 10^{-11}$             | $1.30^{+0.05}_{-0.05} \times 10^{-10}$               | 221.2 / 237 |
| 31.813                    | $0.80^{+0.13}_{-0.10}$                          | $24.3^{+4.3}_{-2.4}$     | $0.643^{+0.066}_{-0.073}$        | $1.413^{+0.100}_{-0.099}$       | $9.71^{+0.39}_{-0.39} \times 10^{-11}$             | $1.24^{+0.06}_{-0.06} \times 10^{-10}$               | 221.1 / 241 |
| 31.817                    | $0.41^{+0.12}_{-0.10}$                          | $31.6^{+7.1}_{-3.4}$     | $0.714^{+0.070}_{-0.073}$        | $1.567^{+0.110}_{-0.093}$       | $1.11^{+0.04}_{-0.05} \times 10^{-10}$             | $1.33^{+0.06}_{-0.05} \times 10^{-10}$               | 299.3 / 248 |
| 32.088                    | $0.55^{+0.09}_{-0.06}$                          | $29.5^{+4.1}_{-2.4}$     | $0.740^{+0.061}_{-0.065}$        | $1.581^{+0.196}_{-0.157}$       | $2.45^{+0.07}_{-0.07} \times 10^{-10}$             | $1.14^{+0.07}_{-0.06} \times 10^{-10}$               | 208.2 / 215 |
| 32.09                     | $0.74^{+0.14}_{-0.07}$                          | $30.7^{+4.3}_{-2.7}$     | $0.847^{+0.065}_{-0.237}$        | $1.347^{+0.545}_{-0.295}$       | $3.02^{+0.08}_{-0.08} \times 10^{-10}$             | $1.62^{+0.07}_{-0.07} \times 10^{-10}$               | 269.3 / 240 |
| 32.74                     | $0.57^{+0.14}_{-0.26}$                          | $21.1^{+7.0}_{-2.4}$     | $0.150^{+0.022}_{-0.150}$        | $1.376^{+0.099}_{-0.976}$       | $2.49^{+0.37}_{-0.37} \times 10^{-11}$             | $1.24^{+0.09}_{-0.09} \times 10^{-10}$               | 155.8 / 181 |
| 32.744                    | $1.17^{+0.10}_{-0.09}$                          | $24.0^{+2.7}_{-1.4}$     | $0.555^{+0.049}_{-0.050}$        | $1.330^{+0.376}_{-0.141}$       | $3.81^{+0.21}_{-0.20} \times 10^{-11}$             | $1.26^{+0.09}_{-0.04} \times 10^{-10}$               | 331.4 / 286 |
| 32.878                    | $1.17^{+0.09}_{-0.08}$                          | $23.5^{+2.4}_{-1.2}$     | $0.564^{+0.046}_{-0.047}$        | $1.345^{+0.207}_{-0.120}$       | $3.05^{+0.16}_{-0.15} \times 10^{-11}$             | $1.12^{+0.03}_{-0.04} \times 10^{-10}$               | 170.5 / 193 |

Continued on next page

Table 1 – continued from previous page

| $T_{\text{mid}}$<br>(day) | $N_{\text{H}}$<br>( $10^{22} \text{ cm}^{-2}$ ) | $kT_{\text{BB}}$<br>(eV) | APEC $kT_{\text{cool}}$<br>(keV) | APEC $kT_{\text{hot}}$<br>(keV) | BB Flux<br>( $\text{erg cm}^{-2} \text{ s}^{-1}$ ) | APEC Flux<br>( $\text{erg cm}^{-2} \text{ s}^{-1}$ ) | Cstat/dof   |
|---------------------------|-------------------------------------------------|--------------------------|----------------------------------|---------------------------------|----------------------------------------------------|------------------------------------------------------|-------------|
| 33.482                    | $0.69^{+0.09}_{-0.10}$                          | $30.2^{+4.8}_{-1.8}$     | $0.644^{+0.051}_{-0.055}$        | $1.291^{+0.077}_{-0.065}$       | $7.92^{+0.25}_{-0.25} \times 10^{-11}$             | $1.11^{+0.03}_{-0.03} \times 10^{-10}$               | 304.5 / 277 |
| 33.551                    | $0.89^{+0.08}_{-0.11}$                          | $25.2^{+3.2}_{-1.2}$     | $0.598^{+0.048}_{-0.044}$        | $1.331^{+0.117}_{-0.095}$       | $6.06^{+0.21}_{-0.21} \times 10^{-11}$             | $1.00^{+0.03}_{-0.03} \times 10^{-10}$               | 303.4 / 271 |
| 33.621                    | $0.94^{+0.10}_{-0.09}$                          | $26.5^{+3.1}_{-1.6}$     | $0.554^{+0.044}_{-0.049}$        | $1.402^{+0.230}_{-0.132}$       | $4.63^{+0.18}_{-0.19} \times 10^{-11}$             | $1.00^{+0.04}_{-0.03} \times 10^{-10}$               | 304.8 / 281 |
| 33.69                     | $0.77^{+0.11}_{-0.18}$                          | $21.9^{+6.1}_{-3.2}$     | $0.557^{+0.078}_{-0.092}$        | $1.306^{+0.309}_{-0.209}$       | $3.57^{+0.30}_{-0.29} \times 10^{-11}$             | $9.96^{+0.61}_{-0.52} \times 10^{-11}$               | 166.1 / 203 |
| 33.758                    | $0.27^{+0.06}_{-0.07}$                          | $31.1^{+7.9}_{-4.1}$     | $0.660^{+0.051}_{-0.063}$        | $1.539^{+0.076}_{-0.069}$       | $5.57^{+0.22}_{-0.22} \times 10^{-11}$             | $1.09^{+0.03}_{-0.03} \times 10^{-10}$               | 334.2 / 274 |
| 33.825                    | $0.37^{+0.07}_{-0.11}$                          | $32.4^{+5.2}_{-2.6}$     | $0.659^{+0.041}_{-0.043}$        | $1.633^{+0.092}_{-0.066}$       | $5.48^{+0.24}_{-0.23} \times 10^{-11}$             | $1.09^{+0.04}_{-0.03} \times 10^{-10}$               | 291.9 / 272 |
| 33.891                    | $0.28^{+0.11}_{-0.09}$                          | $39.2^{+15.4}_{-5.2}$    | $0.574^{+0.099}_{-0.103}$        | $1.529^{+0.099}_{-0.080}$       | $5.95^{+0.41}_{-0.39} \times 10^{-11}$             | $1.07^{+0.05}_{-0.06} \times 10^{-10}$               | 229.3 / 221 |
| 33.955                    | $0.80^{+0.09}_{-0.11}$                          | $24.6^{+3.8}_{-1.5}$     | $0.604^{+0.044}_{-0.043}$        | $1.422^{+0.100}_{-0.082}$       | $5.76^{+0.20}_{-0.20} \times 10^{-11}$             | $1.01^{+0.03}_{-0.03} \times 10^{-10}$               | 330.6 / 282 |
| 34.018                    | $1.07^{+0.08}_{-0.08}$                          | $23.8^{+2.2}_{-1.1}$     | $0.675^{+0.040}_{-0.040}$        | $1.278^{+0.229}_{-0.146}$       | $6.15^{+0.20}_{-0.19} \times 10^{-11}$             | $9.84^{+0.26}_{-0.27} \times 10^{-11}$               | 315.6 / 279 |
| 34.08                     | $0.91^{+0.10}_{-0.11}$                          | $27.2^{+3.6}_{-1.5}$     | $0.647^{+0.036}_{-0.037}$        | $1.337^{+0.088}_{-0.080}$       | $7.02^{+0.21}_{-0.22} \times 10^{-11}$             | $1.01^{+0.03}_{-0.03} \times 10^{-10}$               | 330.7 / 270 |
| 34.143                    | $0.93^{+0.08}_{-0.12}$                          | $25.7^{+3.1}_{-1.2}$     | $0.657^{+0.035}_{-0.045}$        | $1.566^{+0.284}_{-0.194}$       | $7.59^{+0.23}_{-0.25} \times 10^{-11}$             | $1.05^{+0.03}_{-0.04} \times 10^{-10}$               | 374.3 / 273 |
| 34.156                    | $0.43^{+0.09}_{-0.10}$                          | $36.4^{+6.3}_{-2.7}$     | $0.737^{+0.063}_{-0.046}$        | $1.456^{+0.092}_{-0.057}$       | $8.18^{+0.26}_{-0.25} \times 10^{-11}$             | $9.50^{+0.23}_{-0.24} \times 10^{-11}$               | 348.9 / 278 |
| 34.223                    | $1.21^{+0.07}_{-0.09}$                          | $23.7^{+2.0}_{-0.8}$     | $0.631^{+0.048}_{-0.043}$        | $1.691^{+0.687}_{-0.432}$       | $8.12^{+0.22}_{-0.23} \times 10^{-11}$             | $1.06^{+0.03}_{-0.04} \times 10^{-10}$               | 344.1 / 294 |
| 34.29                     | $0.69^{+0.13}_{-0.08}$                          | $30.5^{+4.7}_{-2.7}$     | $0.658^{+0.049}_{-0.050}$        | $1.415^{+0.076}_{-0.072}$       | $8.86^{+0.28}_{-0.28} \times 10^{-11}$             | $1.07^{+0.03}_{-0.04} \times 10^{-10}$               | 278.0 / 264 |
| 34.409                    | $1.10^{+0.12}_{-0.15}$                          | $22.9^{+3.7}_{-1.5}$     | $0.535^{+0.067}_{-0.066}$        | $1.319^{+0.333}_{-0.235}$       | $6.12^{+0.30}_{-0.29} \times 10^{-11}$             | $8.09^{+0.39}_{-0.39} \times 10^{-11}$               | 266.2 / 221 |
| 36.873                    | $0.30^{+0.06}_{-0.05}$                          | $33.4^{+4.4}_{-2.2}$     | $0.687^{+0.038}_{-0.040}$        | $1.520^{+0.059}_{-0.062}$       | $7.59^{+0.19}_{-0.20} \times 10^{-11}$             | $8.85^{+0.21}_{-0.22} \times 10^{-11}$               | 383.6 / 280 |
| 36.939                    | $0.84^{+0.06}_{-0.09}$                          | $24.5^{+2.5}_{-0.9}$     | $0.624^{+0.035}_{-0.033}$        | $1.330^{+0.131}_{-0.106}$       | $1.01^{+0.02}_{-0.02} \times 10^{-10}$             | $9.06^{+0.25}_{-0.24} \times 10^{-11}$               | 367.5 / 267 |
| 37.206                    | $0.74^{+0.08}_{-0.05}$                          | $28.4^{+2.5}_{-1.4}$     | $0.618^{+0.030}_{-0.032}$        | $1.356^{+0.116}_{-0.088}$       | $1.02^{+0.02}_{-0.02} \times 10^{-10}$             | $8.53^{+0.20}_{-0.19} \times 10^{-11}$               | 481.7 / 285 |
| 37.722                    | $0.38^{+0.03}_{-0.03}$                          | $29.4^{+2.0}_{-1.0}$     | $0.626^{+0.049}_{-0.049}$        | $1.492^{+0.065}_{-0.061}$       | $2.81^{+0.04}_{-0.04} \times 10^{-10}$             | $8.96^{+0.23}_{-0.22} \times 10^{-11}$               | 328.1 / 297 |
| 37.924                    | $0.39^{+0.04}_{-0.05}$                          | $32.5^{+3.1}_{-1.2}$     | $0.589^{+0.061}_{-0.044}$        | $1.356^{+0.055}_{-0.041}$       | $1.37^{+0.03}_{-0.02} \times 10^{-10}$             | $8.79^{+0.21}_{-0.20} \times 10^{-11}$               | 449.2 / 283 |
| 38.197                    | $0.43^{+0.03}_{-0.04}$                          | $32.2^{+2.2}_{-0.9}$     | $0.706^{+0.040}_{-0.039}$        | $1.525^{+0.089}_{-0.079}$       | $2.08^{+0.03}_{-0.03} \times 10^{-10}$             | $8.56^{+0.21}_{-0.22} \times 10^{-11}$               | 380.4 / 293 |
| 38.789                    | $0.41^{+0.05}_{-0.06}$                          | $40.4^{+4.7}_{-2.0}$     | $0.613^{+0.098}_{-0.088}$        | $1.427^{+0.078}_{-0.069}$       | $1.74^{+0.04}_{-0.04} \times 10^{-10}$             | $7.32^{+0.29}_{-0.29} \times 10^{-11}$               | 299.1 / 249 |
| 39.048                    | $0.35^{+0.03}_{-0.05}$                          | $40.2^{+3.9}_{-1.4}$     | $0.750^{+0.046}_{-0.042}$        | $1.520^{+0.091}_{-0.077}$       | $1.32^{+0.02}_{-0.03} \times 10^{-10}$             | $8.09^{+0.20}_{-0.20} \times 10^{-11}$               | 424.6 / 279 |
| 39.313                    | $0.45^{+0.06}_{-0.06}$                          | $38.0^{+4.2}_{-1.9}$     | $0.698^{+0.062}_{-0.061}$        | $1.353^{+0.070}_{-0.063}$       | $1.34^{+0.03}_{-0.03} \times 10^{-10}$             | $8.05^{+0.22}_{-0.22} \times 10^{-11}$               | 408.9 / 275 |
| 39.648                    | $0.81^{+0.02}_{-0.03}$                          | $26.4^{+0.9}_{-0.4}$     | $0.613^{+0.094}_{-0.080}$        | $1.022^{+0.059}_{-0.046}$       | $9.40^{+0.07}_{-0.07} \times 10^{-10}$             | $7.73^{+0.21}_{-0.20} \times 10^{-11}$               | 560.9 / 250 |
| 40.186                    | $0.29^{+0.02}_{-0.03}$                          | $34.9^{+2.3}_{-0.9}$     | $0.696^{+0.050}_{-0.046}$        | $1.546^{+0.133}_{-0.097}$       | $3.78^{+0.05}_{-0.05} \times 10^{-10}$             | $7.41^{+0.28}_{-0.26} \times 10^{-11}$               | 279.6 / 239 |
| 40.582                    | $0.48^{+0.02}_{-0.02}$                          | $32.5^{+1.3}_{-0.6}$     | $0.663^{+0.045}_{-0.043}$        | $1.393^{+0.083}_{-0.068}$       | $6.35^{+0.05}_{-0.06} \times 10^{-10}$             | $7.22^{+0.22}_{-0.22} \times 10^{-11}$               | 378.6 / 252 |
| 40.843                    | $0.80^{+0.03}_{-0.04}$                          | $32.4^{+1.6}_{-0.7}$     | $0.733^{+0.061}_{-0.075}$        | $1.217^{+0.387}_{-0.226}$       | $8.10^{+0.09}_{-0.08} \times 10^{-10}$             | $6.40^{+0.30}_{-0.26} \times 10^{-11}$               | 363.0 / 223 |
| 41.437                    | $0.60^{+0.02}_{-0.02}$                          | $34.3^{+0.9}_{-0.5}$     | $0.687^{+0.069}_{-0.064}$        | $1.200^{+0.081}_{-0.069}$       | $1.33^{+0.01}_{-0.01} \times 10^{-9}$              | $7.32^{+0.22}_{-0.23} \times 10^{-11}$               | 509.8 / 255 |
| 41.639                    | $0.57^{+0.01}_{-0.02}$                          | $33.5^{+0.9}_{-0.3}$     | $0.640^{+0.055}_{-0.053}$        | $1.208^{+0.065}_{-0.066}$       | $1.31^{+0.01}_{-0.01} \times 10^{-9}$              | $7.19^{+0.20}_{-0.20} \times 10^{-11}$               | 351.7 / 261 |
| 41.973                    | $0.55^{+0.01}_{-0.01}$                          | $34.4^{+0.4}_{-1.1}$     | $0.695^{+0.062}_{-0.118}$        | $1.150^{+0.041}_{-0.048}$       | $1.27^{+0.01}_{-0.01} \times 10^{-9}$              | $7.00^{+0.20}_{-0.22} \times 10^{-11}$               | 508.3 / 255 |
| 42.436                    | $0.41^{+0.01}_{-0.02}$                          | $36.8^{+1.1}_{-0.4}$     | $0.502^{+0.136}_{-0.072}$        | $1.182^{+0.074}_{-0.061}$       | $1.47^{+0.01}_{-0.01} \times 10^{-9}$              | $6.15^{+0.30}_{-0.32} \times 10^{-11}$               | 222.8 / 232 |
| 42.569                    | $0.57^{+0.03}_{-0.03}$                          | $32.9^{+1.0}_{-1.0}$     | $0.544^{+0.091}_{-0.073}$        | $1.253^{+0.112}_{-0.087}$       | $5.79^{+0.09}_{-0.07} \times 10^{-10}$             | $5.53^{+0.29}_{-0.28} \times 10^{-11}$               | 249.5 / 207 |
| 42.902                    | $0.85^{+0.02}_{-0.02}$                          | $29.8^{+0.9}_{-0.4}$     | $0.641^{+0.053}_{-0.056}$        | $1.085^{+0.123}_{-0.103}$       | $1.07^{+0.01}_{-0.01} \times 10^{-9}$              | $6.66^{+0.20}_{-0.18} \times 10^{-11}$               | 495.8 / 256 |
| 43.249                    | $0.52^{+0.02}_{-0.02}$                          | $34.9^{+1.1}_{-0.5}$     | $0.630^{+0.102}_{-0.084}$        | $1.156^{+0.086}_{-0.069}$       | $1.13^{+0.01}_{-0.01} \times 10^{-9}$              | $6.55^{+0.23}_{-0.23} \times 10^{-11}$               | 360.8 / 241 |
| 43.627                    | $0.22^{+0.02}_{-0.02}$                          | $47.4^{+2.6}_{-1.3}$     | $0.590^{+0.196}_{-0.094}$        | $1.430^{+0.072}_{-0.057}$       | $4.49^{+0.06}_{-0.05} \times 10^{-10}$             | $5.99^{+0.31}_{-0.30} \times 10^{-11}$               | 295.8 / 247 |
| 43.83                     | $0.26^{+0.01}_{-0.02}$                          | $42.8^{+1.6}_{-0.7}$     | $0.543^{+0.061}_{-0.066}$        | $1.475^{+0.095}_{-0.075}$       | $7.74^{+0.07}_{-0.06} \times 10^{-10}$             | $6.28^{+0.30}_{-0.29} \times 10^{-11}$               | 296.3 / 238 |
| 44.491                    | $0.47^{+0.01}_{-0.01}$                          | $38.0^{+0.9}_{-0.4}$     | $0.699^{+0.109}_{-0.113}$        | $1.286^{+0.075}_{-0.073}$       | $2.24^{+0.01}_{-0.02} \times 10^{-9}$              | $5.86^{+0.27}_{-0.27} \times 10^{-11}$               | 360.9 / 240 |
| 45.493                    | $0.76^{+0.02}_{-0.02}$                          | $32.5^{+0.8}_{-0.4}$     | $0.478^{+0.053}_{-0.064}$        | $1.174^{+0.218}_{-0.164}$       | $2.40^{+0.02}_{-0.02} \times 10^{-9}$              | $6.81^{+0.27}_{-0.27} \times 10^{-11}$               | 421.2 / 213 |
| 45.835                    | $0.67^{+0.02}_{-0.02}$                          | $35.9^{+1.0}_{-0.4}$     | $0.553^{+0.070}_{-0.073}$        | $1.150^{+0.164}_{-0.114}$       | $2.41^{+0.01}_{-0.02} \times 10^{-9}$              | $6.46^{+0.37}_{-0.15} \times 10^{-11}$               | 349.8 / 193 |
| 46.164                    | $0.77^{+0.01}_{-0.02}$                          | $33.6^{+0.9}_{-0.4}$     | $0.580^{+0.041}_{-0.055}$        | —                               | $2.29^{+0.02}_{-0.01} \times 10^{-9}$              | $6.96^{+0.32}_{-0.33} \times 10^{-11}$               | 403.5 / 200 |
| 46.485                    | $0.39^{+0.01}_{-0.02}$                          | $40.2^{+0.7}_{-0.3}$     | $0.506^{+0.106}_{-0.096}$        | $1.234^{+0.079}_{-0.057}$       | $2.00^{+0.01}_{-0.02} \times 10^{-9}$              | $5.50^{+0.34}_{-0.29} \times 10^{-11}$               | 312.3 / 196 |
| 46.812                    | $0.72^{+0.03}_{-0.01}$                          | $35.5^{+0.9}_{-0.6}$     | $0.486^{+0.057}_{-0.049}$        | $1.637^{+0.433}_{-0.247}$       | $2.03^{+0.02}_{-0.01} \times 10^{-9}$              | $6.89^{+0.44}_{-0.39} \times 10^{-11}$               | 325.4 / 185 |
| 47.159                    | $0.72^{+0.02}_{-0.02}$                          | $36.0^{+1.0}_{-0.5}$     | $0.459^{+0.071}_{-0.075}$        | $1.221^{+0.153}_{-0.116}$       | $2.70^{+0.02}_{-0.02} \times 10^{-9}$              | $7.34^{+0.44}_{-0.40} \times 10^{-11}$               | 274.7 / 202 |
| 47.824                    | $0.61^{+0.02}_{-0.02}$                          | $36.9^{+0.9}_{-0.5}$     | $0.513^{+0.075}_{-0.078}$        | $1.179^{+0.320}_{-0.178}$       | $2.39^{+0.01}_{-0.02} \times 10^{-9}$              | $5.57^{+0.42}_{-0.35} \times 10^{-11}$               | 320.3 / 194 |
| 48.155                    | $0.57^{+0.01}_{-0.02}$                          | $37.8^{+1.0}_{-0.4}$     | $0.504^{+0.048}_{-0.058}$        | $1.366^{+0.194}_{-0.157}$       | $2.67^{+0.02}_{-0.01} \times 10^{-9}$              | $5.72^{+0.30}_{-0.35} \times 10^{-11}$               | 281.8 / 189 |
| 48.479                    | $0.41^{+0.02}_{-0.01}$                          | $39.6^{+1.1}_{-0.6}$     | $0.515^{+0.173}_{-0.109}$        | $1.145^{+0.064}_{-0.064}$       | $2.10^{+0.02}_{-0.01} \times 10^{-9}$              | $5.38^{+0.50}_{-0.26} \times 10^{-11}$               | 238.9 / 189 |
| 48.819                    | $0.58^{+0.02}_{-0.02}$                          | $34.9^{+1.0}_{-0.5}$     | $0.546^{+0.041}_{-0.052}$        | $1.223^{+0.173}_{-0.111}$       | $1.20^{+0.01}_{-0.01} \times 10^{-9}$              | $5.83^{+0.23}_{-0.23} \times 10^{-11}$               | 353.0 / 223 |
| 49.15                     | $0.35^{+0.01}_{-0.01}$                          | $39.1^{+1.1}_{-0.6}$     | $0.555^{+0.058}_{-0.051}$        | $1.244^{+0.087}_{-0.071}$       | $1.20^{+0.01}_{-0.01} \times 10^{-9}$              | $5.95^{+0.25}_{-0.25} \times 10^{-11}$               | 308.2 / 226 |
| 49.467                    | $0.70^{+0.02}_{-0.02}$                          | $33.0^{+0.8}_{-0.4}$     | $0.465^{+0.066}_{-0.071}$        | $0.862^{+0.112}_{-0.102}$       | $1.62^{+0.01}_{-0.01} \times 10^{-9}$              | $6.14^{+0.20}_{-0.20} \times 10^{-11}$               | 384.4 / 220 |
| 49.799                    | $0.75^{+0.02}_{-0.02}$                          | $34.1^{+0.8}_{-0.4}$     | $0.242^{+0.035}_{-0.242}$        | $0.579^{+0.034}_{-0.030}$       | $1.43^{+0.01}_{-0.01} \times 10^{-9}$              | $7.96^{+0.32}_{-0.23} \times 10^{-11}$               | 450.3 / 219 |
| 50.145                    | $0.58^{+0.01}_{-0.01}$                          | $35.8^{+0.8}_{-0.4}$     | $0.455^{+0.048}_{-0.050}$        | $1.021^{+0.098}_{-0.070}$       | $1.68^{+0.01}_{-0.01} \times 10^{-9}$              | $5.70^{+0.22}_{-0.19} \times 10^{-11}$               | 312.5 / 226 |
| 50.464                    | $0.52^{+0.03}_{-0.03}$                          | $35.3^{+1.5}_{-1.0}$     | $0.698^{+0.234}_{-0.252}$        | $1.140^{+0.207}_{-0.108}$       | $9.73^{+0.12}_{-0.12} \times 10^{-10}$             | $4.49^{+0.34}_{-0.34} \times 10^{-11}$               | 177.2 / 166 |
| 50.802                    | $0.46^{+0.02}_{-0.02}$                          | $36.9^{+1.6}_{-1.0}$     | $0.150^{+0.15}_{-0.150}$         | $0.586^{+0.025}_{-0.040}$       | $6.22^{+0.09}_{-0.11} \times 10^{-10}$             | $5.41^{+0.29}_{-0.37} \times 10^{-11}$               | 172.6 / 174 |
| 51.14                     | $0.45^{+0.03}_{-0.02}$                          | $38.6^{+2.4}_{-1.1}$     | $0.125^{+0.000}_{-0.125}$        | $0.726^{+0.051}_{-0.025}$       | $6.58^{+0.14}_{-0.14} \times 10^{-10}$             | $9.86^{+1.34}_{-1.30} \times 10^{-11}$               | 216.8 / 177 |
| 51.541                    | $0.72^{+0.02}_{-0.02}$                          | $32.0^{+0.5}_{-0.5}$     | $0.125^{+0.125}_{-0.125}$        | $0.591^{+0.029}_{-0.029}$       | $1.06^{+0.01}_{-0.01} \times 10^{-9}$              | $5.66^{+0.30}_{-0.34} \times 10^{-11}$               | 453.1 / 228 |
| 52.529                    | $0.28^{+0.04}_{-0.02}$                          | $40.5^{+2.7}_{-1.9}$     | $0.470^{+0.153}_{-0.132}$        | $1.345^{+0.226}_{-0.154}$       | $6.25^{+0.11}_{-0.14} \times 10^{-10}$             | $3.12^{+0.36}_{-0.34} \times 10^{-11}$               | 123.9 / 146 |

Continued on next page

Table 1 – continued from previous page

| $T_{\text{mid}}$<br>(day) | $N_{\text{H}}$<br>( $10^{22} \text{ cm}^{-2}$ ) | $kT_{\text{BB}}$<br>(eV) | APEC $kT_{\text{cool}}$<br>(keV) | APEC $kT_{\text{hot}}$<br>(keV) | BB Flux<br>( $\text{erg cm}^{-2} \text{ s}^{-1}$ ) | APEC Flux<br>( $\text{erg cm}^{-2} \text{ s}^{-1}$ ) | Cstat/dof   |
|---------------------------|-------------------------------------------------|--------------------------|----------------------------------|---------------------------------|----------------------------------------------------|------------------------------------------------------|-------------|
| 52.662                    | $0.33^{+0.04}_{-0.03}$                          | $40.1^{+2.2}_{-0.8}$     | $0.518^{+0.129}_{-0.136}$        | $1.293^{+0.222}_{-0.135}$       | $6.28^{+0.11}_{-0.11} \times 10^{-10}$             | $4.03^{+0.44}_{-0.35} \times 10^{-11}$               | 162.8 / 155 |
| 52.794                    | $0.22^{+0.04}_{-0.04}$                          | $45.5^{+4.6}_{-2.3}$     | $0.686^{+0.198}_{-0.191}$        | $1.464^{+0.371}_{-0.186}$       | $5.02^{+0.12}_{-0.12} \times 10^{-10}$             | $4.08^{+0.52}_{-0.46} \times 10^{-11}$               | 110.4 / 142 |
| 52.735                    | $0.39^{+0.02}_{-0.03}$                          | $40.1^{+2.0}_{-1.0}$     | $0.529^{+0.060}_{-0.059}$        | $1.429^{+0.130}_{-0.118}$       | $5.38^{+0.07}_{-0.06} \times 10^{-10}$             | $4.82^{+0.24}_{-0.23} \times 10^{-11}$               | 250.2 / 215 |
| 52.918                    | $0.65^{+0.03}_{-0.03}$                          | $33.5^{+1.4}_{-0.6}$     | $0.565^{+0.061}_{-0.066}$        | $2.745^{+2.74}_{-1.276}$        | $6.87^{+0.07}_{-0.06} \times 10^{-10}$             | $5.03^{+0.32}_{-0.28} \times 10^{-11}$               | 247.7 / 204 |
| 54.593                    | $0.58^{+0.01}_{-0.01}$                          | $36.6^{+0.7}_{-0.4}$     | $0.557^{+0.033}_{-0.033}$        | $1.153^{+0.124}_{-0.095}$       | $1.01^{+0.01}_{-0.00} \times 10^{-9}$              | $4.48^{+0.13}_{-0.12} \times 10^{-11}$               | 624.3 / 238 |
| 55.575                    | $0.54^{+0.01}_{-0.01}$                          | $36.3^{+0.7}_{-0.3}$     | $0.485^{+0.068}_{-0.063}$        | $1.124^{+0.116}_{-0.080}$       | $1.71^{+0.01}_{-0.01} \times 10^{-9}$              | $4.96^{+0.12}_{-0.18} \times 10^{-11}$               | 424.2 / 215 |
| 55.656                    | $0.77^{+0.03}_{-0.01}$                          | $33.3^{+0.8}_{-0.6}$     | $0.349^{+0.036}_{-0.045}$        | $1.569^{+0.475}_{-0.256}$       | $1.52^{+0.01}_{-0.01} \times 10^{-9}$              | $5.19^{+0.20}_{-0.20} \times 10^{-11}$               | 598.0 / 211 |
| 56.651                    | $0.67^{+0.01}_{-0.01}$                          | $35.1^{+0.6}_{-0.3}$     | $0.445^{+0.030}_{-0.027}$        | $1.365^{+0.262}_{-0.146}$       | $1.52^{+0.01}_{-0.01} \times 10^{-9}$              | $4.91^{+0.14}_{-0.15} \times 10^{-11}$               | 545.6 / 219 |
| 57.515                    | $0.55^{+0.01}_{-0.01}$                          | $35.2^{+0.7}_{-0.4}$     | $0.473^{+0.052}_{-0.047}$        | $1.164^{+0.091}_{-0.072}$       | $1.42^{+0.01}_{-0.00} \times 10^{-9}$              | $4.31^{+0.17}_{-0.15} \times 10^{-11}$               | 440.6 / 220 |
| 58.561                    | $0.53^{+0.01}_{-0.01}$                          | $37.9^{+0.9}_{-0.5}$     | $0.515^{+0.032}_{-0.044}$        | $1.247^{+0.230}_{-0.134}$       | $9.24^{+0.05}_{-0.06} \times 10^{-10}$             | $4.01^{+0.19}_{-0.18} \times 10^{-11}$               | 294.9 / 213 |
| 60.831                    | $0.41^{+0.01}_{-0.01}$                          | $37.4^{+0.8}_{-0.4}$     | $0.576^{+0.062}_{-0.053}$        | $1.188^{+0.069}_{-0.062}$       | $8.59^{+0.05}_{-0.05} \times 10^{-10}$             | $2.95^{+0.11}_{-0.11} \times 10^{-11}$               | 381.0 / 228 |
| 61.563                    | $0.49^{+0.01}_{-0.01}$                          | $35.2^{+0.9}_{-0.4}$     | $0.537^{+0.063}_{-0.065}$        | $1.004^{+0.078}_{-0.073}$       | $8.89^{+0.05}_{-0.05} \times 10^{-10}$             | $2.77^{+0.11}_{-0.14} \times 10^{-11}$               | 285.8 / 211 |
| 63.886                    | $0.06^{+0.01}_{-0.02}$                          | $50.3^{+2.9}_{-1.4}$     | $0.513^{+0.096}_{-0.078}$        | $1.379^{+0.114}_{-0.091}$       | $2.97^{+0.04}_{-0.04} \times 10^{-10}$             | $2.43^{+0.19}_{-0.19} \times 10^{-11}$               | 243.6 / 190 |
| 64.614                    | $0.23^{+0.01}_{-0.02}$                          | $45.2^{+2.2}_{-0.8}$     | $0.484^{+0.069}_{-0.055}$        | $1.284^{+0.073}_{-0.059}$       | $2.31^{+0.03}_{-0.02} \times 10^{-10}$             | $2.53^{+0.22}_{-0.16} \times 10^{-11}$               | 260.4 / 220 |
| 65.545                    | $0.18^{+0.02}_{-0.02}$                          | $49.3^{+3.3}_{-1.6}$     | $0.538^{+0.091}_{-0.094}$        | $1.224^{+0.073}_{-0.062}$       | $1.88^{+0.03}_{-0.03} \times 10^{-10}$             | $2.41^{+0.16}_{-0.14} \times 10^{-11}$               | 233.3 / 203 |
| 66.656                    | $0.31^{+0.04}_{-0.04}$                          | $42.9^{+3.7}_{-1.8}$     | $0.584^{+0.093}_{-0.083}$        | $1.222^{+0.356}_{-0.206}$       | $2.18^{+0.05}_{-0.04} \times 10^{-10}$             | $2.12^{+0.20}_{-0.19} \times 10^{-11}$               | 162.9 / 150 |
| 67.271                    | $0.15^{+0.03}_{-0.03}$                          | $47.7^{+3.3}_{-1.4}$     | $0.683^{+0.093}_{-0.091}$        | $1.964^{+1.263}_{-0.484}$       | $2.15^{+0.04}_{-0.05} \times 10^{-10}$             | $1.97^{+0.23}_{-0.19} \times 10^{-11}$               | 165.0 / 141 |
| 69.393                    | $0.14^{+0.02}_{-0.02}$                          | $49.3^{+2.8}_{-1.4}$     | $0.543^{+0.073}_{-0.079}$        | $1.360^{+0.102}_{-0.085}$       | $1.89^{+0.02}_{-0.03} \times 10^{-10}$             | $1.98^{+0.07}_{-0.12} \times 10^{-11}$               | 233.3 / 214 |
| 69.594                    | $0.25^{+0.03}_{-0.03}$                          | $46.0^{+3.0}_{-1.4}$     | $0.671^{+0.071}_{-0.071}$        | $1.329^{+0.243}_{-0.177}$       | $1.75^{+0.02}_{-0.03} \times 10^{-10}$             | $2.06^{+0.12}_{-0.14} \times 10^{-11}$               | 221.8 / 195 |
| 70.655                    | $0.16^{+0.02}_{-0.03}$                          | $49.6^{+3.8}_{-1.8}$     | $0.568^{+0.089}_{-0.099}$        | $1.290^{+0.099}_{-0.081}$       | $1.79^{+0.03}_{-0.03} \times 10^{-10}$             | $1.87^{+0.16}_{-0.11} \times 10^{-11}$               | 213.6 / 176 |
| 72.573                    | $0.55^{+0.10}_{-0.08}$                          | $39.4^{+6.5}_{-3.1}$     | $0.445^{+0.136}_{-0.124}$        | $0.929^{+0.494}_{-0.552}$       | $1.27^{+0.05}_{-0.05} \times 10^{-10}$             | $1.58^{+0.25}_{-0.23} \times 10^{-11}$               | 98.1 / 112  |
| 72.58                     | $0.41^{+0.06}_{-0.05}$                          | $45.6^{+4.7}_{-2.7}$     | $0.579^{+0.051}_{-0.074}$        | $1.360^{+0.334}_{-0.155}$       | $1.05^{+0.02}_{-0.03} \times 10^{-10}$             | $1.60^{+0.07}_{-0.11} \times 10^{-11}$               | 194.1 / 175 |
| 73.966                    | $0.39^{+0.03}_{-0.04}$                          | $44.5^{+3.7}_{-1.5}$     | $0.562^{+0.115}_{-0.101}$        | $1.088^{+0.092}_{-0.081}$       | $1.15^{+0.02}_{-0.02} \times 10^{-10}$             | $1.70^{+0.10}_{-0.10} \times 10^{-11}$               | 229.0 / 195 |
| 74.638                    | $0.13^{+0.03}_{-0.03}$                          | $50.6^{+4.4}_{-2.1}$     | $0.702^{+0.107}_{-0.110}$        | $1.274^{+0.252}_{-0.161}$       | $1.18^{+0.03}_{-0.02} \times 10^{-10}$             | $1.46^{+0.12}_{-0.11} \times 10^{-11}$               | 192.3 / 174 |
| 75.567                    | $0.26^{+0.03}_{-0.04}$                          | $46.0^{+3.8}_{-1.6}$     | $0.575^{+0.052}_{-0.060}$        | $1.359^{+0.160}_{-0.136}$       | $1.04^{+0.02}_{-0.03} \times 10^{-10}$             | $1.63^{+0.07}_{-0.10} \times 10^{-11}$               | 202.5 / 178 |
| 76.688                    | $0.10^{+0.07}_{-0.06}$                          | $53.6^{+9.8}_{-4.8}$     | $0.672^{+0.283}_{-0.305}$        | $1.602^{+1.191}_{-0.387}$       | $1.02^{+0.05}_{-0.05} \times 10^{-10}$             | $1.21^{+0.30}_{-0.15} \times 10^{-11}$               | 100.0 / 108 |
| 78.753                    | $0.16^{+0.03}_{-0.03}$                          | $45.9^{+4.4}_{-2.2}$     | $0.694^{+0.069}_{-0.074}$        | $1.289^{+0.328}_{-0.228}$       | $8.47^{+0.19}_{-0.20} \times 10^{-11}$             | $1.31^{+0.07}_{-0.08} \times 10^{-11}$               | 166.8 / 176 |
| 80.941                    | $0.21^{+0.03}_{-0.04}$                          | $46.0^{+3.0}_{-1.7}$     | $0.815^{+0.063}_{-0.068}$        | $1.410^{+0.438}_{-0.243}$       | $7.28^{+0.20}_{-0.19} \times 10^{-11}$             | $1.11^{+0.10}_{-0.06} \times 10^{-11}$               | 199.6 / 172 |



Table 2: As Table 1, but with absorption edges included in the fits (plotted in Fig. 12 of the manuscript).

<sup>f</sup> BB temperatures which were fixed at the average of the temporally adjacent observations. See main text for details.

| T <sub>mid</sub><br>(day) | N <sub>H</sub><br>(10 <sup>22</sup> cm <sup>-2</sup> ) | kT <sub>BB</sub><br>(eV)             | APEC kT <sub>cool</sub><br>(keV)          | APEC kT <sub>hot</sub><br>(keV)           | BB Flux<br>(erg cm <sup>-2</sup> s <sup>-1</sup> )         | APEC Flux<br>(erg cm <sup>-2</sup> s <sup>-1</sup> )       | Cstat/dof    |
|---------------------------|--------------------------------------------------------|--------------------------------------|-------------------------------------------|-------------------------------------------|------------------------------------------------------------|------------------------------------------------------------|--------------|
| <b>2006 eruption</b>      |                                                        |                                      |                                           |                                           |                                                            |                                                            |              |
| 3.178                     | 6.77 <sup>+0.40</sup> <sub>-0.38</sub>                 | —                                    | 0.168 <sup>+0.023</sup> <sub>-0.028</sub> | 8.449 <sup>+0.637</sup> <sub>-0.576</sub> | —                                                          | 1.30 <sup>+0.02</sup> <sub>-0.02</sub> × 10 <sup>-09</sup> | 903.6 / 799  |
| 5.033                     | 2.47 <sup>+0.10</sup> <sub>-0.09</sub>                 | —                                    | 0.248 <sup>+0.017</sup> <sub>-0.024</sub> | 7.407 <sup>+0.312</sup> <sub>-0.310</sub> | —                                                          | 2.01 <sup>+0.02</sup> <sub>-0.02</sub> × 10 <sup>-10</sup> | 1175.1 / 854 |
| 8.183                     | 1.68 <sup>+0.10</sup> <sub>-0.10</sub>                 | —                                    | 0.280 <sup>+0.017</sup> <sub>-0.017</sub> | 5.964 <sup>+0.335</sup> <sub>-0.268</sub> | —                                                          | 1.11 <sup>+0.01</sup> <sub>-0.02</sub> × 10 <sup>-10</sup> | 1007.5 / 781 |
| 10.99                     | 1.75 <sup>+0.16</sup> <sub>-0.20</sub>                 | —                                    | 0.192 <sup>+0.041</sup> <sub>-0.028</sub> | 2.976 <sup>+0.199</sup> <sub>-0.165</sub> | —                                                          | 6.50 <sup>+0.18</sup> <sub>-0.17</sub> × 10 <sup>-10</sup> | 655.4 / 602  |
| 11.057                    | 1.55 <sup>+0.19</sup> <sub>-0.20</sub>                 | —                                    | 0.263 <sup>+0.039</sup> <sub>-0.054</sub> | 3.208 <sup>+0.294</sup> <sub>-0.251</sub> | —                                                          | 6.97 <sup>+0.23</sup> <sub>-0.22</sub> × 10 <sup>-10</sup> | 563.1 / 574  |
| 11.124                    | 2.07 <sup>+0.02</sup> <sub>-0.08</sub>                 | —                                    | 0.138 <sup>+0.011</sup> <sub>-0.007</sub> | 2.688 <sup>+0.093</sup> <sub>-0.082</sub> | —                                                          | 6.79 <sup>+0.18</sup> <sub>-0.12</sub> × 10 <sup>-10</sup> | 574.4 / 585  |
| 13.605                    | 1.56 <sup>+0.10</sup> <sub>-0.11</sub>                 | —                                    | 0.200 <sup>+0.019</sup> <sub>-0.012</sub> | 2.535 <sup>+0.101</sup> <sub>-0.074</sub> | —                                                          | 4.82 <sup>+0.09</sup> <sub>-0.07</sub> × 10 <sup>-10</sup> | 749.4 / 659  |
| 15.616                    | 1.54 <sup>+0.06</sup> <sub>-0.06</sub>                 | —                                    | 0.621 <sup>+0.020</sup> <sub>-0.058</sub> | 2.782 <sup>+0.109</sup> <sub>-0.096</sub> | —                                                          | 3.89 <sup>+0.07</sup> <sub>-0.06</sub> × 10 <sup>-10</sup> | 890.9 / 639  |
| 18.176                    | 1.54 <sup>+0.11</sup> <sub>-0.13</sub>                 | —                                    | 0.800 <sup>+0.044</sup> <sub>-0.038</sub> | 2.533 <sup>+0.256</sup> <sub>-0.203</sub> | —                                                          | 2.31 <sup>+0.09</sup> <sub>-0.04</sub> × 10 <sup>-10</sup> | 408.5 / 437  |
| 18.229                    | 1.50 <sup>+0.16</sup> <sub>-0.18</sub>                 | —                                    | 0.844 <sup>+0.064</sup> <sub>-0.070</sub> | 2.427 <sup>+0.630</sup> <sub>-0.380</sub> | —                                                          | 2.29 <sup>+0.08</sup> <sub>-0.10</sub> × 10 <sup>-10</sup> | 257.0 / 311  |
| 18.239                    | 1.54 <sup>+0.11</sup> <sub>-0.13</sub>                 | —                                    | 0.665 <sup>+0.056</sup> <sub>-0.051</sub> | 2.597 <sup>+0.289</sup> <sub>-0.212</sub> | —                                                          | 2.89 <sup>+0.10</sup> <sub>-0.11</sub> × 10 <sup>-10</sup> | 447.0 / 461  |
| 29.01                     | 0.95 <sup>+0.02</sup> <sub>-0.01</sub>                 | 18.0 <sup>+0.1</sup> <sub>-0.3</sub> | 0.699 <sup>+0.009</sup> <sub>-0.013</sub> | 1.568 <sup>+0.036</sup> <sub>-0.038</sub> | 2.74 <sup>+0.02</sup> <sub>-0.02</sub> × 10 <sup>-10</sup> | 1.48 <sup>+0.02</sup> <sub>-0.02</sub> × 10 <sup>-10</sup> | 715.7 / 464  |
| 29.886                    | 0.65 <sup>+0.03</sup> <sub>-0.01</sub>                 | 25.1 <sup>+0.9</sup> <sub>-0.9</sub> | 0.708 <sup>+0.013</sup> <sub>-0.012</sub> | 1.603 <sup>+0.038</sup> <sub>-0.031</sub> | 8.72 <sup>+0.13</sup> <sub>-0.18</sub> × 10 <sup>-11</sup> | 1.31 <sup>+0.01</sup> <sub>-0.02</sub> × 10 <sup>-10</sup> | 836.0 / 429  |
| 31.02                     | 0.75 <sup>+0.06</sup> <sub>-0.05</sub>                 | 19.1 <sup>+0.9</sup> <sub>-1.1</sub> | 0.630 <sup>+0.013</sup> <sub>-0.011</sub> | 1.574 <sup>+0.034</sup> <sub>-0.035</sub> | 4.57 <sup>+0.11</sup> <sub>-0.17</sub> × 10 <sup>-11</sup> | 1.30 <sup>+0.02</sup> <sub>-0.02</sub> × 10 <sup>-10</sup> | 818.6 / 436  |
| 32.024                    | 0.96 <sup>+0.02</sup> <sub>-0.03</sub>                 | 18.9 <sup>+0.1</sup> <sub>-0.1</sub> | 0.662 <sup>+0.011</sup> <sub>-0.009</sub> | 1.482 <sup>+0.042</sup> <sub>-0.054</sub> | 3.71 <sup>+0.02</sup> <sub>-0.01</sub> × 10 <sup>-10</sup> | 1.21 <sup>+0.01</sup> <sub>-0.02</sub> × 10 <sup>-10</sup> | 796.3 / 423  |
| 32.821                    | 0.78 <sup>+0.01</sup> <sub>-0.01</sub>                 | 20.6 <sup>+0.1</sup> <sub>-0.1</sub> | 0.747 <sup>+0.045</sup> <sub>-0.054</sub> | 1.418 <sup>+0.187</sup> <sub>-0.144</sub> | 1.25 <sup>+0.01</sup> <sub>-0.01</sub> × 10 <sup>-9</sup>  | 9.63 <sup>+0.49</sup> <sub>-0.43</sub> × 10 <sup>-11</sup> | 249.0 / 230  |
| 33.376                    | 1.53 <sup>+0.15</sup> <sub>-0.12</sub>                 | 20.1 <sup>+1.3</sup> <sub>-1.9</sub> | 0.250 <sup>+0.034</sup> <sub>-0.031</sub> | 0.980 <sup>+0.094</sup> <sub>-0.082</sub> | 3.01 <sup>+0.30</sup> <sub>-0.30</sub> × 10 <sup>-11</sup> | 8.94 <sup>+0.34</sup> <sub>-0.29</sub> × 10 <sup>-11</sup> | 278.5 / 274  |
| 33.563                    | 0.77 <sup>+0.16</sup> <sub>-0.10</sub>                 | 18.3 <sup>+1.3</sup> <sub>-1.6</sub> | 0.557 <sup>+0.082</sup> <sub>-0.048</sub> | 2.568 <sup>+0.133</sup> <sub>-0.086</sub> | 4.02 <sup>+0.13</sup> <sub>-0.07</sub> × 10 <sup>-10</sup> | 9.74 <sup>+0.95</sup> <sub>-0.70</sub> × 10 <sup>-11</sup> | 133.4 / 174  |
| 33.632                    | 0.85 <sup>+0.02</sup> <sub>-0.05</sub>                 | 18.6 <sup>+0.8</sup> <sub>-0.5</sub> | 0.786 <sup>+0.044</sup> <sub>-0.057</sub> | 2.451 <sup>+1.247</sup> <sub>-0.539</sub> | 8.58 <sup>+0.15</sup> <sub>-0.05</sub> × 10 <sup>-10</sup> | 9.78 <sup>+1.08</sup> <sub>-0.54</sub> × 10 <sup>-11</sup> | 192.3 / 209  |
| 33.768                    | 0.64 <sup>+0.01</sup> <sub>-0.01</sub>                 | 30.2 <sup>+0.4</sup> <sub>-0.1</sub> | 0.628 <sup>+0.060</sup> <sub>-0.056</sub> | 1.329 <sup>+0.098</sup> <sub>-0.084</sub> | 2.07 <sup>+0.01</sup> <sub>-0.01</sub> × 10 <sup>-9</sup>  | 8.62 <sup>+0.48</sup> <sub>-0.33</sub> × 10 <sup>-11</sup> | 315.7 / 231  |
| 33.838                    | 0.65 <sup>+0.01</sup> <sub>-0.01</sub>                 | 32.4 <sup>+0.1</sup> <sub>-0.1</sub> | 0.783 <sup>+0.091</sup> <sub>-0.113</sub> | 1.418 <sup>+0.099</sup> <sub>-0.088</sub> | 2.39 <sup>+0.01</sup> <sub>-0.01</sub> × 10 <sup>-9</sup>  | 9.10 <sup>+0.30</sup> <sub>-0.42</sub> × 10 <sup>-11</sup> | 354.4 / 298  |
| 33.907                    | 0.80 <sup>+0.01</sup> <sub>-0.04</sub>                 | 20.3 <sup>+0.1</sup> <sub>-0.1</sub> | 0.706 <sup>+0.021</sup> <sub>-0.022</sub> | 1.576 <sup>+0.121</sup> <sub>-0.105</sub> | 8.95 <sup>+0.07</sup> <sub>-0.02</sub> × 10 <sup>-10</sup> | 9.33 <sup>+0.29</sup> <sub>-0.28</sub> × 10 <sup>-11</sup> | 312.0 / 306  |
| 33.973                    | 0.78 <sup>+0.06</sup> <sub>-0.04</sub>                 | 18.3 <sup>+0.7</sup> <sub>-0.8</sub> | 0.562 <sup>+0.034</sup> <sub>-0.037</sub> | 1.490 <sup>+0.100</sup> <sub>-0.086</sub> | 3.87 <sup>+0.09</sup> <sub>-0.02</sub> × 10 <sup>-10</sup> | 9.31 <sup>+0.27</sup> <sub>-0.25</sub> × 10 <sup>-11</sup> | 392.4 / 310  |
| 34.04                     | 0.75 <sup>+0.01</sup> <sub>-0.01</sub>                 | 22.2 <sup>+0.1</sup> <sub>-0.1</sub> | 0.807 <sup>+0.021</sup> <sub>-0.035</sub> | 1.482 <sup>+0.106</sup> <sub>-0.089</sub> | 9.47 <sup>+0.09</sup> <sub>-0.02</sub> × 10 <sup>-10</sup> | 9.49 <sup>+0.27</sup> <sub>-0.26</sub> × 10 <sup>-11</sup> | 338.6 / 330  |
| 32.907                    | 0.65 <sup>+0.04</sup> <sub>-0.01</sub>                 | 33.4 <sup>+1.9</sup> <sub>-0.2</sub> | 0.768 <sup>+0.208</sup> <sub>-0.173</sub> | 1.363 <sup>+0.078</sup> <sub>-0.063</sub> | 1.75 <sup>+0.01</sup> <sub>-0.01</sub> × 10 <sup>-9</sup>  | 1.06 <sup>+0.04</sup> <sub>-0.04</sub> × 10 <sup>-10</sup> | 324.9 / 268  |
| 34.107                    | 0.71 <sup>+0.01</sup> <sub>-0.01</sub>                 | 25.4 <sup>+0.1</sup> <sub>-0.1</sub> | 0.802 <sup>+0.028</sup> <sub>-0.018</sub> | 1.833 <sup>+0.211</sup> <sub>-0.155</sub> | 1.93 <sup>+0.01</sup> <sub>-0.01</sub> × 10 <sup>-9</sup>  | 1.00 <sup>+0.02</sup> <sub>-0.04</sub> × 10 <sup>-10</sup> | 376.8 / 334  |
| 34.166                    | 0.56 <sup>+0.04</sup> <sub>-0.04</sub>                 | 31.2 <sup>+0.4</sup> <sub>-1.6</sub> | 0.885 <sup>+0.051</sup> <sub>-0.030</sub> | 1.702 <sup>+0.221</sup> <sub>-0.145</sub> | 2.81 <sup>+0.01</sup> <sub>-0.01</sub> × 10 <sup>-9</sup>  | 1.00 <sup>+0.05</sup> <sub>-0.05</sub> × 10 <sup>-10</sup> | 377.5 / 261  |
| 34.18                     | 0.73 <sup>+0.03</sup> <sub>-0.02</sub>                 | 30.5 <sup>+1.5</sup> <sub>-0.2</sub> | 1.009 <sup>+0.061</sup> <sub>-0.370</sub> | 1.507 <sup>+3.082</sup> <sub>-0.801</sub> | 3.06 <sup>+0.01</sup> <sub>-0.01</sub> × 10 <sup>-9</sup>  | 8.80 <sup>+0.37</sup> <sub>-0.38</sub> × 10 <sup>-11</sup> | 274.4 / 266  |
| 32.956                    | 0.72 <sup>+0.01</sup> <sub>-0.02</sub>                 | 28.8 <sup>+0.6</sup> <sub>-0.5</sub> | 0.735 <sup>+0.088</sup> <sub>-0.094</sub> | 1.409 <sup>+0.162</sup> <sub>-0.122</sub> | 1.94 <sup>+0.01</sup> <sub>-0.01</sub> × 10 <sup>-9</sup>  | 9.49 <sup>+0.58</sup> <sub>-0.42</sub> × 10 <sup>-11</sup> | 268.6 / 251  |
| 32.973                    | 0.72 <sup>+0.03</sup> <sub>-0.01</sub>                 | 31.7 <sup>+2.3</sup> <sub>-1.2</sub> | 0.926 <sup>+0.040</sup> <sub>-0.039</sub> | 1.852 <sup>+0.449</sup> <sub>-0.287</sub> | 1.79 <sup>+0.01</sup> <sub>-0.01</sub> × 10 <sup>-9</sup>  | 9.51 <sup>+0.61</sup> <sub>-0.46</sub> × 10 <sup>-11</sup> | 274.0 / 257  |
| 33.032                    | 0.62 <sup>+0.01</sup> <sub>-0.03</sub>                 | 28.3 <sup>+0.1</sup> <sub>-0.1</sub> | 0.754 <sup>+0.039</sup> <sub>-0.020</sub> | 1.507 <sup>+0.064</sup> <sub>-0.061</sub> | 1.85 <sup>+0.01</sup> <sub>-0.01</sub> × 10 <sup>-9</sup>  | 1.04 <sup>+0.03</sup> <sub>-0.03</sub> × 10 <sup>-10</sup> | 601.2 / 316  |
| 33.107                    | 0.88 <sup>+0.01</sup> <sub>-0.02</sub>                 | 23.8 <sup>+1.3</sup> <sub>-0.1</sub> | 0.883 <sup>+0.044</sup> <sub>-0.036</sub> | 1.450 <sup>+0.519</sup> <sub>-0.223</sub> | 1.87 <sup>+0.01</sup> <sub>-0.01</sub> × 10 <sup>-9</sup>  | 9.80 <sup>+0.71</sup> <sub>-0.69</sub> × 10 <sup>-11</sup> | 289.0 / 241  |
| 33.17                     | 0.86 <sup>+0.10</sup> <sub>-0.07</sub>                 | 20.4 <sup>+1.2</sup> <sub>-1.0</sub> | 0.503 <sup>+0.086</sup> <sub>-0.162</sub> | 1.367 <sup>+0.277</sup> <sub>-0.136</sub> | 1.37 <sup>+0.02</sup> <sub>-0.01</sub> × 10 <sup>-9</sup>  | 9.81 <sup>+0.94</sup> <sub>-0.85</sub> × 10 <sup>-11</sup> | 120.0 / 156  |
| 33.178                    | 1.09 <sup>+0.01</sup> <sub>-0.01</sub>                 | 20.7 <sup>+0.1</sup> <sub>-0.1</sub> | 0.572 <sup>+0.047</sup> <sub>-0.046</sub> | 1.185 <sup>+0.115</sup> <sub>-0.105</sub> | 1.58 <sup>+0.01</sup> <sub>-0.01</sub> × 10 <sup>-9</sup>  | 8.50 <sup>+0.41</sup> <sub>-0.42</sub> × 10 <sup>-11</sup> | 208.8 / 220  |
| 33.242                    | 1.03 <sup>+0.01</sup> <sub>-0.02</sub>                 | 21.0 <sup>+0.1</sup> <sub>-0.1</sub> | 0.623 <sup>+0.069</sup> <sub>-0.060</sub> | 1.006 <sup>+0.052</sup> <sub>-0.038</sub> | 1.65 <sup>+0.01</sup> <sub>-0.01</sub> × 10 <sup>-9</sup>  | 9.44 <sup>+0.31</sup> <sub>-0.31</sub> × 10 <sup>-11</sup> | 293.1 / 275  |
| 33.309                    | 0.72 <sup>+0.05</sup> <sub>-0.03</sub>                 | 19.4 <sup>+0.1</sup> <sub>-0.1</sub> | 0.653 <sup>+0.032</sup> <sub>-0.047</sub> | 1.373 <sup>+0.062</sup> <sub>-0.080</sub> | 2.57 <sup>+0.05</sup> <sub>-0.03</sub> × 10 <sup>-10</sup> | 9.87 <sup>+0.34</sup> <sub>-0.32</sub> × 10 <sup>-11</sup> | 293.1 / 283  |
| 33.697                    | 0.71 <sup>+0.01</sup> <sub>-0.01</sub>                 | 26.9 <sup>+0.1</sup> <sub>-0.1</sub> | 0.908 <sup>+0.034</sup> <sub>-0.050</sub> | 1.690 <sup>+0.183</sup> <sub>-0.135</sub> | 1.84 <sup>+0.01</sup> <sub>-0.01</sub> × 10 <sup>-9</sup>  | 9.79 <sup>+0.37</sup> <sub>-0.37</sub> × 10 <sup>-11</sup> | 388.1 / 289  |
| 34.707                    | 0.59 <sup>+0.01</sup> <sub>-0.03</sub>                 | 30.1 <sup>+1.1</sup> <sub>-0.1</sub> | 0.956 <sup>+0.061</sup> <sub>-0.071</sub> | 3.007 <sup>+4.549</sup> <sub>-1.026</sub> | 1.50 <sup>+0.02</sup> <sub>-0.01</sub> × 10 <sup>-9</sup>  | 8.09 <sup>+0.86</sup> <sub>-0.78</sub> × 10 <sup>-11</sup> | 172.8 / 172  |
| 35.925                    | 0.71 <sup>+0.07</sup> <sub>-0.08</sub>                 | 22.7 <sup>+0.1</sup> <sub>-0.5</sub> | 0.566 <sup>+0.075</sup> <sub>-0.091</sub> | 1.229 <sup>+0.114</sup> <sub>-0.095</sub> | 6.37 <sup>+0.16</sup> <sub>-0.06</sub> × 10 <sup>-10</sup> | 7.97 <sup>+0.56</sup> <sub>-0.62</sub> × 10 <sup>-11</sup> | 155.5 / 184  |
| 35.979                    | 0.73 <sup>+0.01</sup> <sub>-0.01</sub>                 | 23.8 <sup>+1.0</sup> <sub>-0.1</sub> | 0.644 <sup>+0.029</sup> <sub>-0.049</sub> | 1.326 <sup>+0.069</sup> <sub>-0.059</sub> | 5.80 <sup>+0.05</sup> <sub>-0.01</sub> × 10 <sup>-10</sup> | 7.39 <sup>+0.27</sup> <sub>-0.20</sub> × 10 <sup>-11</sup> | 405.3 / 301  |
| 36.049                    | 0.76 <sup>+0.01</sup> <sub>-0.01</sub>                 | 20.1 <sup>+0.1</sup> <sub>-0.3</sub> | 0.740 <sup>+0.021</sup> <sub>-0.029</sub> | 1.612 <sup>+0.159</sup> <sub>-0.129</sub> | 7.01 <sup>+0.06</sup> <sub>-0.02</sub> × 10 <sup>-10</sup> | 8.64 <sup>+0.32</sup> <sub>-0.26</sub> × 10 <sup>-11</sup> | 340.9 / 293  |
| 36.113                    | 0.90 <sup>+0.01</sup> <sub>-0.02</sub>                 | 22.4 <sup>+0.1</sup> <sub>-0.1</sub> | 0.579 <sup>+0.028</sup> <sub>-0.020</sub> | 1.164 <sup>+0.035</sup> <sub>-0.045</sub> | 8.50 <sup>+0.09</sup> <sub>-0.02</sub> × 10 <sup>-10</sup> | 8.80 <sup>+0.20</sup> <sub>-0.21</sub> × 10 <sup>-11</sup> | 332.5 / 326  |
| 36.785                    | 0.69 <sup>+0.12</sup> <sub>-0.01</sub>                 | 20.3 <sup>+1.2</sup> <sub>-1.2</sub> | 0.639 <sup>+0.030</sup> <sub>-0.069</sub> | 1.244 <sup>+0.083</sup> <sub>-0.094</sub> | 4.38 <sup>+0.08</sup> <sub>-0.03</sub> × 10 <sup>-10</sup> | 7.33 <sup>+0.44</sup> <sub>-0.38</sub> × 10 <sup>-11</sup> | 237.9 / 214  |
| 36.851                    | 0.49 <sup>+0.06</sup> <sub>-0.01</sub>                 | 27.2 <sup>+0.1</sup> <sub>-0.1</sub> | 0.583 <sup>+0.094</sup> <sub>-0.085</sub> | 1.316 <sup>+0.099</sup> <sub>-0.092</sub> | 5.04 <sup>+0.09</sup> <sub>-0.03</sub> × 10 <sup>-10</sup> | 8.10 <sup>+0.72</sup> <sub>-0.37</sub> × 10 <sup>-11</sup> | 264.1 / 207  |
| 36.917                    | 0.22 <sup>+0.06</sup> <sub>-0.03</sub>                 | 65.4 <sup>+8.3</sup> <sub>-8.2</sub> | 0.774 <sup>+0.230</sup> <sub>-0.253</sub> | 1.575 <sup>+0.131</sup> <sub>-0.101</sub> | 8.74 <sup>+0.12</sup> <sub>-0.05</sub> × 10 <sup>-10</sup> | 7.19 <sup>+0.83</sup> <sub>-0.51</sub> × 10 <sup>-11</sup> | 221.1 / 209  |
| 36.985                    | 0.26 <sup>+0.01</sup> <sub>-0.03</sub>                 | 63.8 <sup>+9.5</sup> <sub>-3.6</sub> | 1.030 <sup>+0.062</sup> <sub>-0.064</sub> | 1.812 <sup>+0.316</sup> <sub>-0.243</sub> | 8.08 <sup>+0.15</sup> <sub>-0.04</sub> × 10 <sup>-10</sup> | 7.81 <sup>+0.50</sup> <sub>-0.47</sub> × 10 <sup>-11</sup> | 231.6 / 219  |
| 37.051                    | 0.23 <sup>+0.01</sup> <sub>-0.02</sub>                 | 61.5 <sup>+9.2</sup> <sub>-2.7</sub> | 0.796 <sup>+0.169</sup> <sub>-0.151</sub> | 1.634 <sup>+0.141</sup> <sub>-0.101</sub> | 1.08 <sup>+0.01</sup> <sub>-0.01</sub> × 10 <sup>-9</sup>  | 7.23 <sup>+0.71</sup> <sub>-0.49</sub> × 10 <sup>-11</sup> | 240.9 / 217  |
| 36.168                    | 0.70 <sup>+0.03</sup> <sub>-0.03</sub>                 | 23.1 <sup>+0.1</sup> <sub>-0.1</sub> | 0.627 <sup>+0.096</sup> <sub>-0.095</sub> | 1.223 <sup>+0.121</sup> <sub>-0.104</sub> | 6.23 <sup>+0.13</sup> <sub>-0.04</sub> × 10 <sup>-10</sup> | 8.02 <sup>+0.39</sup> <sub>-0.44</sub> × 10 <sup>-11</sup> | 210.5 / 202  |
| 36.185                    | 0.55 <sup>+0.01</sup> <sub>-0.01</sub>                 | 27.9 <sup>+0.1</sup> <sub>-0.2</sub> | 0.681 <sup>+0.041</sup> <sub>-0.041</sub> | 1.500 <sup>+0.085</sup> <sub>-0.070</sub> | 6.16 <sup>+0.06</sup> <sub>-0.02</sub> × 10 <sup>-10</sup> | 8.92 <sup>+0.28</sup> <sub>-0.27</sub> × 10 <sup>-11</sup> | 287.5 / 300  |
| 36.247                    | 0.26 <sup>+0.01</sup> <sub>-0.03</sub>                 | 54.4 <sup>+4.5</sup> <sub>-4.5</sub> | 0.580 <sup>+0.028</sup> <sub>-0.035</sub> | 1.764 <sup>+0.067</sup> <sub>-0.065</sub> | 4.93 <sup>+0.05</sup> <sub>-0.04</sub> × 10 <sup>-10</sup> | 1.00 <sup>+0.04</sup> <sub>-0.04</sub> × 10 <sup>-10</sup> | 437.0 / 343  |
| 36.314                    | 0.62 <sup>+0.02</sup> <sub>-0.02</sub>                 | 26.3 <sup>+0.6</sup> <sub>-0.4</sub> | 0.747 <sup>+0.026</sup> <sub>-0.029</sub> | 1.597 <sup>+0.102</sup> <sub>-0.100</sub> | 5.43 <sup>+0.04</sup> <sub>-0.02</sub> × 10 <sup>-10</sup> | 8.29 <sup>+0.25</sup> <sub>-0.23</sub> × 10 <sup>-11</sup> | 421.0 / 316  |
| 36.367                    | 0.98 <sup>+0.18</sup> <sub>-0.02</sub>                 | 19.6 <sup>+3.1</sup> <sub>-0.6</sub> | 0.150 <sup>+0.150</sup> <sub>-0.150</sub> | 0.727 <sup>+0.089</sup> <sub>-0.071</sub> | 9.16 <sup>+0.28</sup> <sub>-0.08</sub> × 10 <sup>-10</sup> | 6.38 <sup>+0.76</sup> <sub>-0.82</sub> × 10 <sup>-11</sup> | 120.1 / 115  |

Continued on next page

Table 2 – continued from previous page

| T <sub>mid</sub><br>(day) | N <sub>H</sub><br>(10 <sup>22</sup> cm <sup>-2</sup> ) | kT <sub>BB</sub><br>(eV)              | APEC kT <sub>cool</sub><br>(keV)          | APEC kT <sub>hot</sub><br>(keV)           | BB Flux<br>(erg cm <sup>-2</sup> s <sup>-1</sup> )         | APEC Flux<br>(erg cm <sup>-2</sup> s <sup>-1</sup> )       | Cstat/dof   |
|---------------------------|--------------------------------------------------------|---------------------------------------|-------------------------------------------|-------------------------------------------|------------------------------------------------------------|------------------------------------------------------------|-------------|
| 36.387                    | 0.62 <sup>+0.01</sup> <sub>-0.01</sub>                 | 24.7 <sup>+0.2</sup> <sub>-0.3</sub>  | 0.782 <sup>+0.034</sup> <sub>-0.067</sub> | 1.663 <sup>+0.167</sup> <sub>-0.149</sub> | 8.48 <sup>+0.07</sup> <sub>-0.03</sub> × 10 <sup>-10</sup> | 7.02 <sup>+0.39</sup> <sub>-0.32</sub> × 10 <sup>-11</sup> | 317.7 / 268 |
| 36.436                    | 0.78 <sup>+0.03</sup> <sub>-0.03</sub>                 | 20.1 <sup>+0.4</sup> <sub>-0.7</sub>  | 0.583 <sup>+0.047</sup> <sub>-0.087</sub> | 1.068 <sup>+0.089</sup> <sub>-0.042</sub> | 7.45 <sup>+0.13</sup> <sub>-0.04</sub> × 10 <sup>-10</sup> | 7.85 <sup>+0.60</sup> <sub>-0.46</sub> × 10 <sup>-11</sup> | 185.7 / 199 |
| 36.46                     | 0.86 <sup>+0.08</sup> <sub>-0.10</sub>                 | 20.6 <sup>+2.1</sup> <sub>-0.3</sub>  | 0.749 <sup>+0.088</sup> <sub>-0.092</sub> | 1.219 <sup>+0.549</sup> <sub>-0.196</sub> | 5.92 <sup>+0.16</sup> <sub>-0.05</sub> × 10 <sup>-10</sup> | 6.72 <sup>+0.61</sup> <sub>-0.53</sub> × 10 <sup>-11</sup> | 159.5 / 166 |
| 36.506                    | 0.85 <sup>+0.12</sup> <sub>-0.08</sub>                 | 18.0 <sup>+1.2</sup> <sub>-1.4</sub>  | 0.686 <sup>+0.048</sup> <sub>-0.069</sub> | 1.542 <sup>+0.162</sup> <sub>-0.206</sub> | 5.49 <sup>+0.09</sup> <sub>-0.04</sub> × 10 <sup>-10</sup> | 7.34 <sup>+0.79</sup> <sub>-0.45</sub> × 10 <sup>-11</sup> | 205.4 / 181 |
| 37.123                    | 0.38 <sup>+0.01</sup> <sub>-0.01</sub>                 | 56.2 <sup>+4.3</sup> <sub>-2.2</sub>  | 0.433 <sup>+0.051</sup> <sub>-0.034</sub> | 1.433 <sup>+0.087</sup> <sub>-0.055</sub> | 1.62 <sup>+0.01</sup> <sub>-0.01</sub> × 10 <sup>-9</sup>  | 7.53 <sup>+0.42</sup> <sub>-0.41</sub> × 10 <sup>-11</sup> | 351.4 / 272 |
| 37.192                    | 0.39 <sup>+0.01</sup> <sub>-0.01</sub>                 | 57.4 <sup>+3.8</sup> <sub>-0.4</sub>  | 1.055 <sup>+0.121</sup> <sub>-0.110</sub> | 1.447 <sup>+0.107</sup> <sub>-0.071</sub> | 2.31 <sup>+0.01</sup> <sub>-0.01</sub> × 10 <sup>-9</sup>  | 7.46 <sup>+0.36</sup> <sub>-0.33</sub> × 10 <sup>-11</sup> | 298.4 / 266 |
| 37.259                    | 0.60 <sup>+0.01</sup> <sub>-0.03</sub>                 | 36.4 <sup>+1.6</sup> <sub>-0.5</sub>  | 0.787 <sup>+0.073</sup> <sub>-0.073</sub> | 1.432 <sup>+0.122</sup> <sub>-0.106</sub> | 2.04 <sup>+0.01</sup> <sub>-0.01</sub> × 10 <sup>-9</sup>  | 7.78 <sup>+0.35</sup> <sub>-0.36</sub> × 10 <sup>-11</sup> | 286.2 / 255 |
| 37.326                    | 0.33 <sup>+0.01</sup> <sub>-0.01</sub>                 | 48.1 <sup>+1.1</sup> <sub>-2.8</sub>  | 1.071 <sup>+0.050</sup> <sub>-0.067</sub> | 1.596 <sup>+0.121</sup> <sub>-0.119</sub> | 2.50 <sup>+0.01</sup> <sub>-0.01</sub> × 10 <sup>-9</sup>  | 7.78 <sup>+0.33</sup> <sub>-0.35</sub> × 10 <sup>-11</sup> | 397.5 / 256 |
| 37.395                    | 0.66 <sup>+0.02</sup> <sub>-0.03</sub>                 | 30.4 <sup>+1.4</sup> <sub>-0.3</sub>  | 0.528 <sup>+0.169</sup> <sub>-0.176</sub> | 1.871 <sup>+0.331</sup> <sub>-0.248</sub> | 1.55 <sup>+0.01</sup> <sub>-0.01</sub> × 10 <sup>-9</sup>  | 8.23 <sup>+0.61</sup> <sub>-0.55</sub> × 10 <sup>-11</sup> | 280.8 / 238 |
| 37.442                    | 0.70 <sup>+0.02</sup> <sub>-0.04</sub>                 | 28.0 <sup>+2.3</sup> <sub>-0.1</sub>  | 0.902 <sup>+0.074</sup> <sub>-0.081</sub> | 2.046 <sup>+1.430</sup> <sub>-0.628</sub> | 1.58 <sup>+0.02</sup> <sub>-0.01</sub> × 10 <sup>-9</sup>  | 7.56 <sup>+1.07</sup> <sub>-0.92</sub> × 10 <sup>-11</sup> | 178.1 / 183 |
| 37.465                    | 0.79 <sup>+0.01</sup> <sub>-0.07</sub>                 | 23.0 <sup>+0.1</sup> <sub>-0.1</sub>  | 0.701 <sup>+0.075</sup> <sub>-0.164</sub> | 1.170 <sup>+0.324</sup> <sub>-0.153</sub> | 1.29 <sup>+0.01</sup> <sub>-0.01</sub> × 10 <sup>-9</sup>  | 7.19 <sup>+0.57</sup> <sub>-0.46</sub> × 10 <sup>-11</sup> | 153.0 / 175 |
| 37.794                    | 0.57 <sup>+0.02</sup> <sub>-0.03</sub>                 | 37.7 <sup>+1.1</sup> <sub>-0.3</sub>  | 0.468 <sup>+0.133</sup> <sub>-0.053</sub> | 1.154 <sup>+0.070</sup> <sub>-0.050</sub> | 3.52 <sup>+0.02</sup> <sub>-0.01</sub> × 10 <sup>-9</sup>  | 8.24 <sup>+0.76</sup> <sub>-0.50</sub> × 10 <sup>-11</sup> | 215.2 / 193 |
| 37.989                    | 0.59 <sup>+0.01</sup> <sub>-0.01</sub>                 | 37.8 <sup>+0.6</sup> <sub>-0.1</sub>  | 0.984 <sup>+0.041</sup> <sub>-0.039</sub> | 1.354 <sup>+0.079</sup> <sub>-0.075</sub> | 3.50 <sup>+0.01</sup> <sub>-0.01</sub> × 10 <sup>-9</sup>  | 7.45 <sup>+0.22</sup> <sub>-0.22</sub> × 10 <sup>-11</sup> | 533.0 / 314 |
| 38.056                    | 0.40 <sup>+0.01</sup> <sub>-0.01</sub>                 | 45.3 <sup>+0.1</sup> <sub>-0.1</sub>  | 1.016 <sup>+0.047</sup> <sub>-0.060</sub> | 1.460 <sup>+0.061</sup> <sub>-0.050</sub> | 3.90 <sup>+0.01</sup> <sub>-0.01</sub> × 10 <sup>-9</sup>  | 7.36 <sup>+0.25</sup> <sub>-0.23</sub> × 10 <sup>-11</sup> | 752.5 / 312 |
| 38.123                    | 0.69 <sup>+0.01</sup> <sub>-0.01</sub>                 | 32.8 <sup>+0.2</sup> <sub>-1.2</sub>  | 0.633 <sup>+0.054</sup> <sub>-0.049</sub> | 1.119 <sup>+0.045</sup> <sub>-0.041</sub> | 2.96 <sup>+0.01</sup> <sub>-0.01</sub> × 10 <sup>-9</sup>  | 7.72 <sup>+0.22</sup> <sub>-0.22</sub> × 10 <sup>-11</sup> | 363.6 / 294 |
| 38.18                     | 0.63 <sup>+0.01</sup> <sub>-0.01</sub>                 | 25.9 <sup>+0.1</sup> <sub>-0.1</sub>  | 0.780 <sup>+0.043</sup> <sub>-0.079</sub> | 2.315 <sup>+0.950</sup> <sub>-0.500</sub> | 2.01 <sup>+0.01</sup> <sub>-0.01</sub> × 10 <sup>-9</sup>  | 7.05 <sup>+0.43</sup> <sub>-0.40</sub> × 10 <sup>-11</sup> | 255.6 / 213 |
| 38.262                    | 0.70 <sup>+0.02</sup> <sub>-0.04</sub>                 | 25.6 <sup>+2.0</sup> <sub>-0.2</sub>  | 0.540 <sup>+0.095</sup> <sub>-0.106</sub> | 0.959 <sup>+0.054</sup> <sub>-0.059</sub> | 1.66 <sup>+0.01</sup> <sub>-0.01</sub> × 10 <sup>-9</sup>  | 7.26 <sup>+0.50</sup> <sub>-0.44</sub> × 10 <sup>-11</sup> | 195.5 / 208 |
| 38.329                    | 0.67 <sup>+0.01</sup> <sub>-0.04</sub>                 | 28.7 <sup>+0.1</sup> <sub>-0.1</sub>  | 0.848 <sup>+0.043</sup> <sub>-0.047</sub> | 2.715 <sup>+1.696</sup> <sub>-0.834</sub> | 2.29 <sup>+0.01</sup> <sub>-0.01</sub> × 10 <sup>-9</sup>  | 7.91 <sup>+0.56</sup> <sub>-0.50</sub> × 10 <sup>-11</sup> | 209.8 / 215 |
| 38.399                    | 0.56 <sup>+0.13</sup> <sub>-0.12</sub>                 | 50.4 <sup>+6.2</sup> <sub>-11.5</sub> | 0.470 <sup>+0.356</sup> <sub>-0.096</sub> | 2.007 <sup>+0.723</sup> <sub>-0.316</sub> | 2.67 <sup>+0.02</sup> <sub>-0.01</sub> × 10 <sup>-9</sup>  | 8.88 <sup>+0.61</sup> <sub>-0.60</sub> × 10 <sup>-11</sup> | 191.8 / 211 |
| 38.446                    | 0.44 <sup>+0.02</sup> <sub>-0.03</sub>                 | 38.1 <sup>+1.9</sup> <sub>-1.0</sub>  | 0.174 <sup>+0.071</sup> <sub>-0.174</sub> | 1.514 <sup>+0.225</sup> <sub>-0.164</sub> | 2.43 <sup>+0.03</sup> <sub>-0.01</sub> × 10 <sup>-9</sup>  | 7.76 <sup>+1.68</sup> <sub>-1.37</sub> × 10 <sup>-11</sup> | 149.6 / 139 |
| 38.514                    | 0.16 <sup>+0.01</sup> <sub>-0.02</sub>                 | 67.8 <sup>+14.</sup> <sub>-0.6</sub>  | 0.351 <sup>+0.082</sup> <sub>-0.067</sub> | 1.887 <sup>+0.311</sup> <sub>-0.194</sub> | 8.78 <sup>+0.17</sup> <sub>-0.10</sub> × 10 <sup>-10</sup> | 8.96 <sup>+1.05</sup> <sub>-1.06</sub> × 10 <sup>-11</sup> | 177.0 / 185 |
| 38.582                    | 0.37 <sup>+0.13</sup> <sub>-0.13</sub>                 | 36.5 <sup>+1.0</sup> <sub>-0.3</sub>  | 0.777 <sup>+0.043</sup> <sub>-0.120</sub> | 1.678 <sup>+0.337</sup> <sub>-0.242</sub> | 1.17 <sup>+0.08</sup> <sub>-0.04</sub> × 10 <sup>-10</sup> | 6.77 <sup>+0.46</sup> <sub>-0.47</sub> × 10 <sup>-11</sup> | 232.3 / 202 |
| 38.648                    | 0.17 <sup>+0.03</sup> <sub>-0.01</sub>                 | 49.0 <sup>+6.5</sup> <sub>-2.7</sub>  | 0.880 <sup>+0.049</sup> <sub>-0.095</sub> | 1.735 <sup>+0.232</sup> <sub>-0.187</sub> | 1.47 <sup>+0.07</sup> <sub>-0.04</sub> × 10 <sup>-10</sup> | 7.07 <sup>+0.73</sup> <sub>-0.68</sub> × 10 <sup>-11</sup> | 195.1 / 198 |
| 38.716                    | 0.42 <sup>+0.02</sup> <sub>-0.04</sub>                 | 34.2 <sup>+2.6</sup> <sub>-0.6</sub>  | 0.518 <sup>+0.065</sup> <sub>-0.077</sub> | 1.790 <sup>+0.249</sup> <sub>-0.189</sub> | 7.06 <sup>+0.11</sup> <sub>-0.05</sub> × 10 <sup>-10</sup> | 7.74 <sup>+0.42</sup> <sub>-0.51</sub> × 10 <sup>-11</sup> | 191.7 / 203 |
| 38.998                    | 0.21 <sup>+0.01</sup> <sub>-0.01</sub>                 | 56.5 <sup>+2.3</sup> <sub>-3.0</sub>  | 0.860 <sup>+0.133</sup> <sub>-0.120</sub> | 1.456 <sup>+0.175</sup> <sub>-0.119</sub> | 8.56 <sup>+0.12</sup> <sub>-0.04</sub> × 10 <sup>-10</sup> | 6.47 <sup>+0.43</sup> <sub>-0.46</sub> × 10 <sup>-11</sup> | 221.8 / 194 |
| 39.065                    | 0.05 <sup>+0.02</sup> <sub>-0.01</sub>                 | 79.1 <sup>+20.9</sup> <sub>-5.4</sub> | 0.486 <sup>+0.068</sup> <sub>-0.061</sub> | 1.661 <sup>+0.153</sup> <sub>-0.122</sub> | 2.38 <sup>+0.10</sup> <sub>-0.09</sub> × 10 <sup>-10</sup> | 9.06 <sup>+0.79</sup> <sub>-0.92</sub> × 10 <sup>-11</sup> | 207.3 / 198 |
| 39.132                    | 0.08 <sup>+0.04</sup> <sub>-0.08</sub>                 | 76.8 <sup>+21.</sup> <sub>-7.6</sub>  | 0.372 <sup>+0.162</sup> <sub>-0.046</sub> | 1.836 <sup>+0.251</sup> <sub>-0.162</sub> | 1.61 <sup>+0.08</sup> <sub>-0.13</sub> × 10 <sup>-10</sup> | 1.02 <sup>+0.08</sup> <sub>-0.13</sub> × 10 <sup>-10</sup> | 196.9 / 199 |
| 39.188                    | 0.00 <sup>+0.05</sup> <sub>-0.01</sub>                 | 79.3 <sup>+11.6</sup> <sub>-8.4</sub> | 0.150 <sup>+0.150</sup> <sub>-0.150</sub> | —                                         | 6.44 <sup>+0.79</sup> <sub>-0.45</sub> × 10 <sup>-10</sup> | 7.44 <sup>+7.37</sup> <sub>-4.53</sub> × 10 <sup>-11</sup> | 67.8 / 51   |
| 39.255                    | 0.47 <sup>+0.04</sup> <sub>-0.02</sub>                 | 41.7 <sup>+4.6</sup> <sub>-0.5</sub>  | 0.383 <sup>+0.121</sup> <sub>-0.096</sub> | —                                         | 6.37 <sup>+0.65</sup> <sub>-0.71</sub> × 10 <sup>-10</sup> | 1.51 <sup>+1.24</sup> <sub>-0.71</sub> × 10 <sup>-10</sup> | 52.4 / 64   |
| 39.325                    | 0.00 <sup>+0.02</sup> <sub>-0.01</sub>                 | 65.0 <sup>+5.4</sup> <sub>-2.0</sub>  | 0.430 <sup>+0.229</sup> <sub>-0.281</sub> | 1.363 <sup>+0.230</sup> <sub>-0.158</sub> | 3.61 <sup>+0.25</sup> <sub>-0.15</sub> × 10 <sup>-10</sup> | 6.41 <sup>+2.92</sup> <sub>-1.51</sub> × 10 <sup>-11</sup> | 100.9 / 98  |
| 39.194                    | 0.06 <sup>+0.01</sup> <sub>-0.01</sub>                 | 93.4 <sup>+6.9</sup> <sub>-4.4</sub>  | 0.408 <sup>+0.035</sup> <sub>-0.026</sub> | 1.728 <sup>+0.149</sup> <sub>-0.106</sub> | 8.15 <sup>+0.14</sup> <sub>-0.08</sub> × 10 <sup>-10</sup> | 1.06 <sup>+0.10</sup> <sub>-0.09</sub> × 10 <sup>-10</sup> | 347.4 / 230 |
| 39.261                    | 0.12 <sup>+0.02</sup> <sub>-0.04</sub>                 | 75.8 <sup>+12.9</sup> <sub>-6.5</sub> | 1.068 <sup>+0.109</sup> <sub>-0.127</sub> | 1.625 <sup>+0.278</sup> <sub>-0.171</sub> | 9.45 <sup>+0.11</sup> <sub>-0.04</sub> × 10 <sup>-10</sup> | 7.83 <sup>+0.46</sup> <sub>-0.47</sub> × 10 <sup>-11</sup> | 320.4 / 226 |
| 39.33                     | 0.00 <sup>+0.01</sup> <sub>-0.01</sub>                 | 67.8 <sup>+1.1</sup> <sub>-1.9</sub>  | 0.311 <sup>+0.062</sup> <sub>-0.036</sub> | 1.669 <sup>+0.144</sup> <sub>-0.134</sub> | 4.38 <sup>+0.14</sup> <sub>-0.15</sub> × 10 <sup>-10</sup> | 1.07 <sup>+0.09</sup> <sub>-0.15</sub> × 10 <sup>-10</sup> | 229.1 / 186 |
| 39.519                    | 0.11 <sup>+0.01</sup> <sub>-0.01</sub>                 | 80.8 <sup>+0.8</sup> <sub>-0.1</sub>  | 1.142 <sup>+0.271</sup> <sub>-0.162</sub> | 1.545 <sup>+0.380</sup> <sub>-0.154</sub> | 1.85 <sup>+0.02</sup> <sub>-0.01</sub> × 10 <sup>-9</sup>  | 6.34 <sup>+0.55</sup> <sub>-0.55</sub> × 10 <sup>-11</sup> | 223.1 / 181 |
| 39.718                    | 0.08 <sup>+0.01</sup> <sub>-0.01</sub>                 | 76.1 <sup>+4.8</sup> <sub>-3.1</sub>  | 1.015 <sup>+0.068</sup> <sub>-0.077</sub> | 2.036 <sup>+0.714</sup> <sub>-0.404</sub> | 1.77 <sup>+0.02</sup> <sub>-0.01</sub> × 10 <sup>-9</sup>  | 6.17 <sup>+0.71</sup> <sub>-0.65</sub> × 10 <sup>-11</sup> | 212.6 / 162 |
| 39.786                    | 0.04 <sup>+0.01</sup> <sub>-0.01</sub>                 | 96.2 <sup>+4.2</sup> <sub>-17.1</sub> | 0.431 <sup>+0.267</sup> <sub>-0.178</sub> | 1.443 <sup>+0.096</sup> <sub>-0.079</sub> | 1.56 <sup>+0.01</sup> <sub>-0.01</sub> × 10 <sup>-9</sup>  | 7.08 <sup>+2.04</sup> <sub>-1.00</sub> × 10 <sup>-11</sup> | 255.5 / 172 |
| 39.92                     | 0.00 <sup>+0.07</sup> <sub>-0.01</sub>                 | 66.6 <sup>+1.3</sup> <sub>-2.1</sub>  | 0.313 <sup>+0.075</sup> <sub>-0.051</sub> | 1.719 <sup>+0.243</sup> <sub>-0.171</sub> | 3.66 <sup>+0.21</sup> <sub>-0.05</sub> × 10 <sup>-10</sup> | 9.56 <sup>+0.67</sup> <sub>-0.57</sub> × 10 <sup>-11</sup> | 182.6 / 175 |
| 40.053                    | 0.00 <sup>+0.02</sup> <sub>-0.01</sub>                 | 66.5 <sup>+1.2</sup> <sub>-2.9</sub>  | 0.533 <sup>+0.065</sup> <sub>-0.094</sub> | 1.785 <sup>+0.243</sup> <sub>-0.171</sub> | 3.09 <sup>+0.15</sup> <sub>-0.13</sub> × 10 <sup>-10</sup> | 8.97 <sup>+2.06</sup> <sub>-1.32</sub> × 10 <sup>-11</sup> | 150.6 / 175 |
| 40.121                    | 0.13 <sup>+0.02</sup> <sub>-0.02</sub>                 | 92.3 <sup>+7.9</sup> <sub>-3.1</sub>  | 0.433 <sup>+0.062</sup> <sub>-0.054</sub> | 1.929 <sup>+0.507</sup> <sub>-0.249</sub> | 1.67 <sup>+0.02</sup> <sub>-0.01</sub> × 10 <sup>-9</sup>  | 8.44 <sup>+1.15</sup> <sub>-1.19</sub> × 10 <sup>-11</sup> | 175.3 / 182 |
| 40.258                    | 0.12 <sup>+0.01</sup> <sub>-0.01</sub>                 | 81.7 <sup>+4.9</sup> <sub>-9.8</sub>  | 1.094 <sup>+0.064</sup> <sub>-0.061</sub> | 1.653 <sup>+0.166</sup> <sub>-0.132</sub> | 1.08 <sup>+0.01</sup> <sub>-0.01</sub> × 10 <sup>-9</sup>  | 6.74 <sup>+0.40</sup> <sub>-0.36</sub> × 10 <sup>-11</sup> | 342.6 / 227 |
| 40.339                    | 0.07 <sup>+0.01</sup> <sub>-0.01</sub>                 | 99.0 <sup>+1.4</sup> <sub>-12.1</sub> | 0.456 <sup>+0.192</sup> <sub>-0.077</sub> | 1.724 <sup>+0.123</sup> <sub>-0.103</sub> | 1.70 <sup>+0.01</sup> <sub>-0.01</sub> × 10 <sup>-9</sup>  | 7.27 <sup>+1.02</sup> <sub>-0.74</sub> × 10 <sup>-11</sup> | 352.6 / 230 |
| 40.728                    | 0.06 <sup>+0.02</sup> <sub>-0.02</sub>                 | 79.5 <sup>+9.4</sup> <sub>-9.1</sub>  | 0.431 <sup>+0.040</sup> <sub>-0.040</sub> | 1.714 <sup>+0.075</sup> <sub>-0.120</sub> | 3.93 <sup>+0.11</sup> <sub>-0.06</sub> × 10 <sup>-10</sup> | 8.73 <sup>+0.77</sup> <sub>-0.69</sub> × 10 <sup>-11</sup> | 344.9 / 217 |
| 40.793                    | 0.13 <sup>+0.03</sup> <sub>-0.03</sub>                 | 74.2 <sup>+7.5</sup> <sub>-7.5</sub>  | —                                         | 1.646 <sup>+0.032</sup> <sub>-0.032</sub> | 1.49 <sup>+0.01</sup> <sub>-0.01</sub> × 10 <sup>-9</sup>  | 7.30 <sup>+0.65</sup> <sub>-0.61</sub> × 10 <sup>-11</sup> | 428.6 / 218 |
| 40.861                    | 0.19 <sup>+0.01</sup> <sub>-0.02</sub>                 | 83.0 <sup>+4.8</sup> <sub>-8.7</sub>  | 0.971 <sup>+0.089</sup> <sub>-0.109</sub> | 1.679 <sup>+0.107</sup> <sub>-0.106</sub> | 1.67 <sup>+0.01</sup> <sub>-0.01</sub> × 10 <sup>-9</sup>  | 6.96 <sup>+0.37</sup> <sub>-0.44</sub> × 10 <sup>-11</sup> | 59.0 / 60   |
| 40.927                    | 0.33 <sup>+0.01</sup> <sub>-0.01</sub>                 | 58.8 <sup>+0.8</sup> <sub>-0.2</sub>  | 0.473 <sup>+0.654</sup> <sub>-0.473</sub> | 1.275 <sup>+0.081</sup> <sub>-0.043</sub> | 3.16 <sup>+0.01</sup> <sub>-0.01</sub> × 10 <sup>-9</sup>  | 6.01 <sup>+0.33</sup> <sub>-0.29</sub> × 10 <sup>-11</sup> | 78.6 / 91   |
| 40.994                    | 0.35 <sup>+0.01</sup> <sub>-0.02</sub>                 | 61.4 <sup>+3.4</sup> <sub>-0.8</sub>  | 0.457 <sup>+0.193</sup> <sub>-0.067</sub> | 1.299 <sup>+0.052</sup> <sub>-0.048</sub> | 3.80 <sup>+0.01</sup> <sub>-0.01</sub> × 10 <sup>-9</sup>  | 7.60 <sup>+0.89</sup> <sub>-0.76</sub> × 10 <sup>-11</sup> | 89.5 / 78   |
| 42.863                    | 0.26 <sup>+0.02</sup> <sub>-0.01</sub>                 | 69.4 <sup>+30.8</sup> <sub>-5.4</sub> | 1.148 <sup>+1.14</sup> <sub>-1.148</sub>  | —                                         | 2.91 <sup>+0.13</sup> <sub>-0.03</sub> × 10 <sup>-9</sup>  | 9.63 <sup>+3.48</sup> <sub>-3.15</sub> × 10 <sup>-11</sup> | 353.1 / 226 |
| 42.997                    | 0.33 <sup>+0.03</sup> <sub>-0.06</sub>                 | 76.1 <sup>+23.9</sup> <sub>-3.1</sub> | 0.406 <sup>+0.089</sup> <sub>-0.166</sub> | —                                         | 3.11 <sup>+0.07</sup> <sub>-0.02</sub> × 10 <sup>-9</sup>  | 7.18 <sup>+2.55</sup> <sub>-2.15</sub> × 10 <sup>-11</sup> | 291.1 / 215 |
| 43.064                    | 0.29 <sup>+0.01</sup> <sub>-0.02</sub>                 | 70.7 <sup>+1.4</sup> <sub>-0.7</sub>  | —                                         | 1.385 <sup>+1.117</sup> <sub>-0.195</sub> | 2.42 <sup>+0.08</sup> <sub>-0.06</sub> × 10 <sup>-9</sup>  | 6.40 <sup>+2.64</sup> <sub>-2.19</sub> × 10 <sup>-11</sup> | 391.6 / 252 |
| 43.204                    | 0.55 <sup>+0.04</sup> <sub>-0.06</sub>                 | 44.0 <sup>+1.5</sup> <sub>-0.7</sub>  | 0.848 <sup>+0.180</sup> <sub>-0.223</sub> | —                                         | 2.73 <sup>+0.06</sup> <sub>-0.08</sub> × 10 <sup>-9</sup>  | 1.15 <sup>+0.96</sup> <sub>-0.87</sub> × 10 <sup>-10</sup> | 35.8 / 62   |
| 43.67                     | 0.48 <sup>+0.03</sup> <sub>-0.02</sub>                 | 42.1 <sup>+2.0</sup> <sub>-2.6</sub>  | 0.535 <sup>+0.049</sup> <sub>-0.082</sub> | 1.322 <sup>+0.278</sup> <sub>-0.105</sub> | 2.23 <sup>+0.01</sup> <sub>-0.01</sub> × 10 <sup>-9</sup>  | 6.65 <sup>+0.74</sup> <sub>-0.62</sub> × 10 <sup>-11</sup> | 197.3 / 197 |
| 43.742                    | 0.31 <sup>+0.02</sup> <sub>-0.02</sub>                 | 46.0 <sup>+2.3</sup> <sub>-1.1</sub>  | 0.931 <sup>+0.071</sup> <sub>-0.123</sub> | 1.462 <sup>+0.133</sup> <sub>-0.076</sub> | 2.36 <sup>+0.01</sup> <sub>-0.01</sub> × 10 <sup>-9</sup>  | 5.76 <sup>+1.78</sup> <sub>-0.30</sub> × 10 <sup>-11</sup> | 317.1 / 234 |
| 43.807                    | 0.36 <sup>+0.02</sup> <sub>-0.02</sub>                 | 60.2 <sup>+2.3</sup> <sub>-0.7</sub>  | 0.482 <sup>+0.045</sup> <sub>-0.043</sub> | 1.457 <sup>+0.124</sup> <sub>-0.088</sub> | 1.76 <sup>+0.01</sup> <sub>-0.01</sub> × 10 <sup>-9</sup>  | 6.56 <sup>+0.36</sup> <sub>-0.45</sub> × 10 <sup>-11</sup> | 263.1 / 228 |
| 43.874                    | 0.29 <sup>+0.03</sup> <sub>-0.01</sub>                 | 63.3 <sup>+3.2</sup> <sub>-2.9</sub>  | 0.460 <sup>+0.065</sup> <sub>-0.039</sub> | 1.476 <sup>+0.140</sup> <sub>-0.107</sub> | 1.76 <sup>+0.01</sup> <sub>-0.01</sub> × 10 <sup>-9</sup>  | 7.15 <sup>+0.49</sup> <sub>-0.65</sub> × 10 <sup>-11</sup> | 343.3 / 231 |
| 43.941                    | 0.40 <sup>+0.01</sup> <sub>-0.01</sub>                 | 52.3 <sup>+0.1</sup> <sub>-0.1</sub>  | 0.434 <sup>+0.053</sup> <sub>-0.036</sub> | 1.325 <sup>+0.350</sup> <sub>-0.089</sub> | 2.32 <sup>+0.01</sup> <sub>-0.01</sub> × 10 <sup>-9</sup>  | 6.02 <sup>+1.21</sup> <sub>-0.57</sub> × 10 <sup>-11</sup> | 304.3 / 224 |
| 44.008                    | 0.18 <sup>+0.03</sup> <sub>-0.01</sub>                 | 65.9 <sup>+0.4</sup> <sub>-0.4</sub>  | 1.024 <sup>+0.049</sup> <sub>-0.058</sub> | 1.719 <sup>+0.169</sup> <sub>-0.149</sub> | 1.44 <sup>+0.01</sup> <sub>-0.01</sub> × 10 <sup>-9</sup>  | 5.88 <sup>+0</sup>                                         |             |

Table 2 – continued from previous page

| T <sub>mid</sub><br>(day) | N <sub>H</sub><br>(10 <sup>22</sup> cm <sup>-2</sup> ) | kT <sub>BB</sub><br>(eV)              | APEC kT <sub>cool</sub><br>(keV)          | APEC kT <sub>hot</sub><br>(keV)           | BB Flux<br>(erg cm <sup>-2</sup> s <sup>-1</sup> )         | APEC Flux<br>(erg cm <sup>-2</sup> s <sup>-1</sup> )       | Cstat/dof   |
|---------------------------|--------------------------------------------------------|---------------------------------------|-------------------------------------------|-------------------------------------------|------------------------------------------------------------|------------------------------------------------------------|-------------|
| 44.877                    | 0.45 <sup>+0.01</sup> <sub>-0.02</sub>                 | 44.1 <sup>+0.4</sup> <sub>-0.6</sub>  | 0.524 <sup>+0.102</sup> <sub>-0.104</sub> | 1.410 <sup>+0.135</sup> <sub>-0.113</sub> | 3.05 <sup>+0.02</sup> <sub>-0.01</sub> × 10 <sup>-9</sup>  | 4.88 <sup>+0.29</sup> <sub>-0.82</sub> × 10 <sup>-11</sup> | 274.6 / 183 |
| 44.944                    | 0.46 <sup>+0.02</sup> <sub>-0.04</sub>                 | 36.4 <sup>+0.1</sup> <sub>-2.2</sub>  | 0.504 <sup>+0.175</sup> <sub>-0.255</sub> | 0.977 <sup>+0.062</sup> <sub>-0.065</sub> | 2.84 <sup>+0.02</sup> <sub>-0.01</sub> × 10 <sup>-9</sup>  | 4.32 <sup>+1.00</sup> <sub>-0.41</sub> × 10 <sup>-11</sup> | 323.3 / 178 |
| 45.012                    | 0.48 <sup>+0.03</sup> <sub>-0.03</sub>                 | 52.1 <sup>+0.4</sup> <sub>-0.7</sub>  | 0.460 <sup>+0.094</sup> <sub>-0.083</sub> | 1.265 <sup>+0.231</sup> <sub>-0.074</sub> | 2.82 <sup>+0.01</sup> <sub>-0.01</sub> × 10 <sup>-9</sup>  | 4.97 <sup>+0.61</sup> <sub>-0.54</sub> × 10 <sup>-11</sup> | 321.1 / 195 |
| 45.079                    | 0.35 <sup>+0.01</sup> <sub>-0.01</sub>                 | 55.8 <sup>+0.2</sup> <sub>-0.1</sub>  | 1.148 <sup>+1.148</sup> <sub>-1.148</sub> | 1.263 <sup>+0.162</sup> <sub>-0.041</sub> | 4.01 <sup>+0.02</sup> <sub>-0.01</sub> × 10 <sup>-9</sup>  | 4.75 <sup>+0.35</sup> <sub>-0.26</sub> × 10 <sup>-11</sup> | 377.8 / 191 |
| 45.144                    | 0.36 <sup>+0.01</sup> <sub>-0.02</sub>                 | 54.5 <sup>+1.5</sup> <sub>-0.1</sub>  | —                                         | 1.249 <sup>+1.036</sup> <sub>-1.036</sub> | 4.11 <sup>+0.03</sup> <sub>-0.01</sub> × 10 <sup>-9</sup>  | 6.47 <sup>+0.40</sup> <sub>-0.32</sub> × 10 <sup>-11</sup> | 340.0 / 191 |
| 45.214                    | 0.46 <sup>+0.02</sup> <sub>-0.02</sub>                 | 56.1 <sup>+2.8</sup> <sub>-3.3</sub>  | —                                         | 1.125 <sup>+0.128</sup> <sub>-0.098</sub> | 4.28 <sup>+0.034</sup> <sub>-0.01</sub> × 10 <sup>-9</sup> | 5.17 <sup>+0.91</sup> <sub>-0.66</sub> × 10 <sup>-11</sup> | 185.8 / 138 |
| 45.676                    | 0.48 <sup>+0.01</sup> <sub>-0.05</sub>                 | 51.2 <sup>+0.6</sup> <sub>-1.0</sub>  | 0.429 <sup>+0.087</sup> <sub>-0.087</sub> | 1.631 <sup>+2.337</sup> <sub>-0.523</sub> | 3.89 <sup>+0.05</sup> <sub>-0.01</sub> × 10 <sup>-9</sup>  | 6.66 <sup>+1.26</sup> <sub>-1.25</sub> × 10 <sup>-11</sup> | 117.8 / 123 |
| 45.743                    | 0.27 <sup>+0.01</sup> <sub>-0.03</sub>                 | 53.5 <sup>+6.9</sup> <sub>-0.1</sub>  | 0.721 <sup>+0.253</sup> <sub>-0.146</sub> | 1.474 <sup>+0.237</sup> <sub>-0.162</sub> | 3.19 <sup>+0.04</sup> <sub>-0.01</sub> × 10 <sup>-9</sup>  | 6.75 <sup>+1.86</sup> <sub>-1.66</sub> × 10 <sup>-11</sup> | 145.2 / 138 |
| 45.815                    | 0.43 <sup>+0.01</sup> <sub>-0.01</sub>                 | 53.6 <sup>+0.9</sup> <sub>-0.4</sub>  | 0.434 <sup>+0.066</sup> <sub>-0.054</sub> | 1.301 <sup>+0.084</sup> <sub>-0.046</sub> | 3.85 <sup>+0.02</sup> <sub>-0.01</sub> × 10 <sup>-9</sup>  | 5.49 <sup>+0.30</sup> <sub>-0.27</sub> × 10 <sup>-11</sup> | 354.6 / 218 |
| 45.881                    | 0.39 <sup>+0.03</sup> <sub>-0.01</sub>                 | 51.6 <sup>+0.7</sup> <sub>-0.5</sub>  | 0.463 <sup>+0.077</sup> <sub>-0.121</sub> | 1.191 <sup>+0.065</sup> <sub>-0.060</sub> | 3.69 <sup>+0.02</sup> <sub>-0.01</sub> × 10 <sup>-9</sup>  | 5.49 <sup>+0.46</sup> <sub>-0.54</sub> × 10 <sup>-11</sup> | 366.3 / 200 |
| 45.949                    | 0.40 <sup>+0.01</sup> <sub>-0.01</sub>                 | 54.1 <sup>+2.4</sup> <sub>-0.8</sub>  | —                                         | 1.213 <sup>+0.061</sup> <sub>-0.043</sub> | 3.67 <sup>+0.01</sup> <sub>-0.01</sub> × 10 <sup>-9</sup>  | 5.53 <sup>+0.43</sup> <sub>-0.40</sub> × 10 <sup>-11</sup> | 380.2 / 214 |
| 46.082                    | 0.49 <sup>+0.01</sup> <sub>-0.01</sub>                 | 49.7 <sup>+0.3</sup> <sub>-0.5</sub>  | 0.433 <sup>+0.063</sup> <sub>-0.047</sub> | 1.348 <sup>+0.086</sup> <sub>-0.074</sub> | 3.82 <sup>+0.01</sup> <sub>-0.01</sub> × 10 <sup>-9</sup>  | 4.79 <sup>+0.36</sup> <sub>-0.19</sub> × 10 <sup>-11</sup> | 353.7 / 211 |
| 46.149                    | 0.40 <sup>+0.01</sup> <sub>-0.01</sub>                 | 52.5 <sup>+1.7</sup> <sub>-0.9</sub>  | 0.409 <sup>+0.066</sup> <sub>-0.058</sub> | 1.306 <sup>+0.165</sup> <sub>-0.098</sub> | 3.69 <sup>+0.02</sup> <sub>-0.01</sub> × 10 <sup>-9</sup>  | 5.89 <sup>+0.39</sup> <sub>-0.79</sub> × 10 <sup>-11</sup> | 303.9 / 203 |
| 46.55                     | 0.51 <sup>+0.01</sup> <sub>-0.01</sub>                 | 51.1 <sup>+1.0</sup> <sub>-1.6</sub>  | 0.434 <sup>+0.072</sup> <sub>-0.058</sub> | 1.199 <sup>+0.080</sup> <sub>-0.069</sub> | 4.10 <sup>+0.02</sup> <sub>-0.01</sub> × 10 <sup>-9</sup>  | 5.48 <sup>+0.66</sup> <sub>-0.34</sub> × 10 <sup>-11</sup> | 311.2 / 178 |
| 46.752                    | 0.30 <sup>+0.01</sup> <sub>-0.01</sub>                 | 59.0 <sup>+0.5</sup> <sub>-0.2</sub>  | 0.432 <sup>+0.069</sup> <sub>-0.056</sub> | 1.288 <sup>+0.075</sup> <sub>-0.074</sub> | 3.48 <sup>+0.02</sup> <sub>-0.01</sub> × 10 <sup>-9</sup>  | 5.20 <sup>+0.31</sup> <sub>-0.31</sub> × 10 <sup>-11</sup> | 379.9 / 188 |
| 47.154                    | 0.46 <sup>+0.01</sup> <sub>-0.01</sub>                 | 53.5 <sup>+1.9</sup> <sub>-1.3</sub>  | 0.456 <sup>+0.035</sup> <sub>-0.052</sub> | 1.367 <sup>+0.142</sup> <sub>-0.098</sub> | 4.26 <sup>+0.02</sup> <sub>-0.01</sub> × 10 <sup>-9</sup>  | 6.89 <sup>+0.34</sup> <sub>-0.35</sub> × 10 <sup>-11</sup> | 354.5 / 200 |
| 47.555                    | 0.41 <sup>+0.01</sup> <sub>-0.01</sub>                 | 55.5 <sup>+4.3</sup> <sub>-0.7</sub>  | 0.454 <sup>+0.070</sup> <sub>-0.068</sub> | 1.375 <sup>+0.193</sup> <sub>-0.109</sub> | 4.49 <sup>+0.05</sup> <sub>-0.01</sub> × 10 <sup>-9</sup>  | 5.96 <sup>+0.50</sup> <sub>-0.64</sub> × 10 <sup>-11</sup> | 189.8 / 153 |
| 47.89                     | 0.41 <sup>+0.02</sup> <sub>-0.01</sub>                 | 56.5 <sup>+1.6</sup> <sub>-3.3</sub>  | 0.436 <sup>+0.046</sup> <sub>-0.028</sub> | 1.367 <sup>+0.108</sup> <sub>-0.086</sub> | 4.07 <sup>+0.02</sup> <sub>-0.01</sub> × 10 <sup>-9</sup>  | 4.20 <sup>+0.25</sup> <sub>-0.24</sub> × 10 <sup>-11</sup> | 437.2 / 197 |
| 47.957                    | 0.37 <sup>+0.01</sup> <sub>-0.01</sub>                 | 56.5 <sup>+2.4</sup> <sub>-1.0</sub>  | 0.431 <sup>+0.030</sup> <sub>-0.033</sub> | 1.367 <sup>+0.181</sup> <sub>-0.087</sub> | 4.49 <sup>+0.02</sup> <sub>-0.01</sub> × 10 <sup>-9</sup>  | 7.20 <sup>+0.19</sup> <sub>-0.60</sub> × 10 <sup>-11</sup> | 412.7 / 196 |
| 48.091                    | 0.58 <sup>+0.01</sup> <sub>-0.01</sub>                 | 47.2 <sup>+2.0</sup> <sub>-2.3</sub>  | 0.433 <sup>+0.027</sup> <sub>-0.030</sub> | 1.091 <sup>+0.112</sup> <sub>-0.082</sub> | 4.13 <sup>+0.01</sup> <sub>-0.01</sub> × 10 <sup>-9</sup>  | 6.31 <sup>+0.33</sup> <sub>-0.30</sub> × 10 <sup>-11</sup> | 345.5 / 191 |
| 48.154                    | 0.48 <sup>+0.03</sup> <sub>-0.02</sub>                 | 57.4 <sup>+4.5</sup> <sub>-4.5</sub>  | 0.381 <sup>+0.062</sup> <sub>-0.081</sub> | —                                         | 3.72 <sup>+0.09</sup> <sub>-0.01</sub> × 10 <sup>-9</sup>  | 7.28 <sup>+1.72</sup> <sub>-1.99</sub> × 10 <sup>-11</sup> | 84.5 / 83   |
| 48.161                    | 0.50 <sup>+0.01</sup> <sub>-0.01</sub>                 | 53.4 <sup>+0.2</sup> <sub>-1.1</sub>  | 0.421 <sup>+0.047</sup> <sub>-0.049</sub> | 1.236 <sup>+0.137</sup> <sub>-0.082</sub> | 3.84 <sup>+0.02</sup> <sub>-0.01</sub> × 10 <sup>-9</sup>  | 6.00 <sup>+1.16</sup> <sub>-0.72</sub> × 10 <sup>-11</sup> | 208.7 / 166 |
| 48.233                    | 0.44 <sup>+0.01</sup> <sub>-0.01</sub>                 | 50.1 <sup>+1.7</sup> <sub>-1.3</sub>  | 0.432 <sup>+0.073</sup> <sub>-0.072</sub> | 1.107 <sup>+0.067</sup> <sub>-0.063</sub> | 3.74 <sup>+0.02</sup> <sub>-0.01</sub> × 10 <sup>-9</sup>  | 5.44 <sup>+0.50</sup> <sub>-0.56</sub> × 10 <sup>-11</sup> | 267.6 / 178 |
| 48.76                     | 0.35 <sup>+0.01</sup> <sub>-0.03</sub>                 | 52.4 <sup>+0.1</sup> <sub>-0.4</sub>  | 1.021 <sup>+0.094</sup> <sub>-0.094</sub> | 1.476 <sup>+0.338</sup> <sub>-0.065</sub> | 3.84 <sup>+0.01</sup> <sub>-0.01</sub> × 10 <sup>-9</sup>  | 4.37 <sup>+0.42</sup> <sub>-0.54</sub> × 10 <sup>-11</sup> | 382.0 / 197 |
| 48.827                    | 0.51 <sup>+0.01</sup> <sub>-0.01</sub>                 | 49.7 <sup>+0.3</sup> <sub>-0.5</sub>  | 0.431 <sup>+0.042</sup> <sub>-0.050</sub> | 1.217 <sup>+0.065</sup> <sub>-0.060</sub> | 3.91 <sup>+0.02</sup> <sub>-0.01</sub> × 10 <sup>-9</sup>  | 5.22 <sup>+0.46</sup> <sub>-0.44</sub> × 10 <sup>-11</sup> | 306.5 / 193 |
| 48.894                    | 0.41 <sup>+0.01</sup> <sub>-0.01</sub>                 | 53.4 <sup>+0.8</sup> <sub>-0.8</sub>  | 0.406 <sup>+0.065</sup> <sub>-0.061</sub> | 1.161 <sup>+0.052</sup> <sub>-0.048</sub> | 3.93 <sup>+0.01</sup> <sub>-0.03</sub> × 10 <sup>-9</sup>  | 4.72 <sup>+1.01</sup> <sub>-3.23</sub> × 10 <sup>-11</sup> | 412.8 / 197 |
| 48.962                    | 0.31 <sup>+0.01</sup> <sub>-0.02</sub>                 | 55.0 <sup>+0.7</sup> <sub>-0.7</sub>  | 0.430 <sup>+0.043</sup> <sub>-0.050</sub> | 1.233 <sup>+0.191</sup> <sub>-0.083</sub> | 3.40 <sup>+0.01</sup> <sub>-0.01</sub> × 10 <sup>-9</sup>  | 5.12 <sup>+0.70</sup> <sub>-0.48</sub> × 10 <sup>-11</sup> | 261.4 / 178 |
| 49.028                    | 0.38 <sup>+0.02</sup> <sub>-0.01</sub>                 | 55.1 <sup>+1.1</sup> <sub>-2.6</sub>  | 0.408 <sup>+0.040</sup> <sub>-0.031</sub> | 1.282 <sup>+0.083</sup> <sub>-0.079</sub> | 3.99 <sup>+0.02</sup> <sub>-0.01</sub> × 10 <sup>-9</sup>  | 6.90 <sup>+0.44</sup> <sub>-0.59</sub> × 10 <sup>-11</sup> | 373.2 / 206 |
| 49.095                    | 0.42 <sup>+0.01</sup> <sub>-0.01</sub>                 | 53.7 <sup>+2.7</sup> <sub>-0.5</sub>  | 0.442 <sup>+0.881</sup> <sub>-0.298</sub> | 1.158 <sup>+0.049</sup> <sub>-0.042</sub> | 3.70 <sup>+0.01</sup> <sub>-0.01</sub> × 10 <sup>-9</sup>  | 4.52 <sup>+0.24</sup> <sub>-0.23</sub> × 10 <sup>-11</sup> | 330.1 / 196 |
| 49.168                    | 0.42 <sup>+0.01</sup> <sub>-0.03</sub>                 | 50.2 <sup>+2.6</sup> <sub>-0.1</sub>  | 0.409 <sup>+0.048</sup> <sub>-0.031</sub> | 1.138 <sup>+0.058</sup> <sub>-0.067</sub> | 3.59 <sup>+0.01</sup> <sub>-0.01</sub> × 10 <sup>-9</sup>  | 5.18 <sup>+0.43</sup> <sub>-0.38</sub> × 10 <sup>-11</sup> | 309.0 / 194 |
| 49.494                    | 0.44 <sup>+0.01</sup> <sub>-0.01</sub>                 | 51.3 <sup>+0.3</sup> <sub>-0.3</sub>  | 0.442 <sup>+0.058</sup> <sub>-0.039</sub> | 1.295 <sup>+0.154</sup> <sub>-0.095</sub> | 4.61 <sup>+0.03</sup> <sub>-0.01</sub> × 10 <sup>-9</sup>  | 6.04 <sup>+1.43</sup> <sub>-0.41</sub> × 10 <sup>-11</sup> | 244.1 / 155 |
| 49.698                    | 0.48 <sup>+0.01</sup> <sub>-0.02</sub>                 | 53.5 <sup>+0.5</sup> <sub>-0.2</sub>  | 0.407 <sup>+0.089</sup> <sub>-0.097</sub> | 1.247 <sup>+0.066</sup> <sub>-0.057</sub> | 4.57 <sup>+0.02</sup> <sub>-0.01</sub> × 10 <sup>-9</sup>  | 4.87 <sup>+0.31</sup> <sub>-0.27</sub> × 10 <sup>-11</sup> | 332.0 / 189 |
| 49.827                    | 0.50 <sup>+0.06</sup> <sub>-0.10</sub>                 | 49.4 <sup>+10.7</sup> <sub>-2.5</sub> | —                                         | 0.907 <sup>+0.920</sup> <sub>-0.907</sub> | 4.51 <sup>+0.11</sup> <sub>-0.03</sub> × 10 <sup>-9</sup>  | 6.59 <sup>+2.84</sup> <sub>-3.06</sub> × 10 <sup>-11</sup> | 73.9 / 77   |
| 49.893                    | 0.42 <sup>+0.03</sup> <sub>-0.04</sub>                 | 70.8 <sup>+4.3</sup> <sub>-4.9</sub>  | —                                         | 1.228 <sup>+4.422</sup> <sub>-1.228</sub> | 4.42 <sup>+0.07</sup> <sub>-0.01</sub> × 10 <sup>-9</sup>  | 3.88 <sup>+1.12</sup> <sub>-0.74</sub> × 10 <sup>-11</sup> | 87.5 / 81   |
| 50.169                    | 0.37 <sup>+0.02</sup> <sub>-0.02</sub>                 | 59.5 <sup>+1.1</sup> <sub>-1.2</sub>  | 0.408 <sup>+0.059</sup> <sub>-0.052</sub> | 1.158 <sup>+0.161</sup> <sub>-0.106</sub> | 5.08 <sup>+0.04</sup> <sub>-0.01</sub> × 10 <sup>-9</sup>  | 6.56 <sup>+0.80</sup> <sub>-1.09</sub> × 10 <sup>-11</sup> | 217.3 / 132 |
| 50.499                    | 0.37 <sup>+0.01</sup> <sub>-0.03</sub>                 | 53.2 <sup>+0.1</sup> <sub>-0.1</sub>  | 0.433 <sup>+0.070</sup> <sub>-0.110</sub> | 1.257 <sup>+0.190</sup> <sub>-0.160</sub> | 4.30 <sup>+0.02</sup> <sub>-0.01</sub> × 10 <sup>-9</sup>  | 5.23 <sup>+0.68</sup> <sub>-1.30</sub> × 10 <sup>-11</sup> | 235.2 / 165 |
| 50.637                    | 0.46 <sup>+0.01</sup> <sub>-0.01</sub>                 | 51.6 <sup>+0.2</sup> <sub>-0.6</sub>  | 0.433 <sup>+0.040</sup> <sub>-0.030</sub> | 1.272 <sup>+0.056</sup> <sub>-0.066</sub> | 4.02 <sup>+0.02</sup> <sub>-0.01</sub> × 10 <sup>-9</sup>  | 5.29 <sup>+0.68</sup> <sub>-0.35</sub> × 10 <sup>-11</sup> | 381.6 / 204 |
| 50.702                    | 0.39 <sup>+0.01</sup> <sub>-0.01</sub>                 | 52.3 <sup>+0.5</sup> <sub>-0.4</sub>  | 0.432 <sup>+0.060</sup> <sub>-0.056</sub> | 1.150 <sup>+0.064</sup> <sub>-0.061</sub> | 4.03 <sup>+0.02</sup> <sub>-0.01</sub> × 10 <sup>-9</sup>  | 4.04 <sup>+0.35</sup> <sub>-0.18</sub> × 10 <sup>-11</sup> | 327.5 / 173 |
| 50.97                     | 0.55 <sup>+0.03</sup> <sub>-0.01</sub>                 | 47.6 <sup>+2.3</sup> <sub>-0.3</sub>  | 0.429 <sup>+0.031</sup> <sub>-0.044</sub> | 1.173 <sup>+0.129</sup> <sub>-0.103</sub> | 4.12 <sup>+0.02</sup> <sub>-0.01</sub> × 10 <sup>-9</sup>  | 4.96 <sup>+0.35</sup> <sub>-0.45</sub> × 10 <sup>-11</sup> | 302.3 / 180 |
| 51.037                    | 0.55 <sup>+0.02</sup> <sub>-0.02</sub>                 | 52.2 <sup>+1.1</sup> <sub>-1.6</sub>  | 0.412 <sup>+0.052</sup> <sub>-0.043</sub> | 1.220 <sup>+0.179</sup> <sub>-0.117</sub> | 4.56 <sup>+0.02</sup> <sub>-0.01</sub> × 10 <sup>-9</sup>  | 4.73 <sup>+0.44</sup> <sub>-0.30</sub> × 10 <sup>-11</sup> | 373.5 / 177 |
| 51.105                    | 0.38 <sup>+0.01</sup> <sub>-0.01</sub>                 | 54.5 <sup>+3.0</sup> <sub>-0.3</sub>  | 0.420 <sup>+0.026</sup> <sub>-0.022</sub> | 1.157 <sup>+0.146</sup> <sub>-0.094</sub> | 4.37 <sup>+0.03</sup> <sub>-0.01</sub> × 10 <sup>-9</sup>  | 6.18 <sup>+0.52</sup> <sub>-0.53</sub> × 10 <sup>-11</sup> | 348.4 / 156 |
| 51.174                    | 0.37 <sup>+0.01</sup> <sub>-0.02</sub>                 | 53.0 <sup>+1.6</sup> <sub>-0.5</sub>  | —                                         | 1.340 <sup>+1.470</sup> <sub>-1.150</sub> | 4.65 <sup>+0.08</sup> <sub>-0.01</sub> × 10 <sup>-9</sup>  | 4.59 <sup>+0.88</sup> <sub>-0.69</sub> × 10 <sup>-11</sup> | 123.0 / 113 |
| 51.185                    | 0.37 <sup>+0.01</sup> <sub>-0.02</sub>                 | 54.0 <sup>+0.1</sup> <sub>-0.1</sub>  | 0.434 <sup>+0.053</sup> <sub>-0.032</sub> | 1.352 <sup>+0.104</sup> <sub>-0.085</sub> | 4.82 <sup>+0.02</sup> <sub>-0.01</sub> × 10 <sup>-9</sup>  | 4.67 <sup>+0.58</sup> <sub>-0.36</sub> × 10 <sup>-11</sup> | 404.9 / 202 |
| 51.572                    | 0.56 <sup>+0.01</sup> <sub>-0.02</sub>                 | 49.5 <sup>+1.6</sup> <sub>-1.8</sub>  | 0.390 <sup>+0.049</sup> <sub>-0.041</sub> | 1.210 <sup>+0.108</sup> <sub>-0.113</sub> | 4.93 <sup>+0.02</sup> <sub>-0.01</sub> × 10 <sup>-9</sup>  | 6.84 <sup>+0.67</sup> <sub>-0.43</sub> × 10 <sup>-11</sup> | 338.9 / 180 |
| 51.638                    | 0.27 <sup>+0.03</sup> <sub>-0.02</sub>                 | 63.1 <sup>+2.5</sup> <sub>-3.4</sub>  | 0.382 <sup>+0.076</sup> <sub>-0.067</sub> | 1.516 <sup>+0.294</sup> <sub>-0.191</sub> | 5.19 <sup>+0.03</sup> <sub>-0.01</sub> × 10 <sup>-9</sup>  | 7.01 <sup>+0.98</sup> <sub>-0.56</sub> × 10 <sup>-11</sup> | 280.0 / 174 |
| 51.706                    | 0.31 <sup>+0.01</sup> <sub>-0.01</sub>                 | 57.6 <sup>+0.4</sup> <sub>-0.4</sub>  | 0.432 <sup>+0.077</sup> <sub>-0.186</sub> | 1.151 <sup>+0.081</sup> <sub>-0.077</sub> | 4.94 <sup>+0.03</sup> <sub>-0.01</sub> × 10 <sup>-9</sup>  | 6.95 <sup>+0.48</sup> <sub>-0.24</sub> × 10 <sup>-11</sup> | 237.5 / 166 |
| 51.772                    | 0.46 <sup>+0.01</sup> <sub>-0.01</sub>                 | 52.8 <sup>+1.5</sup> <sub>-0.2</sub>  | 0.455 <sup>+0.028</sup> <sub>-0.051</sub> | 1.094 <sup>+0.375</sup> <sub>-0.116</sub> | 4.59 <sup>+0.02</sup> <sub>-0.01</sub> × 10 <sup>-9</sup>  | 3.21 <sup>+0.65</sup> <sub>-0.47</sub> × 10 <sup>-11</sup> | 259.2 / 176 |
| 51.84                     | 0.49 <sup>+0.02</sup> <sub>-0.02</sub>                 | 49.7 <sup>+0.4</sup> <sub>-0.4</sub>  | 0.431 <sup>+0.067</sup> <sub>-0.060</sub> | 1.119 <sup>+0.135</sup> <sub>-0.141</sub> | 4.95 <sup>+0.03</sup> <sub>-0.01</sub> × 10 <sup>-9</sup>  | 5.72 <sup>+0.62</sup> <sub>-0.63</sub> × 10 <sup>-11</sup> | 247.7 / 169 |
| 52.11                     | 0.32 <sup>+0.01</sup> <sub>-0.01</sub>                 | 58.0 <sup>+0.8</sup> <sub>-0.8</sub>  | 0.430 <sup>+0.042</sup> <sub>-0.057</sub> | 1.228 <sup>+0.102</sup> <sub>-0.091</sub> | 4.99 <sup>+0.02</sup> <sub>-0.01</sub> × 10 <sup>-9</sup>  | 5.38 <sup>+0.61</sup> <sub>-0.51</sub> × 10 <sup>-11</sup> | 307.5 / 173 |
| 52.322                    | 0.36 <sup>+0.01</sup> <sub>-0.02</sub>                 | 55.3 <sup>+0.1</sup> <sub>-0.4</sub>  | 0.456 <sup>+0.038</sup> <sub>-0.039</sub> | 1.273 <sup>+0.051</sup> <sub>-0.075</sub> | 4.49 <sup>+0.03</sup> <sub>-0.01</sub> × 10 <sup>-9</sup>  | 5.80 <sup>+0.68</sup> <sub>-0.41</sub> × 10 <sup>-11</sup> | 395.4 / 194 |
| 52.393                    | 0.37 <sup>+0.01</sup> <sub>-0.01</sub>                 | 54.5 <sup>+0.4</sup> <sub>-0.1</sub>  | 0.433 <sup>+0.034</sup> <sub>-0.025</sub> | 1.322 <sup>+0.201</sup> <sub>-0.128</sub> | 4.42 <sup>+0.02</sup> <sub>-0.01</sub> × 10 <sup>-9</sup>  | 6.29 <sup>+0.51</sup> <sub>-0.47</sub> × 10 <sup>-11</sup> | 307.2 / 184 |
| 52.461                    | 0.50 <sup>+0.01</sup> <sub>-0.01</sub>                 | 53.1 <sup>+1.5</sup> <sub>-0.1</sub>  | 0.400 <sup>+0.034</sup> <sub>-0.034</sub> | 1.147 <sup>+0.087</sup> <sub>-0.086</sub> | 4.31 <sup>+0.02</sup> <sub>-0.01</sub> × 10 <sup>-9</sup>  | 6.04 <sup>+0.38</sup> <sub>-0.28</sub> × 10 <sup>-11</sup> | 318.0 / 173 |
| 52.576                    | 0.40 <sup>+0.03</sup> <sub>-0.03</sub>                 | 54.7 <sup>+0.5</sup> <sub>-0.3</sub>  | 1.148 <sup>+0.064</sup> <sub>-0.058</sub> | 0.431 <sup>+0.091</sup> <sub>-0.082</sub> | 4.42 <sup>+0.02</sup> <sub>-0.01</sub> × 10 <sup>-9</sup>  | 5.26 <sup>+0.45</sup> <sub>-0.29</sub> × 10 <sup>-11</sup> | 275.7 / 179 |
| 52.648                    | 0.41 <sup>+0.01</sup> <sub>-0.02</sub>                 | 52.9 <sup>+3.0</sup> <sub>-0.4</sub>  | 0.454 <sup>+0.016</sup> <sub>-0.040</sub> | 1.260 <sup>+0.107</sup> <sub>-0.089</sub> | 4.56 <sup>+0.01</sup> <sub>-0.01</sub> × 10 <sup>-9</sup>  | 6.20 <sup>+0.28</sup> <sub>-0.55</sub> × 10 <sup>-11</sup> | 448.4 / 213 |
| 52.715                    | 0.33 <sup>+0.01</sup> <sub>-0.01</sub>                 | 55.6 <sup>+0.6</sup> <sub>-0.1</sub>  | 0.433 <sup>+0.028</sup> <sub>-0.024</sub> | 1.351 <sup>+0.166</sup> <sub>-0.082</sub> | 4.45 <sup>+0.02</sup> <sub>-0.01</sub> × 10 <sup>-9</sup>  | 6.10 <sup>+0.46</sup> <sub>-0.26</sub> × 10 <sup>-11</sup> | 481.2 / 226 |
| 52.849                    | 0.26 <sup>+0.01</sup> <sub>-0.01</sub>                 | 58.8 <sup>+0.5</sup> <sub>-0.7</sub>  | 0.408 <sup>+0.035</sup> <sub>-0.031</sub> | 1.278 <sup>+0.082</sup> <sub>-0.065</sub> | 4.09 <sup>+0.02</sup> <sub>-0.01</sub> × 10 <sup>-9</sup>  | 5.61 <sup>+0.51</sup> <sub>-0.56</sub>                     |             |

Table 2 – continued from previous page

| T <sub>mid</sub><br>(day) | N <sub>H</sub><br>(10 <sup>22</sup> cm <sup>-2</sup> ) | kT <sub>BB</sub><br>(eV)              | APEC kT <sub>cool</sub><br>(keV)          | APEC kT <sub>hot</sub><br>(keV)           | BB Flux<br>(erg cm <sup>-2</sup> s <sup>-1</sup> )        | APEC Flux<br>(erg cm <sup>-2</sup> s <sup>-1</sup> )       | Cstat/dof   |
|---------------------------|--------------------------------------------------------|---------------------------------------|-------------------------------------------|-------------------------------------------|-----------------------------------------------------------|------------------------------------------------------------|-------------|
| 52.983                    | 0.37 <sup>+0.01</sup> <sub>-0.01</sub>                 | 52.9 <sup>+0.2</sup> <sub>-0.2</sub>  | 0.385 <sup>+0.026</sup> <sub>-0.025</sub> | 1.107 <sup>+0.056</sup> <sub>-0.047</sub> | 4.09 <sup>+0.02</sup> <sub>-0.01</sub> × 10 <sup>-9</sup> | 6.03 <sup>+0.51</sup> <sub>-0.37</sub> × 10 <sup>-11</sup> | 513.9 / 224 |
| 53.05                     | 0.33 <sup>+0.01</sup> <sub>-0.01</sub>                 | 55.4 <sup>+0.1</sup> <sub>-0.1</sub>  | 0.407 <sup>+0.029</sup> <sub>-0.036</sub> | 1.213 <sup>+0.055</sup> <sub>-0.061</sub> | 3.92 <sup>+0.01</sup> <sub>-0.01</sub> × 10 <sup>-9</sup> | 5.21 <sup>+0.44</sup> <sub>-0.49</sub> × 10 <sup>-11</sup> | 421.4 / 223 |
| 53.119                    | 0.38 <sup>+0.01</sup> <sub>-0.01</sub>                 | 52.7 <sup>+1.0</sup> <sub>-0.1</sub>  | 0.393 <sup>+0.040</sup> <sub>-0.031</sub> | 1.142 <sup>+0.053</sup> <sub>-0.051</sub> | 3.63 <sup>+0.01</sup> <sub>-0.01</sub> × 10 <sup>-9</sup> | 3.76 <sup>+0.19</sup> <sub>-0.19</sub> × 10 <sup>-11</sup> | 518.0 / 210 |
| 53.187                    | 0.63 <sup>+0.11</sup> <sub>-0.09</sub>                 | 49.4 <sup>+19.2</sup> <sub>-2.8</sub> | 0.430 <sup>+0.737</sup> <sub>-0.297</sub> | 1.373 <sup>+1.37</sup> <sub>-1.373</sub>  | 4.43 <sup>+0.17</sup> <sub>-0.01</sub> × 10 <sup>-9</sup> | 4.43 <sup>+2.34</sup> <sub>-1.66</sub> × 10 <sup>-11</sup> | 67.5 / 58   |
| 53.26                     | 0.49 <sup>+0.01</sup> <sub>-0.02</sub>                 | 48.9 <sup>+0.3</sup> <sub>-0.1</sub>  | 0.431 <sup>+0.033</sup> <sub>-0.033</sub> | 1.212 <sup>+0.059</sup> <sub>-0.060</sub> | 4.18 <sup>+0.01</sup> <sub>-0.01</sub> × 10 <sup>-9</sup> | 5.21 <sup>+0.23</sup> <sub>-0.47</sub> × 10 <sup>-11</sup> | 424.9 / 211 |
| 53.329                    | 0.44 <sup>+0.01</sup> <sub>-0.01</sub>                 | 50.9 <sup>+0.5</sup> <sub>-1.2</sub>  | 0.408 <sup>+0.049</sup> <sub>-0.046</sub> | 1.153 <sup>+0.077</sup> <sub>-0.067</sub> | 3.64 <sup>+0.02</sup> <sub>-0.01</sub> × 10 <sup>-9</sup> | 5.11 <sup>+0.33</sup> <sub>-0.37</sub> × 10 <sup>-11</sup> | 281.0 / 201 |
| 53.396                    | 0.43 <sup>+0.01</sup> <sub>-0.01</sub>                 | 51.3 <sup>+0.1</sup> <sub>-0.1</sub>  | 0.402 <sup>+0.029</sup> <sub>-0.029</sub> | 1.180 <sup>+0.165</sup> <sub>-0.111</sub> | 3.91 <sup>+0.01</sup> <sub>-0.01</sub> × 10 <sup>-9</sup> | 5.83 <sup>+0.50</sup> <sub>-0.42</sub> × 10 <sup>-11</sup> | 285.1 / 183 |
| 53.465                    | 0.63 <sup>+0.02</sup> <sub>-0.01</sub>                 | 43.1 <sup>+0.5</sup> <sub>-0.5</sub>  | 0.406 <sup>+0.045</sup> <sub>-0.026</sub> | 1.130 <sup>+0.213</sup> <sub>-0.151</sub> | 3.47 <sup>+0.02</sup> <sub>-0.01</sub> × 10 <sup>-9</sup> | 4.56 <sup>+0.42</sup> <sub>-0.37</sub> × 10 <sup>-11</sup> | 300.1 / 175 |
| 53.512                    | 0.40 <sup>+0.01</sup> <sub>-0.01</sub>                 | 53.4 <sup>+1.2</sup> <sub>-0.1</sub>  | 0.410 <sup>+0.071</sup> <sub>-0.054</sub> | 1.152 <sup>+0.200</sup> <sub>-0.118</sub> | 5.04 <sup>+0.04</sup> <sub>-0.01</sub> × 10 <sup>-9</sup> | 5.91 <sup>+1.56</sup> <sub>-0.79</sub> × 10 <sup>-11</sup> | 271.0 / 161 |
| 53.533                    | 0.73 <sup>+0.01</sup> <sub>-0.01</sub>                 | 42.4 <sup>+2.2</sup> <sub>-0.1</sub>  | 0.371 <sup>+0.033</sup> <sub>-0.041</sub> | 1.098 <sup>+0.179</sup> <sub>-0.124</sub> | 4.01 <sup>+0.02</sup> <sub>-0.01</sub> × 10 <sup>-9</sup> | 5.87 <sup>+0.55</sup> <sub>-0.41</sub> × 10 <sup>-11</sup> | 325.8 / 152 |
| 53.581                    | 0.38 <sup>+0.01</sup> <sub>-0.01</sub>                 | 53.5 <sup>+2.0</sup> <sub>-2.2</sub>  | 0.431 <sup>+0.063</sup> <sub>-0.045</sub> | 1.261 <sup>+0.324</sup> <sub>-0.170</sub> | 4.46 <sup>+0.03</sup> <sub>-0.01</sub> × 10 <sup>-9</sup> | 5.96 <sup>+0.75</sup> <sub>-0.67</sub> × 10 <sup>-11</sup> | 258.1 / 160 |
| 53.598                    | 0.29 <sup>+0.03</sup> <sub>-0.03</sub>                 | 59.3 <sup>+3.1</sup> <sub>-3.9</sub>  | 0.484 <sup>+0.079</sup> <sub>-0.073</sub> | 1.357 <sup>+0.809</sup> <sub>-0.345</sub> | 3.28 <sup>+0.01</sup> <sub>-0.01</sub> × 10 <sup>-9</sup> | 5.10 <sup>+0.46</sup> <sub>-0.54</sub> × 10 <sup>-11</sup> | 247.6 / 166 |
| 53.652                    | 0.30 <sup>+0.01</sup> <sub>-0.01</sub>                 | 56.8 <sup>+0.6</sup> <sub>-0.7</sub>  | 0.355 <sup>+0.037</sup> <sub>-0.037</sub> | 1.157 <sup>+0.061</sup> <sub>-0.061</sub> | 4.67 <sup>+0.02</sup> <sub>-0.01</sub> × 10 <sup>-9</sup> | 6.65 <sup>+0.60</sup> <sub>-0.93</sub> × 10 <sup>-11</sup> | 400.1 / 205 |
| 53.719                    | 0.43 <sup>+0.01</sup> <sub>-0.02</sub>                 | 50.8 <sup>+0.3</sup> <sub>-0.4</sub>  | 0.435 <sup>+0.032</sup> <sub>-0.027</sub> | 1.286 <sup>+0.262</sup> <sub>-0.338</sub> | 5.94 <sup>+0.02</sup> <sub>-0.01</sub> × 10 <sup>-9</sup> | 9.37 <sup>+0.58</sup> <sub>-0.38</sub> × 10 <sup>-11</sup> | 364.6 / 186 |
| 53.786                    | 0.41 <sup>+0.01</sup> <sub>-0.01</sub>                 | 51.3 <sup>+0.1</sup> <sub>-0.3</sub>  | 0.410 <sup>+0.028</sup> <sub>-0.020</sub> | 1.212 <sup>+0.108</sup> <sub>-0.092</sub> | 4.62 <sup>+0.01</sup> <sub>-0.01</sub> × 10 <sup>-9</sup> | 6.71 <sup>+0.44</sup> <sub>-0.52</sub> × 10 <sup>-11</sup> | 369.2 / 205 |
| 53.987                    | 0.28 <sup>+0.01</sup> <sub>-0.02</sub>                 | 57.0 <sup>+0.5</sup> <sub>-0.6</sub>  | 0.410 <sup>+0.025</sup> <sub>-0.028</sub> | 1.299 <sup>+0.126</sup> <sub>-0.086</sub> | 5.46 <sup>+0.02</sup> <sub>-0.01</sub> × 10 <sup>-9</sup> | 6.01 <sup>+0.66</sup> <sub>-0.56</sub> × 10 <sup>-11</sup> | 477.9 / 182 |
| 54.06                     | 0.31 <sup>+0.01</sup> <sub>-0.01</sub>                 | 54.7 <sup>+0.6</sup> <sub>-0.3</sub>  | —                                         | 1.152 <sup>+0.069</sup> <sub>-0.059</sub> | 3.84 <sup>+0.02</sup> <sub>-0.01</sub> × 10 <sup>-9</sup> | 3.42 <sup>+0.45</sup> <sub>-0.63</sub> × 10 <sup>-11</sup> | 302.4 / 158 |
| 54.125                    | 0.33 <sup>+0.01</sup> <sub>-0.01</sub>                 | 57.3 <sup>+1.1</sup> <sub>-2.0</sub>  | 0.408 <sup>+0.044</sup> <sub>-0.036</sub> | 1.163 <sup>+0.091</sup> <sub>-0.058</sub> | 4.64 <sup>+0.02</sup> <sub>-0.01</sub> × 10 <sup>-9</sup> | 4.32 <sup>+0.22</sup> <sub>-0.21</sub> × 10 <sup>-11</sup> | 503.9 / 198 |
| 54.199                    | 0.35 <sup>+0.01</sup> <sub>-0.02</sub>                 | 54.4 <sup>+0.1</sup> <sub>-0.1</sub>  | 0.410 <sup>+0.037</sup> <sub>-0.034</sub> | 1.211 <sup>+0.058</sup> <sub>-0.078</sub> | 4.47 <sup>+0.02</sup> <sub>-0.01</sub> × 10 <sup>-9</sup> | 6.21 <sup>+0.64</sup> <sub>-0.48</sub> × 10 <sup>-11</sup> | 302.9 / 184 |
| 54.265                    | 0.45 <sup>+0.01</sup> <sub>-0.01</sub>                 | 49.6 <sup>+0.8</sup> <sub>-0.8</sub>  | 0.425 <sup>+0.045</sup> <sub>-0.050</sub> | 1.086 <sup>+0.128</sup> <sub>-0.090</sub> | 4.45 <sup>+0.01</sup> <sub>-0.01</sub> × 10 <sup>-9</sup> | 5.29 <sup>+0.49</sup> <sub>-0.42</sub> × 10 <sup>-11</sup> | 309.7 / 195 |
| 54.334                    | 0.41 <sup>+0.01</sup> <sub>-0.01</sub>                 | 51.5 <sup>+2.5</sup> <sub>-0.1</sub>  | 0.425 <sup>+0.133</sup> <sub>-0.133</sub> | 1.148 <sup>+0.050</sup> <sub>-0.057</sub> | 4.33 <sup>+0.02</sup> <sub>-0.01</sub> × 10 <sup>-9</sup> | 4.61 <sup>+0.38</sup> <sub>-0.40</sub> × 10 <sup>-11</sup> | 341.3 / 189 |
| 54.47                     | 0.53 <sup>+0.01</sup> <sub>-0.01</sub>                 | 51.1 <sup>+1.5</sup> <sub>-3.2</sub>  | —                                         | 1.084 <sup>+0.041</sup> <sub>-0.057</sub> | 4.12 <sup>+0.02</sup> <sub>-0.01</sub> × 10 <sup>-9</sup> | 4.23 <sup>+0.43</sup> <sub>-0.21</sub> × 10 <sup>-11</sup> | 243.7 / 170 |
| 54.537                    | 0.58 <sup>+0.02</sup> <sub>-0.02</sub>                 | 49.7 <sup>+4.0</sup> <sub>-1.4</sub>  | 0.440 <sup>+0.055</sup> <sub>-0.050</sub> | 1.296 <sup>+0.207</sup> <sub>-0.122</sub> | 3.65 <sup>+0.02</sup> <sub>-0.01</sub> × 10 <sup>-9</sup> | 5.05 <sup>+0.37</sup> <sub>-0.78</sub> × 10 <sup>-11</sup> | 229.6 / 153 |
| 54.871                    | 0.45 <sup>+0.01</sup> <sub>-0.01</sub>                 | 48.8 <sup>+3.3</sup> <sub>-1.3</sub>  | 0.431 <sup>+0.032</sup> <sub>-0.044</sub> | 1.452 <sup>+0.267</sup> <sub>-0.199</sub> | 4.04 <sup>+0.02</sup> <sub>-0.01</sub> × 10 <sup>-9</sup> | 5.20 <sup>+0.51</sup> <sub>-0.39</sub> × 10 <sup>-11</sup> | 217.0 / 162 |
| 54.924                    | 0.33 <sup>+0.01</sup> <sub>-0.01</sub>                 | 55.7 <sup>+2.7</sup> <sub>-0.1</sub>  | 0.432 <sup>+0.031</sup> <sub>-0.026</sub> | 1.288 <sup>+0.109</sup> <sub>-0.099</sub> | 4.11 <sup>+0.01</sup> <sub>-0.01</sub> × 10 <sup>-9</sup> | 4.97 <sup>+0.48</sup> <sub>-0.33</sub> × 10 <sup>-11</sup> | 419.1 / 173 |
| 54.991                    | 0.47 <sup>+0.01</sup> <sub>-0.01</sub>                 | 48.4 <sup>+1.0</sup> <sub>-0.4</sub>  | 0.430 <sup>+0.071</sup> <sub>-0.070</sub> | 1.122 <sup>+0.062</sup> <sub>-0.055</sub> | 4.39 <sup>+0.02</sup> <sub>-0.01</sub> × 10 <sup>-9</sup> | 4.61 <sup>+0.30</sup> <sub>-0.33</sub> × 10 <sup>-11</sup> | 376.5 / 210 |
| 55.059                    | 0.41 <sup>+0.01</sup> <sub>-0.02</sub>                 | 50.4 <sup>+0.1</sup> <sub>-0.2</sub>  | 0.405 <sup>+0.086</sup> <sub>-0.165</sub> | 1.222 <sup>+0.048</sup> <sub>-0.045</sub> | 3.84 <sup>+0.01</sup> <sub>-0.01</sub> × 10 <sup>-9</sup> | 3.62 <sup>+0.25</sup> <sub>-0.16</sub> × 10 <sup>-11</sup> | 356.5 / 209 |
| 55.13                     | 0.32 <sup>+0.01</sup> <sub>-0.02</sub>                 | 54.8 <sup>+0.2</sup> <sub>-0.3</sub>  | 0.421 <sup>+0.023</sup> <sub>-0.023</sub> | 1.211 <sup>+0.066</sup> <sub>-0.073</sub> | 4.08 <sup>+0.01</sup> <sub>-0.01</sub> × 10 <sup>-9</sup> | 5.70 <sup>+0.35</sup> <sub>-0.46</sub> × 10 <sup>-11</sup> | 450.4 / 186 |
| 55.2                      | 0.62 <sup>+0.01</sup> <sub>-0.02</sub>                 | 46.9 <sup>+0.7</sup> <sub>-1.7</sub>  | 0.418 <sup>+0.042</sup> <sub>-0.040</sub> | 1.105 <sup>+0.133</sup> <sub>-0.099</sub> | 4.29 <sup>+0.01</sup> <sub>-0.01</sub> × 10 <sup>-9</sup> | 5.14 <sup>+0.37</sup> <sub>-0.25</sub> × 10 <sup>-11</sup> | 401.9 / 191 |
| 55.338                    | 0.41 <sup>+0.01</sup> <sub>-0.02</sub>                 | 51.6 <sup>+0.1</sup> <sub>-0.1</sub>  | 0.410 <sup>+0.036</sup> <sub>-0.063</sub> | 1.170 <sup>+0.081</sup> <sub>-0.063</sub> | 4.82 <sup>+0.02</sup> <sub>-0.01</sub> × 10 <sup>-9</sup> | 4.31 <sup>+0.32</sup> <sub>-0.26</sub> × 10 <sup>-11</sup> | 257.5 / 179 |
| 55.474                    | 0.71 <sup>+0.02</sup> <sub>-0.01</sub>                 | 42.7 <sup>+1.5</sup> <sub>-2.4</sub>  | 0.377 <sup>+0.039</sup> <sub>-0.039</sub> | 1.144 <sup>+0.177</sup> <sub>-0.157</sub> | 4.19 <sup>+0.02</sup> <sub>-0.01</sub> × 10 <sup>-9</sup> | 4.97 <sup>+0.51</sup> <sub>-0.26</sub> × 10 <sup>-11</sup> | 250.2 / 164 |
| 55.521                    | 0.33 <sup>+0.01</sup> <sub>-0.04</sub>                 | 54.9 <sup>+1.2</sup> <sub>-1.9</sub>  | —                                         | 1.077 <sup>+1.62</sup> <sub>-0.897</sub>  | 4.57 <sup>+0.04</sup> <sub>-0.01</sub> × 10 <sup>-9</sup> | 5.50 <sup>+1.20</sup> <sub>-1.28</sub> × 10 <sup>-11</sup> | 152.6 / 131 |
| 55.594                    | 0.46 <sup>+0.02</sup> <sub>-0.01</sub>                 | 49.5 <sup>+0.8</sup> <sub>-0.7</sub>  | 0.407 <sup>+0.040</sup> <sub>-0.050</sub> | 1.199 <sup>+0.127</sup> <sub>-0.107</sub> | 4.08 <sup>+0.01</sup> <sub>-0.01</sub> × 10 <sup>-9</sup> | 5.39 <sup>+0.45</sup> <sub>-0.35</sub> × 10 <sup>-11</sup> | 328.2 / 202 |
| 55.677                    | 0.49 <sup>+0.02</sup> <sub>-0.03</sub>                 | 50.6 <sup>+3.1</sup> <sub>-0.9</sub>  | 0.382 <sup>+0.070</sup> <sub>-0.062</sub> | 1.190 <sup>+2.878</sup> <sub>-0.238</sub> | 4.14 <sup>+0.04</sup> <sub>-0.01</sub> × 10 <sup>-9</sup> | 4.65 <sup>+0.92</sup> <sub>-0.88</sub> × 10 <sup>-11</sup> | 144.0 / 124 |
| 55.728                    | 0.39 <sup>+0.02</sup> <sub>-0.02</sub>                 | 53.3 <sup>+2.4</sup> <sub>-0.1</sub>  | 0.409 <sup>+0.039</sup> <sub>-0.030</sub> | 1.092 <sup>+0.084</sup> <sub>-0.071</sub> | 4.31 <sup>+0.01</sup> <sub>-0.01</sub> × 10 <sup>-9</sup> | 5.55 <sup>+0.46</sup> <sub>-0.42</sub> × 10 <sup>-11</sup> | 414.4 / 194 |
| 55.805                    | 0.58 <sup>+0.01</sup> <sub>-0.01</sub>                 | 48.2 <sup>+0.9</sup> <sub>-1.1</sub>  | 0.404 <sup>+0.032</sup> <sub>-0.035</sub> | 1.148 <sup>+0.093</sup> <sub>-0.087</sub> | 4.47 <sup>+0.02</sup> <sub>-0.01</sub> × 10 <sup>-9</sup> | 5.28 <sup>+0.35</sup> <sub>-0.25</sub> × 10 <sup>-11</sup> | 409.5 / 183 |
| 55.861                    | 0.62 <sup>+0.01</sup> <sub>-0.02</sub>                 | 44.0 <sup>+0.7</sup> <sub>-1.7</sub>  | 0.368 <sup>+0.035</sup> <sub>-0.023</sub> | 1.076 <sup>+0.087</sup> <sub>-0.116</sub> | 4.22 <sup>+0.02</sup> <sub>-0.01</sub> × 10 <sup>-9</sup> | 6.21 <sup>+0.23</sup> <sub>-0.33</sub> × 10 <sup>-11</sup> | 333.2 / 188 |
| 55.929                    | 0.37 <sup>+0.01</sup> <sub>-0.01</sub>                 | 53.1 <sup>+0.6</sup> <sub>-2.3</sub>  | 0.400 <sup>+0.024</sup> <sub>-0.028</sub> | 1.117 <sup>+0.083</sup> <sub>-0.080</sub> | 4.58 <sup>+0.01</sup> <sub>-0.01</sub> × 10 <sup>-9</sup> | 5.96 <sup>+0.35</sup> <sub>-0.21</sub> × 10 <sup>-11</sup> | 413.6 / 197 |
| 55.995                    | 0.65 <sup>+0.02</sup> <sub>-0.01</sub>                 | 45.4 <sup>+0.7</sup> <sub>-1.5</sub>  | 0.365 <sup>+0.028</sup> <sub>-0.023</sub> | 0.992 <sup>+0.067</sup> <sub>-0.067</sub> | 4.56 <sup>+0.02</sup> <sub>-0.01</sub> × 10 <sup>-9</sup> | 6.18 <sup>+0.34</sup> <sub>-0.38</sub> × 10 <sup>-11</sup> | 404.9 / 204 |
| 56.063                    | 0.37 <sup>+0.01</sup> <sub>-0.01</sub>                 | 53.1 <sup>+0.3</sup> <sub>-2.4</sub>  | 0.379 <sup>+0.056</sup> <sub>-0.073</sub> | 1.112 <sup>+0.082</sup> <sub>-0.083</sub> | 3.98 <sup>+0.01</sup> <sub>-0.01</sub> × 10 <sup>-9</sup> | 5.14 <sup>+0.56</sup> <sub>-0.34</sub> × 10 <sup>-11</sup> | 422.9 / 191 |
| 56.134                    | 0.38 <sup>+0.01</sup> <sub>-0.02</sub>                 | 52.7 <sup>+0.4</sup> <sub>-0.1</sub>  | 0.405 <sup>+0.054</sup> <sub>-0.055</sub> | 1.027 <sup>+0.060</sup> <sub>-0.057</sub> | 3.99 <sup>+0.01</sup> <sub>-0.01</sub> × 10 <sup>-9</sup> | 4.18 <sup>+0.26</sup> <sub>-0.27</sub> × 10 <sup>-11</sup> | 319.7 / 191 |
| 56.205                    | 0.42 <sup>+0.01</sup> <sub>-0.02</sub>                 | 50.8 <sup>+0.1</sup> <sub>-0.1</sub>  | 0.345 <sup>+0.034</sup> <sub>-0.032</sub> | 1.120 <sup>+0.060</sup> <sub>-0.062</sub> | 4.08 <sup>+0.01</sup> <sub>-0.01</sub> × 10 <sup>-9</sup> | 5.47 <sup>+0.75</sup> <sub>-0.43</sub> × 10 <sup>-11</sup> | 373.4 / 201 |
| 56.274                    | 0.47 <sup>+0.01</sup> <sub>-0.03</sub>                 | 49.6 <sup>+0.2</sup> <sub>-0.4</sub>  | 0.407 <sup>+0.034</sup> <sub>-0.045</sub> | 1.035 <sup>+0.115</sup> <sub>-0.105</sub> | 4.35 <sup>+0.02</sup> <sub>-0.01</sub> × 10 <sup>-9</sup> | 5.77 <sup>+0.43</sup> <sub>-0.41</sub> × 10 <sup>-11</sup> | 288.7 / 182 |
| 56.342                    | 0.57 <sup>+0.01</sup> <sub>-0.03</sub>                 | 45.0 <sup>+0.7</sup> <sub>-1.9</sub>  | 0.401 <sup>+0.041</sup> <sub>-0.048</sub> | 1.143 <sup>+0.153</sup> <sub>-0.098</sub> | 4.31 <sup>+0.04</sup> <sub>-0.01</sub> × 10 <sup>-9</sup> | 5.68 <sup>+0.44</sup> <sub>-0.42</sub> × 10 <sup>-11</sup> | 266.4 / 185 |
| 56.411                    | 0.49 <sup>+0.02</sup> <sub>-0.01</sub>                 | 48.4 <sup>+1.4</sup> <sub>-0.7</sub>  | 0.400 <sup>+0.046</sup> <sub>-0.034</sub> | 1.138 <sup>+0.275</sup> <sub>-0.184</sub> | 4.53 <sup>+0.02</sup> <sub>-0.01</sub> × 10 <sup>-9</sup> | 6.09 <sup>+0.56</sup> <sub>-0.43</sub> × 10 <sup>-11</sup> | 198.4 / 158 |
| 56.478                    | 0.47 <sup>+0.01</sup> <sub>-0.02</sub>                 | 48.3 <sup>+2.4</sup> <sub>-1.1</sub>  | 0.385 <sup>+0.053</sup> <sub>-0.057</sub> | 1.034 <sup>+0.107</sup> <sub>-0.062</sub> | 4.00 <sup>+0.02</sup> <sub>-0.01</sub> × 10 <sup>-9</sup> | 4.68 <sup>+0.91</sup> <sub>-0.53</sub> × 10 <sup>-11</sup> | 252.7 / 157 |
| 56.526                    | 0.28 <sup>+0.01</sup> <sub>-0.02</sub>                 | 59.5 <sup>+2.5</sup> <sub>-0.8</sub>  | 0.408 <sup>+0.053</sup> <sub>-0.030</sub> | 1.144 <sup>+1.531</sup> <sub>-0.228</sub> | 4.03 <sup>+0.03</sup> <sub>-0.01</sub> × 10 <sup>-9</sup> | 5.29 <sup>+0.85</sup> <sub>-0.79</sub> × 10 <sup>-11</sup> | 201.1 / 145 |
| 56.542                    | 0.47 <sup>+0.01</sup> <sub>-0.02</sub>                 | 48.6 <sup>+0.4</sup> <sub>-0.1</sub>  | 0.365 <sup>+0.038</sup> <sub>-0.034</sub> | 1.171 <sup>+0.157</sup> <sub>-0.090</sub> | 4.00 <sup>+0.01</sup> <sub>-0.01</sub> × 10 <sup>-9</sup> | 4.85 <sup>+1.10</sup> <sub>-0.40</sub> × 10 <sup>-11</sup> | 263.0 / 189 |
| 56.604                    | 0.44 <sup>+0.01</sup> <sub>-0.01</sub>                 | 49.2 <sup>+0.2</sup> <sub>-0.2</sub>  | 0.394 <sup>+0.041</sup> <sub>-0.043</sub> | 1.146 <sup>+0.054</sup> <sub>-0.154</sub> | 3.84 <sup>+0.01</sup> <sub>-0.01</sub> × 10 <sup>-9</sup> | 4.32 <sup>+0.51</sup> <sub>-0.26</sub> × 10 <sup>-11</sup> | 391.5 / 195 |
| 56.671                    | 0.51 <sup>+0.01</sup> <sub>-0.01</sub>                 | 46.6 <sup>+0.1</sup> <sub>-0.2</sub>  | 0.416 <sup>+0.040</sup> <sub>-0.033</sub> | 1.217 <sup>+0.082</sup> <sub>-0.082</sub> | 3.82 <sup>+0.01</sup> <sub>-0.01</sub> × 10 <sup>-9</sup> | 4.59 <sup>+0.21</sup> <sub>-0.35</sub> × 10 <sup>-11</sup> | 363.6 / 188 |
| 56.74                     | 0.55 <sup>+0.01</sup> <sub>-0.01</sub>                 | 46.5 <sup>+1.4</sup> <sub>-2.7</sub>  | 0.389 <sup>+0.036</sup> <sub>-0.033</sub> | 1.365 <sup>+0.154</sup> <sub>-0.108</sub> | 4.27 <sup>+0.03</sup> <sub>-0.01</sub> × 10 <sup>-9</sup> | 4.98 <sup>+0.31</sup> <sub>-0.48</sub> × 10 <sup>-11</sup> | 331.5 / 188 |
| 56.875                    | 0.32 <sup>+0.02</sup> <sub>-0.01</sub>                 | 55.7 <sup>+0.1</sup> <sub>-0.1</sub>  | 0.414 <sup>+0.145</sup> <sub>-0.136</sub> | 1.032 <sup>+0.096</sup> <sub>-0.071</sub> | 4.75 <sup>+0.03</sup> <sub>-0.01</sub> × 10 <sup>-9</sup> | 5.03 <sup>+1.03</sup> <sub>-0.70</sub> × 10 <sup>-11</sup> | 186.9 / 144 |
| 56.934                    | 0.43 <sup>+0.01</sup> <sub>-0.01</sub>                 | 49.2 <sup>+0.2</sup> <sub>-0.7</sub>  | 0.392 <sup>+0.064</sup> <sub>-0.019</sub> | 1.105 <sup>+0.053</sup> <sub>-0.066</sub> | 4.24 <sup>+0.02</sup> <sub>-0.01</sub> × 10 <sup>-9</sup> | 5.13 <sup>+0.42</sup> <sub>-0.39</sub> × 10 <sup>-11</sup> | 385.6 / 205 |
| 57                        | 0.43 <sup>+0.01</sup> <sub>-0.02</sub>                 | 49.8 <sup>+0.5</sup> <sub>-0.4</sub>  | 0.430 <sup>+0.033</sup> <sub>-0.034</sub> | 1.283 <sup>+0.149</sup> <sub>-0.109</sub> | 4.14 <sup>+0.02</sup> <sub>-0.01</sub> × 10 <sup>-9</sup> | 5.01 <sup>+0.57</sup> <sub>-0.40</sub> × 10 <sup>-11</sup> | 365.0 / 190 |
| 57.068                    | 0.51 <sup>+0.02</sup> <sub>-0.01</sub>                 | 48.6 <sup>+0.2</sup> <sub>-0.5</sub>  | 0.407 <sup>+0.042</sup> <sub>-0.039</sub> | 1.088 <sup>+0.059</sup> <sub>-0.053</sub> | 4.01 <sup>+0.01</sup> <sub>-0.01</sub> × 10 <sup>-9</sup> | 4.11 <sup>+0.30</sup> <sub>-0.31</sub> × 10 <sup>-11</sup> | 389.8 / 188 |
| 57.138                    | 0.48 <sup>+0.01</sup> <sub>-0.02</sub>                 | 48.6 <sup>+0.1</sup> <sub>-0.1</sub>  | 0.378 <sup>+0.026</sup> <sub>-0.026</sub> | 1.                                        |                                                           |                                                            |             |



Table 2 – continued from previous page

| T <sub>mid</sub><br>(day) | N <sub>H</sub><br>(10 <sup>22</sup> cm <sup>-2</sup> ) | kT <sub>BB</sub><br>(eV)              | APEC kT <sub>cool</sub><br>(keV)          | APEC kT <sub>hot</sub><br>(keV)            | BB Flux<br>(erg cm <sup>-2</sup> s <sup>-1</sup> )        | APEC Flux<br>(erg cm <sup>-2</sup> s <sup>-1</sup> )       | Cstat/dof    |
|---------------------------|--------------------------------------------------------|---------------------------------------|-------------------------------------------|--------------------------------------------|-----------------------------------------------------------|------------------------------------------------------------|--------------|
| 58.281                    | 0.38 <sup>+0.01</sup> <sub>-0.01</sub>                 | 51.3 <sup>+0.9</sup> <sub>-1.2</sub>  | 0.386 <sup>+0.060</sup> <sub>-0.044</sub> | 1.217 <sup>+0.261</sup> <sub>-0.132</sub>  | 4.29 <sup>+0.02</sup> <sub>-0.01</sub> × 10 <sup>-9</sup> | 3.83 <sup>+0.35</sup> <sub>-0.44</sub> × 10 <sup>-11</sup> | 295.2 / 165  |
| 58.812                    | 0.42 <sup>+0.01</sup> <sub>-0.01</sub>                 | 49.6 <sup>+2.2</sup> <sub>-0.1</sub>  | 0.457 <sup>+0.035</sup> <sub>-0.032</sub> | 1.295 <sup>+0.121</sup> <sub>-0.083</sub>  | 3.41 <sup>+0.01</sup> <sub>-0.01</sub> × 10 <sup>-9</sup> | 3.75 <sup>+0.29</sup> <sub>-0.17</sub> × 10 <sup>-11</sup> | 320.2 / 186  |
| 59.542                    | 0.50 <sup>+0.01</sup> <sub>-0.01</sub>                 | 46.9 <sup>+1.1</sup> <sub>-0.7</sub>  | 0.432 <sup>+0.030</sup> <sub>-0.027</sub> | 1.208 <sup>+0.164</sup> <sub>-0.153</sub>  | 4.11 <sup>+0.02</sup> <sub>-0.01</sub> × 10 <sup>-9</sup> | 4.89 <sup>+0.33</sup> <sub>-0.22</sub> × 10 <sup>-11</sup> | 205.5 / 170  |
| 61.293                    | 0.39 <sup>+0.01</sup> <sub>-0.02</sub>                 | 50.2 <sup>+0.3</sup> <sub>-0.6</sub>  | 0.415 <sup>+0.031</sup> <sub>-0.040</sub> | —                                          | 3.49 <sup>+0.02</sup> <sub>-0.01</sub> × 10 <sup>-9</sup> | 5.13 <sup>+0.35</sup> <sub>-0.54</sub> × 10 <sup>-11</sup> | 259.7 / 156  |
| 61.358                    | 0.42 <sup>+0.02</sup> <sub>-0.03</sub>                 | 52.9 <sup>+1.5</sup> <sub>-3.5</sub>  | 0.352 <sup>+0.034</sup> <sub>-0.034</sub> | —                                          | 3.59 <sup>+0.02</sup> <sub>-0.01</sub> × 10 <sup>-9</sup> | 5.33 <sup>+0.60</sup> <sub>-0.96</sub> × 10 <sup>-11</sup> | 133.6 / 142  |
| 61.83                     | 0.41 <sup>+0.02</sup> <sub>-0.02</sub>                 | 49.1 <sup>+0.6</sup> <sub>-0.8</sub>  | 0.360 <sup>+0.052</sup> <sub>-0.044</sub> | 1.092 <sup>+0.277</sup> <sub>-0.147</sub>  | 4.04 <sup>+0.01</sup> <sub>-0.01</sub> × 10 <sup>-9</sup> | 5.04 <sup>+0.55</sup> <sub>-0.63</sub> × 10 <sup>-11</sup> | 158.9 / 139  |
| 61.897                    | 0.45 <sup>+0.02</sup> <sub>-0.01</sub>                 | 47.9 <sup>+0.1</sup> <sub>-0.7</sub>  | 0.346 <sup>+0.040</sup> <sub>-0.028</sub> | 0.918 <sup>+0.549</sup> <sub>-0.268</sub>  | 3.34 <sup>+0.02</sup> <sub>-0.01</sub> × 10 <sup>-9</sup> | 4.62 <sup>+0.55</sup> <sub>-0.49</sub> × 10 <sup>-11</sup> | 179.3 / 138  |
| 62.231                    | 0.35 <sup>+0.01</sup> <sub>-0.01</sub>                 | 54.1 <sup>+0.2</sup> <sub>-0.2</sub>  | 0.387 <sup>+0.056</sup> <sub>-0.040</sub> | 1.087 <sup>+0.205</sup> <sub>-0.219</sub>  | 3.79 <sup>+0.02</sup> <sub>-0.01</sub> × 10 <sup>-9</sup> | 5.32 <sup>+0.63</sup> <sub>-0.38</sub> × 10 <sup>-11</sup> | 209.0 / 136  |
| 62.298                    | 0.39 <sup>+0.01</sup> <sub>-0.03</sub>                 | 52.2 <sup>+2.7</sup> <sub>-0.1</sub>  | 0.378 <sup>+0.058</sup> <sub>-0.047</sub> | 1.147 <sup>+0.216</sup> <sub>-0.116</sub>  | 3.97 <sup>+0.02</sup> <sub>-0.01</sub> × 10 <sup>-9</sup> | 4.79 <sup>+0.72</sup> <sub>-0.59</sub> × 10 <sup>-11</sup> | 183.2 / 152  |
| 62.836                    | 0.50 <sup>+0.01</sup> <sub>-0.03</sub>                 | 44.5 <sup>+1.3</sup> <sub>-2.9</sub>  | 0.274 <sup>+0.040</sup> <sub>-0.028</sub> | 1.048 <sup>+0.177</sup> <sub>-0.115</sub>  | 3.82 <sup>+0.02</sup> <sub>-0.01</sub> × 10 <sup>-9</sup> | 6.21 <sup>+0.96</sup> <sub>-0.80</sub> × 10 <sup>-11</sup> | 182.0 / 148  |
| 62.902                    | 0.48 <sup>+0.04</sup> <sub>-0.01</sub>                 | 45.7 <sup>+0.2</sup> <sub>-0.5</sub>  | 0.365 <sup>+0.050</sup> <sub>-0.049</sub> | 1.280 <sup>+0.408</sup> <sub>-0.432</sub>  | 3.44 <sup>+0.02</sup> <sub>-0.01</sub> × 10 <sup>-9</sup> | 4.25 <sup>+0.61</sup> <sub>-0.60</sub> × 10 <sup>-11</sup> | 172.9 / 132  |
| 63.169                    | 0.41 <sup>+0.05</sup> <sub>-0.01</sub>                 | 50.7 <sup>+6.1</sup> <sub>-0.2</sub>  | 0.151 <sup>+0.048</sup> <sub>-0.151</sub> | 1.028 <sup>+0.141</sup> <sub>-0.083</sub>  | 3.36 <sup>+0.01</sup> <sub>-0.01</sub> × 10 <sup>-9</sup> | 5.00 <sup>+0.84</sup> <sub>-0.96</sub> × 10 <sup>-11</sup> | 123.6 / 115  |
| 63.238                    | 0.45 <sup>+0.01</sup> <sub>-0.02</sub>                 | 47.1 <sup>+3.4</sup> <sub>-0.1</sub>  | 0.434 <sup>+0.063</sup> <sub>-0.095</sub> | 1.150 <sup>+0.137</sup> <sub>-0.140</sub>  | 3.68 <sup>+0.02</sup> <sub>-0.01</sub> × 10 <sup>-9</sup> | 3.83 <sup>+0.75</sup> <sub>-0.30</sub> × 10 <sup>-11</sup> | 120.1 / 125  |
| 63.839                    | 0.49 <sup>+0.02</sup> <sub>-0.02</sub>                 | 45.5 <sup>+0.2</sup> <sub>-0.6</sub>  | 0.359 <sup>+0.069</sup> <sub>-0.075</sub> | 0.962 <sup>+0.161</sup> <sub>-0.136</sub>  | 3.42 <sup>+0.02</sup> <sub>-0.01</sub> × 10 <sup>-9</sup> | 3.19 <sup>+0.47</sup> <sub>-0.43</sub> × 10 <sup>-11</sup> | 150.7 / 132  |
| 63.906                    | 0.41 <sup>+0.02</sup> <sub>-0.03</sub>                 | 49.0 <sup>+0.6</sup> <sub>-1.4</sub>  | 0.368 <sup>+0.043</sup> <sub>-0.037</sub> | 1.285 <sup>+0.302</sup> <sub>-0.204</sub>  | 3.62 <sup>+0.02</sup> <sub>-0.01</sub> × 10 <sup>-9</sup> | 4.73 <sup>+0.54</sup> <sub>-0.51</sub> × 10 <sup>-11</sup> | 209.5 / 143  |
| 64.178                    | 0.51 <sup>+0.02</sup> <sub>-0.01</sub>                 | 45.3 <sup>+1.6</sup> <sub>-0.5</sub>  | 0.289 <sup>+0.010</sup> <sub>-0.036</sub> | 1.159 <sup>+2.831</sup> <sub>-0.804</sub>  | 3.42 <sup>+0.02</sup> <sub>-0.01</sub> × 10 <sup>-9</sup> | 5.79 <sup>+1.25</sup> <sub>-0.91</sub> × 10 <sup>-11</sup> | 137.7 / 141  |
| 64.241                    | 0.46 <sup>+0.01</sup> <sub>-0.01</sub>                 | 44.9 <sup>+1.1</sup> <sub>-0.4</sub>  | 0.373 <sup>+0.035</sup> <sub>-0.031</sub> | 1.085 <sup>+0.333</sup> <sub>-0.314</sub>  | 4.08 <sup>+0.03</sup> <sub>-0.01</sub> × 10 <sup>-9</sup> | 7.43 <sup>+0.83</sup> <sub>-0.78</sub> × 10 <sup>-11</sup> | 154.6 / 129  |
| 65.783                    | 0.49 <sup>+0.05</sup> <sub>-0.01</sub>                 | 46.0 <sup>+1.1</sup> <sub>-0.1</sub>  | 0.346 <sup>+0.020</sup> <sub>-0.031</sub> | 1.695 <sup>+2.146</sup> <sub>-0.788</sub>  | 2.99 <sup>+0.01</sup> <sub>-0.01</sub> × 10 <sup>-9</sup> | 4.39 <sup>+0.55</sup> <sub>-0.84</sub> × 10 <sup>-11</sup> | 149.4 / 153  |
| 65.848                    | 0.45 <sup>+0.01</sup> <sub>-0.03</sub>                 | 47.9 <sup>+1.8</sup> <sub>-1.5</sub>  | 0.369 <sup>+0.054</sup> <sub>-0.039</sub> | 1.022 <sup>+0.049</sup> <sub>-0.083</sub>  | 3.03 <sup>+0.02</sup> <sub>-0.01</sub> × 10 <sup>-9</sup> | 4.00 <sup>+0.38</sup> <sub>-0.38</sub> × 10 <sup>-11</sup> | 181.0 / 157  |
| 65.918                    | 0.52 <sup>+0.02</sup> <sub>-0.01</sub>                 | 46.1 <sup>+2.9</sup> <sub>-1.4</sub>  | 0.386 <sup>+0.045</sup> <sub>-0.045</sub> | —                                          | 3.19 <sup>+0.02</sup> <sub>-0.01</sub> × 10 <sup>-9</sup> | 3.13 <sup>+0.41</sup> <sub>-0.34</sub> × 10 <sup>-11</sup> | 198.1 / 155  |
| 66.788                    | 0.43 <sup>+0.02</sup> <sub>-0.04</sub>                 | 50.1 <sup>+4.1</sup> <sub>-0.1</sub>  | 0.199 <sup>+0.016</sup> <sub>-0.040</sub> | 1.210 <sup>+0.201</sup> <sub>-0.164</sub>  | 3.13 <sup>+0.02</sup> <sub>-0.01</sub> × 10 <sup>-9</sup> | 4.92 <sup>+1.24</sup> <sub>-1.05</sub> × 10 <sup>-11</sup> | 126.9 / 144  |
| 66.856                    | 0.46 <sup>+0.03</sup> <sub>-0.01</sub>                 | 46.5 <sup>+2.0</sup> <sub>-1.7</sub>  | 0.395 <sup>+0.038</sup> <sub>-0.033</sub> | 0.936 <sup>+0.317</sup> <sub>-0.209</sub>  | 3.23 <sup>+0.02</sup> <sub>-0.01</sub> × 10 <sup>-9</sup> | 4.38 <sup>+0.43</sup> <sub>-0.42</sub> × 10 <sup>-11</sup> | 142.3 / 151  |
| 66.922                    | 0.42 <sup>+0.01</sup> <sub>-0.02</sub>                 | 50.9 <sup>+4.9</sup> <sub>-3.4</sub>  | 0.318 <sup>+0.044</sup> <sub>-0.046</sub> | 0.968 <sup>+0.251</sup> <sub>-0.157</sub>  | 3.22 <sup>+0.02</sup> <sub>-0.01</sub> × 10 <sup>-9</sup> | 4.57 <sup>+0.70</sup> <sub>-0.66</sub> × 10 <sup>-11</sup> | 157.4 / 135  |
| 66.99                     | 0.46 <sup>+0.02</sup> <sub>-0.03</sub>                 | 47.8 <sup>+2.4</sup> <sub>-3.4</sub>  | 0.335 <sup>+0.034</sup> <sub>-0.029</sub> | —                                          | 3.26 <sup>+0.02</sup> <sub>-0.01</sub> × 10 <sup>-9</sup> | 4.63 <sup>+0.57</sup> <sub>-0.42</sub> × 10 <sup>-11</sup> | 135.0 / 144  |
| 67.178                    | 0.40 <sup>+0.02</sup> <sub>-0.01</sub>                 | 49.1 <sup>+1.6</sup> <sub>-2.4</sub>  | 0.340 <sup>+0.053</sup> <sub>-0.029</sub> | 1.353 <sup>+1.704</sup> <sub>-0.935</sub>  | 3.12 <sup>+0.02</sup> <sub>-0.01</sub> × 10 <sup>-9</sup> | 4.07 <sup>+0.48</sup> <sub>-0.44</sub> × 10 <sup>-11</sup> | 138.1 / 127  |
| 68.323                    | 0.47 <sup>+0.01</sup> <sub>-0.01</sub>                 | 45.4 <sup>+2.2</sup> <sub>-0.6</sub>  | 0.327 <sup>+0.039</sup> <sub>-0.034</sub> | 1.036 <sup>+0.095</sup> <sub>-0.075</sub>  | 2.87 <sup>+0.01</sup> <sub>-0.01</sub> × 10 <sup>-9</sup> | 3.74 <sup>+0.34</sup> <sub>-0.30</sub> × 10 <sup>-11</sup> | 282.5 / 193  |
| 68.39                     | 0.49 <sup>+0.01</sup> <sub>-0.02</sub>                 | 42.7 <sup>+1.9</sup> <sub>-0.1</sub>  | 0.312 <sup>+0.036</sup> <sub>-0.032</sub> | 1.005 <sup>+0.056</sup> <sub>-0.070</sub>  | 2.70 <sup>+0.01</sup> <sub>-0.01</sub> × 10 <sup>-9</sup> | 3.74 <sup>+0.26</sup> <sub>-0.38</sub> × 10 <sup>-11</sup> | 245.1 / 180  |
| 69.327                    | 0.35 <sup>+0.01</sup> <sub>-0.02</sub>                 | 49.9 <sup>+1.5</sup> <sub>-0.6</sub>  | 0.301 <sup>+0.066</sup> <sub>-0.079</sub> | 0.899 <sup>+0.070</sup> <sub>-0.083</sub>  | 2.68 <sup>+0.01</sup> <sub>-0.01</sub> × 10 <sup>-9</sup> | 3.11 <sup>+0.71</sup> <sub>-0.40</sub> × 10 <sup>-11</sup> | 222.3 / 165  |
| 69.394                    | 0.45 <sup>+0.02</sup> <sub>-0.03</sub>                 | 46.2 <sup>+1.8</sup> <sub>-1.1</sub>  | 0.293 <sup>+0.031</sup> <sub>-0.035</sub> | 0.820 <sup>+0.272</sup> <sub>-0.177</sub>  | 2.66 <sup>+0.01</sup> <sub>-0.01</sub> × 10 <sup>-9</sup> | 3.99 <sup>+0.42</sup> <sub>-0.36</sub> × 10 <sup>-11</sup> | 148.6 / 161  |
| 70.264                    | 0.40 <sup>+0.02</sup> <sub>-0.02</sub>                 | 47.6 <sup>+0.3</sup> <sub>-1.0</sub>  | 0.375 <sup>+0.064</sup> <sub>-0.051</sub> | 0.961 <sup>+0.059</sup> <sub>-0.078</sub>  | 2.57 <sup>+0.01</sup> <sub>-0.01</sub> × 10 <sup>-9</sup> | 2.62 <sup>+0.16</sup> <sub>-0.18</sub> × 10 <sup>-11</sup> | 243.2 / 173  |
| 70.331                    | 0.52 <sup>+0.02</sup> <sub>-0.02</sub>                 | 44.8 <sup>+1.4</sup> <sub>-4.5</sub>  | 0.228 <sup>+0.048</sup> <sub>-0.048</sub> | 0.524 <sup>+0.214</sup> <sub>-0.327</sub>  | 2.57 <sup>+0.01</sup> <sub>-0.01</sub> × 10 <sup>-9</sup> | 4.12 <sup>+0.47</sup> <sub>-0.47</sub> × 10 <sup>-11</sup> | 184.6 / 165  |
| 72.011                    | 0.48 <sup>+0.02</sup> <sub>-0.04</sub>                 | 43.0 <sup>+4.5</sup> <sub>-0.6</sub>  | 0.330 <sup>+0.074</sup> <sub>-0.042</sub> | 1.029 <sup>+0.134</sup> <sub>-0.121</sub>  | 2.20 <sup>+0.01</sup> <sub>-0.01</sub> × 10 <sup>-9</sup> | 2.25 <sup>+0.36</sup> <sub>-0.32</sub> × 10 <sup>-11</sup> | 162.8 / 143  |
| 72.079                    | 0.55 <sup>+0.02</sup> <sub>-0.04</sub>                 | 43.8 <sup>+3.2</sup> <sub>-1.5</sub>  | 0.286 <sup>+0.054</sup> <sub>-0.051</sub> | 1.291 <sup>+0.851</sup> <sub>-0.192</sub>  | 2.16 <sup>+0.01</sup> <sub>-0.01</sub> × 10 <sup>-9</sup> | 2.95 <sup>+0.35</sup> <sub>-0.57</sub> × 10 <sup>-11</sup> | 170.6 / 146  |
| 72.146                    | 0.40 <sup>+0.01</sup> <sub>-0.03</sub>                 | 48.2 <sup>+2.3</sup> <sub>-3.9</sub>  | 0.275 <sup>+0.016</sup> <sub>-0.021</sub> | 1.146 <sup>+0.289</sup> <sub>-0.254</sub>  | 2.14 <sup>+0.01</sup> <sub>-0.01</sub> × 10 <sup>-9</sup> | 2.86 <sup>+0.52</sup> <sub>-0.49</sub> × 10 <sup>-11</sup> | 144.7 / 147  |
| 72.953                    | 0.53 <sup>+0.04</sup> <sub>-0.08</sub>                 | 45.5 <sup>+7.0</sup> <sub>-1.8</sub>  | 0.276 <sup>+1.096</sup> <sub>-0.276</sub> | 1.195 <sup>+1.163</sup> <sub>-0.550</sub>  | 2.16 <sup>+0.03</sup> <sub>-0.01</sub> × 10 <sup>-9</sup> | 1.89 <sup>+0.59</sup> <sub>-0.53</sub> × 10 <sup>-11</sup> | 90.4 / 86    |
| 73.083                    | 0.52 <sup>+0.01</sup> <sub>-0.06</sub>                 | 42.4 <sup>+3.1</sup> <sub>-0.8</sub>  | 0.307 <sup>+0.014</sup> <sub>-0.027</sub> | 1.095 <sup>+1.381</sup> <sub>-1.095</sub>  | 2.22 <sup>+0.01</sup> <sub>-0.01</sub> × 10 <sup>-9</sup> | 3.18 <sup>+0.57</sup> <sub>-0.25</sub> × 10 <sup>-11</sup> | 124.2 / 137  |
| 73.885                    | 0.44 <sup>+0.03</sup> <sub>-0.03</sub>                 | 46.7 <sup>+9.7</sup> <sub>-3.6</sub>  | 0.228 <sup>+0.076</sup> <sub>-0.076</sub> | 1.027 <sup>+0.336</sup> <sub>-0.209</sub>  | 2.31 <sup>+0.02</sup> <sub>-0.01</sub> × 10 <sup>-9</sup> | 3.13 <sup>+0.79</sup> <sub>-0.79</sub> × 10 <sup>-11</sup> | 86.1 / 112   |
| 73.952                    | 0.37 <sup>+0.03</sup> <sub>-0.05</sub>                 | 49.5 <sup>+5.4</sup> <sub>-0.4</sub>  | 0.319 <sup>+0.035</sup> <sub>-0.047</sub> | —                                          | 2.20 <sup>+0.02</sup> <sub>-0.01</sub> × 10 <sup>-9</sup> | 3.48 <sup>+0.56</sup> <sub>-0.47</sub> × 10 <sup>-11</sup> | 101.3 / 121  |
| 74.084                    | 0.40 <sup>+0.02</sup> <sub>-0.01</sub>                 | 48.8 <sup>+10.</sup> <sub>-1.0</sub>  | 0.368 <sup>+0.413</sup> <sub>-0.368</sub> | 0.864 <sup>+0.081</sup> <sub>-0.095</sub>  | 1.97 <sup>+0.01</sup> <sub>-0.01</sub> × 10 <sup>-9</sup> | 2.43 <sup>+0.58</sup> <sub>-0.35</sub> × 10 <sup>-11</sup> | 79.6 / 122   |
| 74.148                    | 0.47 <sup>+0.04</sup> <sub>-0.03</sub>                 | 44.1 <sup>+2.2</sup> <sub>-0.3</sub>  | 0.299 <sup>+0.032</sup> <sub>-0.030</sub> | —                                          | 2.00 <sup>+0.01</sup> <sub>-0.01</sub> × 10 <sup>-9</sup> | 3.60 <sup>+0.37</sup> <sub>-0.50</sub> × 10 <sup>-11</sup> | 139.1 / 133  |
| 74.828                    | 0.35 <sup>+0.03</sup> <sub>-0.06</sub>                 | 51.5 <sup>+8.1</sup> <sub>-3.0</sub>  | 0.303 <sup>+0.067</sup> <sub>-0.132</sub> | —                                          | 1.74 <sup>+0.02</sup> <sub>-0.01</sub> × 10 <sup>-9</sup> | 2.37 <sup>+1.21</sup> <sub>-0.49</sub> × 10 <sup>-11</sup> | 105.9 / 110  |
| 74.887                    | 0.46 <sup>+0.05</sup> <sub>-0.04</sub>                 | 46.4 <sup>+4.8</sup> <sub>-2.9</sub>  | 0.265 <sup>+0.045</sup> <sub>-0.045</sub> | 1.018 <sup>+0.453</sup> <sub>-0.210</sub>  | 1.81 <sup>+0.01</sup> <sub>-0.01</sub> × 10 <sup>-9</sup> | 2.55 <sup>+0.40</sup> <sub>-0.30</sub> × 10 <sup>-11</sup> | 142.0 / 163  |
| 76.895                    | 0.46 <sup>+0.02</sup> <sub>-0.05</sub>                 | 44.9 <sup>+6.6</sup> <sub>-0.5</sub>  | 0.348 <sup>+0.042</sup> <sub>-0.043</sub> | 0.849 <sup>+1.782</sup> <sub>-0.415</sub>  | 1.86 <sup>+0.01</sup> <sub>-0.01</sub> × 10 <sup>-9</sup> | 2.27 <sup>+0.22</sup> <sub>-0.21</sub> × 10 <sup>-11</sup> | 222.0 / 151  |
| 76.961                    | 0.34 <sup>+0.01</sup> <sub>-0.01</sub>                 | 47.0 <sup>+2.9</sup> <sub>-1.2</sub>  | 0.212 <sup>+0.704</sup> <sub>-0.212</sub> | 0.473 <sup>+0.067</sup> <sub>-0.068</sub>  | 1.80 <sup>+0.01</sup> <sub>-0.01</sub> × 10 <sup>-9</sup> | 2.48 <sup>+0.31</sup> <sub>-0.46</sub> × 10 <sup>-11</sup> | 153.3 / 136  |
| 77.028                    | 0.30 <sup>+0.01</sup> <sub>-0.01</sub>                 | 48.5 <sup>+1.9</sup> <sub>-2.1</sub>  | 0.340 <sup>+0.047</sup> <sub>-0.065</sub> | —                                          | 1.76 <sup>+0.01</sup> <sub>-0.01</sub> × 10 <sup>-9</sup> | 2.14 <sup>+0.38</sup> <sub>-0.33</sub> × 10 <sup>-11</sup> | 168.9 / 124  |
| 78.826                    | 0.45 <sup>+0.02</sup> <sub>-0.03</sub>                 | 43.4 <sup>+3.1</sup> <sub>-1.6</sub>  | 0.205 <sup>+0.150</sup> <sub>-0.076</sub> | 0.652 <sup>+0.146</sup> <sub>-0.120</sub>  | 1.36 <sup>+0.01</sup> <sub>-0.01</sub> × 10 <sup>-9</sup> | 2.26 <sup>+0.58</sup> <sub>-0.23</sub> × 10 <sup>-11</sup> | 173.9 / 139  |
| 80.176                    | 0.36 <sup>+0.07</sup> <sub>-0.07</sub>                 | 47.5 <sup>+14.3</sup> <sub>-9.2</sub> | 0.409 <sup>+0.080</sup> <sub>-0.096</sub> | 0.982 <sup>+3.441</sup> <sub>-0.215</sub>  | 1.24 <sup>+0.01</sup> <sub>-0.01</sub> × 10 <sup>-9</sup> | 2.12 <sup>+0.62</sup> <sub>-0.25</sub> × 10 <sup>-11</sup> | 94.1 / 118   |
| 80.236                    | 0.38 <sup>+0.05</sup> <sub>-0.03</sub>                 | 45.4 <sup>+3.1</sup> <sub>-0.3</sub>  | 0.190 <sup>+0.074</sup> <sub>-0.044</sub> | 0.678 <sup>+0.062</sup> <sub>-0.045</sub>  | 1.23 <sup>+0.02</sup> <sub>-0.01</sub> × 10 <sup>-9</sup> | 1.90 <sup>+0.55</sup> <sub>-0.55</sub> × 10 <sup>-11</sup> | 171.7 / 145  |
| 80.299                    | 0.35 <sup>+0.01</sup> <sub>-0.02</sub>                 | 44.6 <sup>+4.3</sup> <sub>-0.1</sub>  | 0.193 <sup>+0.154</sup> <sub>-0.021</sub> | 0.630 <sup>+0.144</sup> <sub>-0.137</sub>  | 1.30 <sup>+0.02</sup> <sub>-0.01</sub> × 10 <sup>-9</sup> | 2.51 <sup>+0.67</sup> <sub>-0.62</sub> × 10 <sup>-11</sup> | 116.4 / 114  |
| <b>2021 eruption</b>      |                                                        |                                       |                                           |                                            |                                                           |                                                            |              |
| 0.371                     | 21.84 <sup>+2.25</sup> <sub>-1.91</sub>                | —                                     | 0.354 <sup>+0.052</sup> <sub>-0.043</sub> | 5.805 <sup>+0.616</sup> <sub>-0.767</sub>  | —                                                         | 4.75 <sup>+0.13</sup> <sub>-1.50</sub> × 10 <sup>-10</sup> | 626.9 / 673  |
| 0.415                     | 28.11 <sup>+4.45</sup> <sub>-3.61</sub>                | —                                     | 0.277 <sup>+0.075</sup> <sub>-0.025</sub> | 5.733 <sup>+1.159</sup> <sub>-1.515</sub>  | —                                                         | 5.86 <sup>+0.48</sup> <sub>-3.70</sub> × 10 <sup>-10</sup> | 295.6 / 421  |
| 1.229                     | 8.89 <sup>+0.48</sup> <sub>-0.45</sub>                 | —                                     | 0.164 <sup>+0.025</sup> <sub>-0.032</sub> | 6.219 <sup>+0.600</sup> <sub>-0.516</sub>  | —                                                         | 7.27 <sup>+0.15</sup> <sub>-1.40</sub> × 10 <sup>-10</sup> | 769.1 / 778  |
| 2.892                     | 8.57 <sup>+0.36</sup> <sub>-0.38</sub>                 | —                                     | 0.186 <sup>+0.011</sup> <sub>-0.008</sub> | 8.149 <sup>+0.652</sup> <sub>-0.435</sub>  | —                                                         | 1.09 <sup>+0.02</sup> <sub>-0.10</sub> × 10 <sup>-9</sup>  | 956.3 / 834  |
| 4.01                      | 3.84 <sup>+0.18</sup> <sub>-0.13</sub>                 | —                                     | 0.125 <sup>+0.000</sup> <sub>-0.125</sub> | 12.570 <sup>+1.331</sup> <sub>-1.573</sub> | —                                                         | 1.27 <sup>+0.01</sup> <sub>-0.10</sub> × 10 <sup>-9</sup>  | 1023.9 / 835 |
| 4.21                      | 4.07 <sup>+0.37</sup> <sub>-0.32</sub>                 | —                                     | 0.133 <sup>+0.029</sup> <sub>-0.133</sub> | 8.166 <sup>+0.900</sup> <sub>-0.816</sub>  | —                                                         | 7.57 <sup>+0.18</sup> <sub>-2.80</sub> × 10 <sup>-10</sup> | 635.0 / 657  |
| 4.683                     | 2.76 <sup>+0.32</sup> <sub>-0.39</sub>                 | —                                     | 0.249 <sup>+0.063</sup> <sub>-0.033</sub> | —                                          | —                                                         | 1.30 <sup>+0.03</sup> <sub>-0.30</sub> × 10 <sup>-9</sup>  | 980.8 / 815  |

Continued on next page

Table 2 – continued from previous page

| T <sub>mid</sub><br>(day) | N <sub>H</sub><br>(10 <sup>22</sup> cm <sup>-2</sup> ) | kT <sub>BB</sub><br>(eV)               | APEC kT <sub>cool</sub><br>(keV)          | APEC kT <sub>hot</sub><br>(keV)             | BB Flux<br>(erg cm <sup>-2</sup> s <sup>-1</sup> )         | APEC Flux<br>(erg cm <sup>-2</sup> s <sup>-1</sup> )       | Cstat/dof   |
|---------------------------|--------------------------------------------------------|----------------------------------------|-------------------------------------------|---------------------------------------------|------------------------------------------------------------|------------------------------------------------------------|-------------|
| 5.675                     | 3.00 <sup>+0.17</sup> <sub>-0.20</sub>                 | —                                      | 0.177 <sup>+0.037</sup> <sub>-0.021</sub> | 20.620 <sup>+11.181</sup> <sub>-4.377</sub> | —                                                          | 1.22 <sup>+0.03</sup> <sub>-0.20</sub> × 10 <sup>-9</sup>  | 792.0 / 802 |
| 5.682                     | 3.89 <sup>+0.05</sup> <sub>-0.04</sub>                 | —                                      | 0.147 <sup>+0.013</sup> <sub>-0.013</sub> | 7.780 <sup>+0.561</sup> <sub>-0.487</sub>   | —                                                          | 9.32 <sup>+0.18</sup> <sub>-2.20</sub> × 10 <sup>-10</sup> | 706.4 / 713 |
| 6.605                     | 2.85 <sup>+0.11</sup> <sub>-0.15</sub>                 | —                                      | 0.150 <sup>+0.018</sup> <sub>-0.011</sub> | 9.238 <sup>+0.794</sup> <sub>-0.761</sub>   | —                                                          | 1.06 <sup>+0.01</sup> <sub>-0.20</sub> × 10 <sup>-9</sup>  | 851.8 / 762 |
| 6.612                     | 2.41 <sup>+0.33</sup> <sub>-0.32</sub>                 | —                                      | 0.263 <sup>+0.053</sup> <sub>-0.068</sub> | 12.296 <sup>+4.614</sup> <sub>-2.572</sub>  | —                                                          | 1.00 <sup>+0.03</sup> <sub>-0.19</sub> × 10 <sup>-9</sup>  | 687.9 / 717 |
| 9.988                     | 1.72 <sup>+0.12</sup> <sub>-0.13</sub>                 | —                                      | 0.739 <sup>+0.046</sup> <sub>-0.047</sub> | 4.662 <sup>+0.366</sup> <sub>-0.287</sub>   | —                                                          | 3.59 <sup>+0.06</sup> <sub>-0.50</sub> × 10 <sup>-10</sup> | 669.6 / 646 |
| 9.995                     | 2.14 <sup>+0.15</sup> <sub>-0.17</sub>                 | —                                      | 0.208 <sup>+0.065</sup> <sub>-0.045</sub> | 3.787 <sup>+0.406</sup> <sub>-0.219</sub>   | —                                                          | 6.07 <sup>+0.13</sup> <sub>-1.20</sub> × 10 <sup>-10</sup> | 676.9 / 710 |
| 10.519                    | 1.75 <sup>+0.12</sup> <sub>-0.14</sub>                 | —                                      | 0.708 <sup>+0.063</sup> <sub>-0.076</sub> | 3.640 <sup>+0.220</sup> <sub>-0.197</sub>   | —                                                          | 5.13 <sup>+0.11</sup> <sub>-1.20</sub> × 10 <sup>-10</sup> | 601.3 / 628 |
| 10.526                    | 1.67 <sup>+0.12</sup> <sub>-0.12</sub>                 | —                                      | 0.670 <sup>+0.059</sup> <sub>-0.079</sub> | 4.335 <sup>+0.285</sup> <sub>-0.242</sub>   | —                                                          | 3.43 <sup>+0.11</sup> <sub>-0.40</sub> × 10 <sup>-10</sup> | 767.8 / 653 |
| 11.846                    | 1.66 <sup>+0.12</sup> <sub>-0.13</sub>                 | —                                      | 0.740 <sup>+0.049</sup> <sub>-0.060</sub> | 3.631 <sup>+0.238</sup> <sub>-0.205</sub>   | —                                                          | 4.64 <sup>+0.11</sup> <sub>-1.20</sub> × 10 <sup>-10</sup> | 590.8 / 620 |
| 11.853                    | 1.97 <sup>+0.14</sup> <sub>-0.16</sub>                 | —                                      | 0.714 <sup>+0.050</sup> <sub>-0.061</sub> | 3.635 <sup>+0.403</sup> <sub>-0.295</sub>   | —                                                          | 3.65 <sup>+0.13</sup> <sub>-1.10</sub> × 10 <sup>-10</sup> | 522.8 / 562 |
| 12.576                    | 1.59 <sup>+0.12</sup> <sub>-0.14</sub>                 | —                                      | 0.694 <sup>+0.044</sup> <sub>-0.048</sub> | 3.398 <sup>+0.222</sup> <sub>-0.192</sub>   | —                                                          | 2.91 <sup>+0.09</sup> <sub>-0.60</sub> × 10 <sup>-10</sup> | 674.6 / 586 |
| 12.583                    | 1.66 <sup>+0.10</sup> <sub>-0.10</sub>                 | —                                      | 0.743 <sup>+0.040</sup> <sub>-0.047</sub> | 3.172 <sup>+0.157</sup> <sub>-0.107</sub>   | —                                                          | 3.16 <sup>+0.06</sup> <sub>-0.30</sub> × 10 <sup>-10</sup> | 643.5 / 622 |
| 13.571                    | 1.76 <sup>+0.10</sup> <sub>-0.10</sub>                 | —                                      | 0.792 <sup>+0.032</sup> <sub>-0.036</sub> | 2.892 <sup>+0.208</sup> <sub>-0.164</sub>   | —                                                          | 3.69 <sup>+0.11</sup> <sub>-0.90</sub> × 10 <sup>-10</sup> | 555.5 / 544 |
| 13.578                    | 1.78 <sup>+0.09</sup> <sub>-0.10</sub>                 | —                                      | 0.655 <sup>+0.051</sup> <sub>-0.063</sub> | 2.807 <sup>+0.146</sup> <sub>-0.136</sub>   | —                                                          | 4.33 <sup>+0.09</sup> <sub>-0.90</sub> × 10 <sup>-10</sup> | 619.5 / 599 |
| 14.7                      | 1.67 <sup>+0.09</sup> <sub>-0.11</sub>                 | —                                      | 0.658 <sup>+0.041</sup> <sub>-0.041</sub> | 2.623 <sup>+0.156</sup> <sub>-0.131</sub>   | —                                                          | 3.40 <sup>+0.07</sup> <sub>-0.80</sub> × 10 <sup>-10</sup> | 563.7 / 544 |
| 14.707                    | 1.77 <sup>+0.12</sup> <sub>-0.15</sub>                 | —                                      | 0.755 <sup>+0.047</sup> <sub>-0.050</sub> | 2.706 <sup>+0.343</sup> <sub>-0.247</sub>   | —                                                          | 3.47 <sup>+0.12</sup> <sub>-1.20</sub> × 10 <sup>-10</sup> | 462.4 / 488 |
| 15.629                    | 1.77 <sup>+0.08</sup> <sub>-0.09</sub>                 | —                                      | 0.772 <sup>+0.032</sup> <sub>-0.042</sub> | 2.799 <sup>+0.285</sup> <sub>-0.220</sub>   | —                                                          | 3.19 <sup>+0.08</sup> <sub>-0.80</sub> × 10 <sup>-10</sup> | 559.4 / 522 |
| 15.636                    | 1.52 <sup>+0.09</sup> <sub>-0.10</sub>                 | —                                      | 0.656 <sup>+0.036</sup> <sub>-0.045</sub> | 2.403 <sup>+0.129</sup> <sub>-0.111</sub>   | —                                                          | 3.26 <sup>+0.07</sup> <sub>-0.80</sub> × 10 <sup>-10</sup> | 578.7 / 553 |
| 16.557                    | 1.85 <sup>+0.17</sup> <sub>-0.19</sub>                 | —                                      | 0.659 <sup>+0.124</sup> <sub>-0.141</sub> | 1.964 <sup>+0.505</sup> <sub>-0.259</sub>   | —                                                          | 2.26 <sup>+0.12</sup> <sub>-1.40</sub> × 10 <sup>-10</sup> | 246.7 / 284 |
| 16.562                    | 1.51 <sup>+0.08</sup> <sub>-0.09</sub>                 | —                                      | 0.744 <sup>+0.029</sup> <sub>-0.032</sub> | 2.474 <sup>+0.147</sup> <sub>-0.114</sub>   | —                                                          | 3.20 <sup>+0.07</sup> <sub>-0.70</sub> × 10 <sup>-10</sup> | 618.5 / 551 |
| 17.552                    | 1.51 <sup>+0.12</sup> <sub>-0.15</sub>                 | —                                      | 0.723 <sup>+0.045</sup> <sub>-0.051</sub> | 2.427 <sup>+0.416</sup> <sub>-0.285</sub>   | —                                                          | 2.05 <sup>+0.07</sup> <sub>-0.90</sub> × 10 <sup>-10</sup> | 295.1 / 347 |
| 17.559                    | 1.48 <sup>+0.10</sup> <sub>-0.13</sub>                 | —                                      | 0.710 <sup>+0.044</sup> <sub>-0.042</sub> | 2.160 <sup>+0.130</sup> <sub>-0.130</sub>   | —                                                          | 1.90 <sup>+0.07</sup> <sub>-0.40</sub> × 10 <sup>-10</sup> | 490.6 / 467 |
| 18.681                    | 1.47 <sup>+0.13</sup> <sub>-0.15</sub>                 | —                                      | 0.667 <sup>+0.066</sup> <sub>-0.071</sub> | 2.201 <sup>+0.416</sup> <sub>-0.247</sub>   | —                                                          | 2.04 <sup>+0.08</sup> <sub>-0.70</sub> × 10 <sup>-10</sup> | 371.7 / 354 |
| 18.688                    | 1.50 <sup>+0.09</sup> <sub>-0.09</sub>                 | —                                      | 0.618 <sup>+0.041</sup> <sub>-0.045</sub> | 2.304 <sup>+0.243</sup> <sub>-0.157</sub>   | —                                                          | 2.13 <sup>+0.04</sup> <sub>-0.70</sub> × 10 <sup>-10</sup> | 414.6 / 444 |
| 19.478                    | 1.25 <sup>+0.06</sup> <sub>-0.29</sub>                 | —                                      | 0.143 <sup>+0.004</sup> <sub>-0.007</sub> | 1.598 <sup>+0.110</sup> <sub>-0.100</sub>   | —                                                          | 1.75 <sup>+0.10</sup> <sub>-1.80</sub> × 10 <sup>-10</sup> | 168.7 / 213 |
| 19.484                    | 1.40 <sup>+0.06</sup> <sub>-0.07</sub>                 | —                                      | 0.625 <sup>+0.036</sup> <sub>-0.043</sub> | 2.029 <sup>+0.096</sup> <sub>-0.085</sub>   | —                                                          | 2.39 <sup>+0.04</sup> <sub>-0.40</sub> × 10 <sup>-10</sup> | 707.0 / 528 |
| 20.605                    | 1.56 <sup>+0.06</sup> <sub>-0.06</sub>                 | 28.1 <sup>+5.9</sup> <sub>-0.4</sub>   | 0.788 <sup>+0.027</sup> <sub>-0.031</sub> | 2.338 <sup>+0.428</sup> <sub>-0.236</sub>   | 1.33 <sup>+0.29</sup> <sub>-0.21</sub> × 10 <sup>-11</sup> | 2.34 <sup>+0.10</sup> <sub>-0.80</sub> × 10 <sup>-10</sup> | 372.0 / 365 |
| 20.613                    | 1.68 <sup>+0.09</sup> <sub>-0.08</sub>                 | 75.8 <sup>+24.7</sup> <sub>-14.9</sub> | 0.887 <sup>+0.039</sup> <sub>-0.039</sub> | 2.254 <sup>+0.662</sup> <sub>-0.303</sub>   | 1.57 <sup>+0.13</sup> <sub>-0.13</sub> × 10 <sup>-11</sup> | 2.44 <sup>+0.04</sup> <sub>-0.30</sub> × 10 <sup>-10</sup> | 481.3 / 507 |
| 21.734                    | 1.46 <sup>+0.04</sup> <sub>-0.04</sub>                 | 38.4 <sup>+0.9</sup> <sub>-5.2</sub>   | 0.669 <sup>+0.041</sup> <sub>-0.015</sub> | 2.049 <sup>+0.361</sup> <sub>-0.219</sub>   | 1.06 <sup>+0.25</sup> <sub>-0.41</sub> × 10 <sup>-11</sup> | 2.12 <sup>+0.13</sup> <sub>-0.90</sub> × 10 <sup>-10</sup> | 287.4 / 309 |
| 21.741                    | 1.46 <sup>+0.07</sup> <sub>-0.07</sub>                 | 78.6 <sup>+48.4</sup> <sub>-20.5</sub> | 0.846 <sup>+0.042</sup> <sub>-0.031</sub> | 2.035 <sup>+0.230</sup> <sub>-0.165</sub>   | 1.32 <sup>+0.16</sup> <sub>-0.16</sub> × 10 <sup>-11</sup> | 2.25 <sup>+0.06</sup> <sub>-0.50</sub> × 10 <sup>-10</sup> | 467.5 / 470 |
| 22.529                    | 1.78 <sup>+0.06</sup> <sub>-0.08</sub>                 | 62.6 <sup>+39.3</sup> <sub>-8.0</sub>  | 0.811 <sup>+0.052</sup> <sub>-0.055</sub> | —                                           | 1.31 <sup>+0.16</sup> <sub>-0.34</sub> × 10 <sup>-11</sup> | 1.78 <sup>+0.06</sup> <sub>-0.60</sub> × 10 <sup>-10</sup> | 280.5 / 311 |
| 23.121                    | 1.72 <sup>+0.08</sup> <sub>-0.07</sub>                 | 99.3 <sup>+3.2</sup> <sub>-10.4</sub>  | 0.927 <sup>+0.036</sup> <sub>-0.050</sub> | —                                           | 1.56 <sup>+0.22</sup> <sub>-0.17</sub> × 10 <sup>-11</sup> | 1.83 <sup>+0.10</sup> <sub>-0.90</sub> × 10 <sup>-10</sup> | 244.4 / 301 |
| 23.126                    | 1.55 <sup>+0.05</sup> <sub>-0.03</sub>                 | 96.9 <sup>+2.4</sup> <sub>-2.8</sub>   | 0.836 <sup>+0.037</sup> <sub>-0.041</sub> | 2.077 <sup>+0.398</sup> <sub>-0.235</sub>   | 1.32 <sup>+0.21</sup> <sub>-0.20</sub> × 10 <sup>-11</sup> | 2.01 <sup>+0.06</sup> <sub>-0.50</sub> × 10 <sup>-10</sup> | 355.5 / 393 |
| 23.66                     | 1.56 <sup>+0.15</sup> <sub>-0.05</sub>                 | 96.7 <sup>+9.5</sup> <sub>-4.5</sub>   | 0.844 <sup>+0.040</sup> <sub>-0.028</sub> | 2.263 <sup>+0.341</sup> <sub>-0.369</sub>   | 1.56 <sup>+0.19</sup> <sub>-0.18</sub> × 10 <sup>-11</sup> | 1.87 <sup>+0.03</sup> <sub>-0.40</sub> × 10 <sup>-10</sup> | 413.1 / 386 |
| 23.666                    | 1.65 <sup>+0.04</sup> <sub>-0.07</sub>                 | 80.9 <sup>+31.5</sup> <sub>-22.0</sub> | 0.913 <sup>+0.029</sup> <sub>-0.035</sub> | —                                           | 1.42 <sup>+0.13</sup> <sub>-0.19</sub> × 10 <sup>-11</sup> | 2.02 <sup>+0.06</sup> <sub>-0.54</sub> × 10 <sup>-10</sup> | 415.5 / 375 |
| 23.992                    | 1.79 <sup>+0.02</sup> <sub>-0.07</sub>                 | 64.2 <sup>+36.4</sup> <sub>-1.2</sub>  | 0.560 <sup>+0.035</sup> <sub>-0.032</sub> | —                                           | 8.98 <sup>+1.62</sup> <sub>-1.79</sub> × 10 <sup>-12</sup> | 2.17 <sup>+0.09</sup> <sub>-1.20</sub> × 10 <sup>-10</sup> | 307.0 / 319 |
| 23.999                    | 1.58 <sup>+0.09</sup> <sub>-0.09</sub>                 | 82.8 <sup>+36.9</sup> <sub>-19.9</sub> | 0.785 <sup>+0.013</sup> <sub>-0.013</sub> | 3.658 <sup>+3.457</sup> <sub>-1.124</sub>   | 1.57 <sup>+0.17</sup> <sub>-0.15</sub> × 10 <sup>-11</sup> | 2.61 <sup>+0.06</sup> <sub>-0.70</sub> × 10 <sup>-10</sup> | 370.5 / 398 |
| 24.788                    | 1.59 <sup>+0.02</sup> <sub>-0.02</sub>                 | 50.4 <sup>+50.1</sup> <sub>-13.9</sub> | 0.688 <sup>+0.027</sup> <sub>-0.028</sub> | 1.726 <sup>+0.243</sup> <sub>-0.184</sub>   | 1.17 <sup>+0.23</sup> <sub>-0.17</sub> × 10 <sup>-11</sup> | 1.77 <sup>+0.06</sup> <sub>-0.60</sub> × 10 <sup>-10</sup> | 355.2 / 361 |
| 25.12                     | 1.59 <sup>+0.09</sup> <sub>-0.07</sub>                 | 87.4 <sup>+52.6</sup> <sub>-8.6</sub>  | 0.803 <sup>+0.021</sup> <sub>-0.038</sub> | 3.255 <sup>+14.486</sup> <sub>-9.14</sub>   | 1.71 <sup>+0.22</sup> <sub>-0.18</sub> × 10 <sup>-11</sup> | 1.73 <sup>+0.06</sup> <sub>-0.30</sub> × 10 <sup>-10</sup> | 338.9 / 382 |
| 25.128                    | 1.52 <sup>+0.01</sup> <sub>-0.06</sub>                 | 71.0 <sup>+13.3</sup> <sub>-22.0</sub> | —                                         | 2.523 <sup>+0.337</sup> <sub>-0.601</sub>   | 1.59 <sup>+0.16</sup> <sub>-0.16</sub> × 10 <sup>-11</sup> | 1.76 <sup>+0.06</sup> <sub>-0.30</sub> × 10 <sup>-10</sup> | 408.4 / 396 |
| 25.908                    | 1.19 <sup>+0.02</sup> <sub>-0.05</sub>                 | 22.7 <sup>+0.2</sup> <sub>-3.0</sub>   | 0.706 <sup>+0.023</sup> <sub>-0.030</sub> | 1.756 <sup>+0.111</sup> <sub>-0.095</sub>   | 1.49 <sup>+0.09</sup> <sub>-0.10</sub> × 10 <sup>-11</sup> | 1.73 <sup>+0.05</sup> <sub>-0.40</sub> × 10 <sup>-10</sup> | 365.8 / 347 |
| 25.913                    | 1.40 <sup>+0.06</sup> <sub>-0.05</sub>                 | 65.0 <sup>+16.5</sup> <sub>-3.2</sub>  | 0.823 <sup>+0.028</sup> <sub>-0.037</sub> | 1.479 <sup>+0.205</sup> <sub>-0.159</sub>   | 2.01 <sup>+0.13</sup> <sub>-0.20</sub> × 10 <sup>-11</sup> | 1.67 <sup>+0.04</sup> <sub>-0.50</sub> × 10 <sup>-10</sup> | 307.6 / 345 |
| 26.303                    | 0.90 <sup>+0.02</sup> <sub>-0.03</sub>                 | 21.3 <sup>+0.4</sup> <sub>-0.4</sub>   | 0.619 <sup>+0.032</sup> <sub>-0.062</sub> | 1.447 <sup>+0.048</sup> <sub>-0.042</sub>   | 8.69 <sup>+0.23</sup> <sub>-0.24</sub> × 10 <sup>-11</sup> | 1.57 <sup>+0.03</sup> <sub>-0.40</sub> × 10 <sup>-10</sup> | 393.3 / 358 |
| 26.309                    | 0.35 <sup>+0.05</sup> <sub>-0.06</sub>                 | 31.3 <sup>+0.1</sup> <sub>-1.1</sub>   | 0.792 <sup>+0.025</sup> <sub>-0.044</sub> | 1.884 <sup>+0.082</sup> <sub>-0.087</sub>   | 7.93 <sup>+0.24</sup> <sub>-0.23</sub> × 10 <sup>-11</sup> | 1.80 <sup>+0.05</sup> <sub>-0.40</sub> × 10 <sup>-10</sup> | 407.4 / 339 |
| 26.714                    | 1.36 <sup>+0.10</sup> <sub>-0.03</sub>                 | 28.3 <sup>+0.4</sup> <sub>-9.7</sub>   | 0.746 <sup>+0.029</sup> <sub>-0.024</sub> | 1.680 <sup>+0.196</sup> <sub>-0.183</sub>   | 1.83 <sup>+0.13</sup> <sub>-0.13</sub> × 10 <sup>-11</sup> | 1.52 <sup>+0.04</sup> <sub>-0.40</sub> × 10 <sup>-10</sup> | 390.6 / 319 |
| 26.72                     | 1.93 <sup>+0.01</sup> <sub>-0.08</sub>                 | 48.6 <sup>+8.7</sup> <sub>-8.7</sub>   | 0.853 <sup>+0.052</sup> <sub>-0.053</sub> | —                                           | 2.44 <sup>+0.24</sup> <sub>-0.28</sub> × 10 <sup>-11</sup> | 1.59 <sup>+0.05</sup> <sub>-0.52</sub> × 10 <sup>-10</sup> | 316.0 / 282 |
| 27.307                    | 1.19 <sup>+0.05</sup> <sub>-0.05</sub>                 | 41.3 <sup>+2.0</sup> <sub>-26.3</sub>  | 0.671 <sup>+0.055</sup> <sub>-0.039</sub> | 1.576 <sup>+0.293</sup> <sub>-0.208</sub>   | 1.83 <sup>+0.39</sup> <sub>-0.33</sub> × 10 <sup>-11</sup> | 1.54 <sup>+0.07</sup> <sub>-0.60</sub> × 10 <sup>-10</sup> | 243.9 / 283 |
| 27.314                    | 1.35 <sup>+0.03</sup> <sub>-0.03</sub>                 | 28.1 <sup>+11.8</sup> <sub>-0.2</sub>  | 0.591 <sup>+0.018</sup> <sub>-0.032</sub> | 1.674 <sup>+0.189</sup> <sub>-0.071</sub>   | 1.32 <sup>+0.10</sup> <sub>-0.14</sub> × 10 <sup>-11</sup> | 1.69 <sup>+0.05</sup> <sub>-0.40</sub> × 10 <sup>-10</sup> | 354.7 / 351 |
| 27.9                      | 1.86 <sup>+0.16</sup> <sub>-0.11</sub>                 | 91.5 <sup>+35.2</sup> <sub>-23.9</sub> | 0.229 <sup>+0.229</sup> <sub>-0.042</sub> | 0.988 <sup>+0.062</sup> <sub>-0.293</sub>   | 1.43 <sup>+0.18</sup> <sub>-0.13</sub> × 10 <sup>-11</sup> | 1.40 <sup>+0.04</sup> <sub>-0.05</sub> × 10 <sup>-10</sup> | 275.8 / 324 |
| 27.907                    | 1.34 <sup>+0.06</sup> <sub>-0.06</sub>                 | 35.5 <sup>+6.0</sup> <sub>-5.3</sub>   | 0.594 <sup>+0.042</sup> <sub>-0.042</sub> | 1.820 <sup>+0.212</sup> <sub>-0.517</sub>   | 1.31 <sup>+0.17</sup> <sub>-0.17</sub> × 10 <sup>-11</sup> | 1.49 <sup>+0.05</sup> <sub>-0.40</sub> × 10 <sup>-10</sup> | 291.7 / 314 |
| 28.036                    | 1.41 <sup>+0.06</sup> <sub>-0.06</sub>                 | 48.9 <sup>+1.3</sup> <sub>-4.9</sub>   | 0.675 <sup>+0.042</sup> <sub>-0.038</sub> | 1.943 <sup>+0.241</sup> <sub>-0.191</sub>   | 1.17 <sup>+0.11</sup> <sub>-0.11</sub> × 10 <sup>-11</sup> | 1.41 <sup>+0.04</sup> <sub>-0.40</sub> × 10 <sup>-10</sup> | 330.1 / 335 |
| 28.043                    | 1.25 <sup>+0.07</sup> <sub>-0.06</sub>                 | 41.7 <sup>+7.0</sup> <sub>-26.8</sub>  | 0.631 <sup>+0.030</sup> <sub>-0.042</sub> | 1.490 <sup>+0.191</sup> <sub>-0.208</sub>   | 1.26 <sup>+0.27</sup> <sub>-0.29</sub> × 10 <sup>-11</sup> | 1.38 <sup>+0.05</sup> <sub>-0.40</sub> × 10 <sup>-10</sup> | 270.8 / 317 |
| 28.902                    | 1.84 <sup>+0.16</sup> <sub>-0.16</sub>                 | 56.0 <sup>f</sup>                      | 0.204 <sup>+0.204</sup> <sub>-0.204</sub> | 0.853 <sup>+0.039</sup> <sub>-0.039</sub>   | 2.03 <sup>+0.13</sup> <sub>-0.17</sub> × 10 <sup>-11</sup> | 1.29 <sup>+0.03</sup> <sub>-0.03</sub> × 10 <sup>-10</sup> | 278.2 / 308 |
| 28.908                    | 1.25 <sup>+0.04</sup> <sub>-0.07</sub>                 | 69.2 <sup>+31.1</sup> <sub>-9.9</sub>  | 0.740 <sup>+0.028</sup> <sub>-0.048</sub> | 1.437 <sup>+0.232</sup> <sub>-0.118</sub>   | 2.00 <sup>+0.26</sup> <sub>-0.30</sub> × 10 <sup>-11</sup> | 1.30 <sup>+0.02</sup> <sub>-0.30</sub> × 10 <sup>-10</sup> | 317.6 / 328 |
| 29.162                    | 1.83 <sup>+0.12</sup> <sub>-0.11</sub>                 | 48.0 <sup>f</sup>                      | 0.228 <sup>+0.228</sup> <sub>-0.228</sub> | 0.958 <sup>+0.078</sup> <sub>-0.958</sub>   | 2.66 <sup>+0.20</sup> <sub>-0.22</sub> × 10 <sup>-11</sup> | 1.34 <sup>+0.04</sup> <sub>-0.04</sub> × 10 <sup>-10</sup> | 278.2 / 308 |
| 29.169                    | 1.33 <sup>+0.03</sup> <sub>-0.05</sub>                 | 27.6 <sup>+2.8</sup> <sub>-0.3</sub>   | 0.589 <sup>+0.025</sup> <sub>-0.031</sub> | 1.719 <sup>+0.216</sup> <sub>-0.158</sub>   | 2.07 <sup>+0.19</sup> <sub>-0.19</sub> × 10 <sup>-11</sup> | 1.61 <sup>+0.07</sup> <sub>-0.50</sub> × 10 <sup>-10</sup> | 288.0 / 314 |
| 29.693                    | 1.96 <sup>+0.15</sup> <sub>-0.12</sub>                 | 68.5 <sup>+9.5</sup> <sub>-17.9</sub>  | 0.234 <sup>+0.025</sup> <sub>-0.031</sub> | 1.008 <sup>+0.078</sup> <sub>-0.067</sub>   | 1.55 <sup>+0.18</sup> <sub>-0.17</sub> × 10 <sup>-11</sup> | 1.26 <sup>+0.04</sup> <sub>-0.40</sub> × 10 <sup>-10</sup> | 325.2 / 302 |

Continued on next page

Table 2 – continued from previous page

| $T_{\text{mid}}$<br>(day) | $N_{\text{H}}$<br>( $10^{22} \text{ cm}^{-2}$ ) | $kT_{\text{BB}}$<br>(eV) | APEC $kT_{\text{cool}}$<br>(keV) | APEC $kT_{\text{hot}}$<br>(keV) | BB Flux<br>( $\text{erg cm}^{-2} \text{ s}^{-1}$ ) | APEC Flux<br>( $\text{erg cm}^{-2} \text{ s}^{-1}$ ) | Cstat/dof   |
|---------------------------|-------------------------------------------------|--------------------------|----------------------------------|---------------------------------|----------------------------------------------------|------------------------------------------------------|-------------|
| 29.699                    | $1.03^{+0.05}_{-0.05}$                          | $33.8^{+0.7}_{-1.4}$     | $0.668^{+0.037}_{-0.044}$        | $1.518^{+0.161}_{-0.105}$       | $1.19^{+0.20}_{-0.14} \times 10^{-11}$             | $1.31^{+0.06}_{-0.30} \times 10^{-10}$               | 275.1 / 276 |
| 30.288                    | $0.64^{+0.03}_{-0.01}$                          | $27.4^{+2.6}_{-2.0}$     | $0.762^{+0.049}_{-0.047}$        | $1.516^{+0.086}_{-0.085}$       | $1.85^{+0.05}_{-0.04} \times 10^{-10}$             | $1.34^{+0.04}_{-0.40} \times 10^{-10}$               | 372.7 / 330 |
| 30.296                    | $0.39^{+0.14}_{-0.11}$                          | $35.6^{+6.1}_{-5.3}$     | $0.741^{+0.122}_{-0.148}$        | $1.499^{+0.125}_{-0.090}$       | $1.73^{+0.05}_{-0.05} \times 10^{-10}$             | $1.19^{+0.04}_{-0.40} \times 10^{-10}$               | 316.6 / 267 |
| 30.749                    | $0.57^{+0.17}_{-0.01}$                          | $27.9^{+0.7}_{-5.6}$     | $0.763^{+0.036}_{-0.073}$        | $1.483^{+0.123}_{-0.101}$       | $6.92^{+0.32}_{-0.35} \times 10^{-11}$             | $1.26^{+0.06}_{-0.60} \times 10^{-10}$               | 247.5 / 239 |
| 30.754                    | $1.01^{+0.01}_{-0.01}$                          | $22.5^{+1.3}_{-0.4}$     | $0.646^{+0.025}_{-0.028}$        | $1.330^{+0.039}_{-0.043}$       | $5.82^{+0.17}_{-0.17} \times 10^{-11}$             | $1.26^{+0.05}_{-0.40} \times 10^{-10}$               | 345.2 / 307 |
| 30.815                    | $1.39^{+0.07}_{-0.03}$                          | $26.8^{+0.3}_{-0.7}$     | $0.598^{+0.047}_{-0.058}$        | $1.331^{+0.186}_{-0.103}$       | $2.65^{+0.22}_{-0.19} \times 10^{-11}$             | $1.31^{+0.06}_{-0.50} \times 10^{-10}$               | 294.5 / 267 |
| 30.82                     | $1.68^{+0.11}_{-0.17}$                          | $20.9^{+2.2}_{-1.1}$     | —                                | $1.085^{+0.095}_{-0.085}$       | $1.75^{+0.17}_{-0.16} \times 10^{-11}$             | $1.12^{+0.04}_{-0.40} \times 10^{-10}$               | 273.4 / 276 |
| 31.746                    | $1.52^{+0.09}_{-0.08}$                          | $21.7^{+1.3}_{-1.0}$     | $0.633^{+0.043}_{-0.028}$        | —                               | $4.10^{+0.31}_{-0.25} \times 10^{-11}$             | $1.16^{+0.09}_{-0.60} \times 10^{-10}$               | 221.1 / 234 |
| 31.75                     | $1.00^{+0.16}_{-0.24}$                          | $24.8^{+1.1}_{-1.8}$     | $0.605^{+0.058}_{-0.054}$        | $1.498^{+0.244}_{-0.151}$       | $5.56^{+0.30}_{-0.28} \times 10^{-11}$             | $1.30^{+0.05}_{-0.60} \times 10^{-10}$               | 234.6 / 251 |
| 31.813                    | $0.76^{+0.10}_{-0.03}$                          | $25.1^{+0.9}_{-3.1}$     | $0.647^{+0.064}_{-0.065}$        | $1.427^{+0.088}_{-0.079}$       | $9.78^{+0.32}_{-0.45} \times 10^{-11}$             | $1.24^{+0.06}_{-0.50} \times 10^{-10}$               | 221.4 / 238 |
| 31.817                    | $0.38^{+0.14}_{-0.09}$                          | $32.3^{+2.5}_{-2.2}$     | $0.708^{+0.070}_{-0.067}$        | $1.586^{+0.099}_{-0.089}$       | $1.12^{+0.04}_{-0.04} \times 10^{-10}$             | $1.35^{+0.05}_{-0.50} \times 10^{-10}$               | 299.0 / 245 |
| 32.088                    | $0.62^{+0.01}_{-0.11}$                          | $27.6^{+0.1}_{-0.1}$     | $0.705^{+0.062}_{-0.065}$        | $1.552^{+0.205}_{-0.133}$       | $2.44^{+0.13}_{-0.13} \times 10^{-10}$             | $1.15^{+0.08}_{-0.20} \times 10^{-10}$               | 208.7 / 212 |
| 32.09                     | $0.44^{+0.10}_{-0.10}$                          | $44.9^{+8.6}_{-2.2}$     | $0.849^{+0.041}_{-0.063}$        | $1.512^{+0.149}_{-0.117}$       | $3.08^{+0.09}_{-0.09} \times 10^{-10}$             | $1.59^{+0.06}_{-0.60} \times 10^{-10}$               | 263.4 / 237 |
| 32.74                     | $0.74^{+0.22}_{-0.06}$                          | $35.1^{+13.4}_{-0.4}$    | $0.787^{+0.199}_{-0.128}$        | $1.324^{+0.296}_{-0.160}$       | $3.85^{+0.57}_{-0.40} \times 10^{-11}$             | $1.03^{+0.09}_{-0.77} \times 10^{-10}$               | 158.2 / 178 |
| 32.744                    | $1.20^{+0.09}_{-0.11}$                          | $23.6^{+1.6}_{-1.1}$     | $0.550^{+0.056}_{-0.055}$        | $1.341^{+0.319}_{-0.149}$       | $3.81^{+0.11}_{-0.19} \times 10^{-11}$             | $1.26^{+0.05}_{-0.30} \times 10^{-10}$               | 331.5 / 283 |
| 32.875                    | $1.00^{+0.17}_{-0.06}$                          | $24.5^{+0.7}_{-4.8}$     | $0.595^{+0.053}_{-0.094}$        | $1.163^{+0.454}_{-0.176}$       | $3.04^{+0.26}_{-0.28} \times 10^{-11}$             | $9.77^{+0.53}_{-0.40} \times 10^{-11}$               | 171.8 / 190 |
| 32.878                    | $1.19^{+0.07}_{-0.04}$                          | $23.5^{+1.1}_{-0.6}$     | $0.567^{+0.027}_{-0.043}$        | $1.341^{+0.154}_{-0.114}$       | $3.05^{+0.16}_{-0.15} \times 10^{-11}$             | $1.09^{+0.03}_{-0.30} \times 10^{-10}$               | 328.0 / 293 |
| 33.482                    | $0.70^{+0.09}_{-0.14}$                          | $30.0^{+1.6}_{-1.7}$     | $0.642^{+0.062}_{-0.055}$        | $1.287^{+0.092}_{-0.063}$       | $7.91^{+0.25}_{-0.25} \times 10^{-11}$             | $1.20^{+0.07}_{-0.20} \times 10^{-10}$               | 304.5 / 274 |
| 33.551                    | $0.84^{+0.11}_{-0.05}$                          | $26.1^{+0.4}_{-1.7}$     | $0.604^{+0.037}_{-0.040}$        | $1.360^{+0.085}_{-0.090}$       | $6.03^{+0.20}_{-0.20} \times 10^{-11}$             | $1.00^{+0.03}_{-0.27} \times 10^{-10}$               | 303.4 / 268 |
| 33.621                    | $0.94^{+0.01}_{-0.05}$                          | $26.5^{+0.1}_{-0.2}$     | $0.554^{+0.035}_{-0.033}$        | $1.402^{+0.120}_{-0.119}$       | $4.63^{+0.18}_{-0.18} \times 10^{-11}$             | $1.00^{+0.04}_{-0.27} \times 10^{-10}$               | 304.8 / 278 |
| 33.69                     | $0.74^{+0.05}_{-0.02}$                          | $22.3^{+0.3}_{-0.2}$     | $0.589^{+0.042}_{-0.079}$        | $1.266^{+0.188}_{-0.119}$       | $3.56^{+0.31}_{-0.27} \times 10^{-11}$             | $9.58^{+0.62}_{-0.53} \times 10^{-11}$               | 166.5 / 200 |
| 33.758                    | $0.27^{+0.11}_{-0.08}$                          | $31.3^{+3.6}_{-4.2}$     | $0.660^{+0.052}_{-0.060}$        | $1.544^{+0.070}_{-0.058}$       | $5.57^{+0.20}_{-0.19} \times 10^{-11}$             | $1.09^{+0.03}_{-0.27} \times 10^{-10}$               | 334.1 / 271 |
| 33.825                    | $0.31^{+0.03}_{-0.01}$                          | $34.8^{+1.6}_{-1.3}$     | $0.671^{+0.040}_{-0.040}$        | $1.669^{+0.083}_{-0.071}$       | $5.40^{+0.30}_{-0.19} \times 10^{-11}$             | $9.58^{+0.23}_{-0.34} \times 10^{-11}$               | 291.8 / 269 |
| 33.891                    | $0.24^{+0.05}_{-0.07}$                          | $41.3^{+13.2}_{-2.8}$    | $0.581^{+0.083}_{-0.082}$        | $1.554^{+0.097}_{-0.079}$       | $5.85^{+0.43}_{-0.37} \times 10^{-11}$             | $1.08^{+0.05}_{-0.50} \times 10^{-10}$               | 228.8 / 218 |
| 33.955                    | $0.77^{+0.07}_{-0.08}$                          | $25.1^{+1.4}_{-1.2}$     | $0.606^{+0.033}_{-0.036}$        | $1.428^{+0.079}_{-0.069}$       | $5.75^{+0.19}_{-0.19} \times 10^{-11}$             | $1.00^{+0.04}_{-0.25} \times 10^{-10}$               | 330.6 / 279 |
| 34.018                    | $1.05^{+0.02}_{-0.02}$                          | $24.1^{+0.1}_{-0.1}$     | $0.686^{+0.025}_{-0.032}$        | $1.286^{+0.152}_{-0.060}$       | $6.16^{+0.20}_{-0.19} \times 10^{-11}$             | $9.89^{+0.41}_{-0.31} \times 10^{-11}$               | 315.8 / 276 |
| 34.08                     | $0.92^{+0.09}_{-0.23}$                          | $27.1^{+1.0}_{-1.4}$     | $0.647^{+0.034}_{-0.041}$        | $1.349^{+0.092}_{-0.091}$       | $6.97^{+0.23}_{-0.21} \times 10^{-11}$             | $1.00^{+0.03}_{-0.26} \times 10^{-10}$               | 330.6 / 267 |
| 34.143                    | $0.91^{+0.05}_{-0.05}$                          | $26.1^{+0.7}_{-2.3}$     | $0.659^{+0.024}_{-0.037}$        | $1.543^{+0.171}_{-0.149}$       | $7.58^{+0.23}_{-0.22} \times 10^{-11}$             | $1.01^{+0.02}_{-0.31} \times 10^{-10}$               | 374.3 / 270 |
| 34.156                    | $0.39^{+0.09}_{-0.01}$                          | $37.8^{+0.2}_{-0.1}$     | $0.725^{+0.040}_{-0.040}$        | $1.488^{+0.057}_{-0.054}$       | $8.07^{+0.27}_{-0.21} \times 10^{-11}$             | $1.05^{+0.02}_{-0.40} \times 10^{-10}$               | 347.9 / 275 |
| 34.223                    | $1.24^{+0.01}_{-0.01}$                          | $23.4^{+0.3}_{-1.5}$     | $0.627^{+0.034}_{-0.043}$        | $1.815^{+0.515}_{-0.352}$       | $8.09^{+0.28}_{-0.27} \times 10^{-11}$             | $1.06^{+0.04}_{-0.30} \times 10^{-10}$               | 344.2 / 291 |
| 34.29                     | $0.70^{+0.01}_{-0.02}$                          | $30.4^{+0.6}_{-3.2}$     | $0.665^{+0.038}_{-0.052}$        | $1.413^{+0.067}_{-0.064}$       | $8.83^{+0.33}_{-0.26} \times 10^{-11}$             | $1.06^{+0.04}_{-0.30} \times 10^{-10}$               | 278.0 / 261 |
| 34.409                    | $1.04^{+0.03}_{-0.02}$                          | $23.7^{+0.4}_{-0.1}$     | $0.551^{+0.042}_{-0.049}$        | $1.262^{+0.122}_{-0.159}$       | $6.12^{+0.30}_{-0.29} \times 10^{-11}$             | $8.09^{+0.39}_{-0.39} \times 10^{-11}$               | 266.3 / 218 |
| 36.873                    | $0.34^{+0.01}_{-0.04}$                          | $31.7^{+4.6}_{-0.1}$     | $0.678^{+0.024}_{-0.049}$        | $1.502^{+0.050}_{-0.045}$       | $7.58^{+0.19}_{-0.17} \times 10^{-11}$             | $8.83^{+0.21}_{-0.24} \times 10^{-11}$               | 384.3 / 277 |
| 36.939                    | $0.80^{+0.05}_{-0.01}$                          | $25.1^{+0.6}_{-1.4}$     | $0.620^{+0.029}_{-0.020}$        | $1.358^{+0.092}_{-0.086}$       | $1.00^{+0.03}_{-0.02} \times 10^{-10}$             | $9.09^{+0.24}_{-0.24} \times 10^{-11}$               | 367.4 / 264 |
| 37.206                    | $0.72^{+0.08}_{-0.03}$                          | $28.8^{+0.5}_{-1.5}$     | $0.608^{+0.033}_{-0.019}$        | $1.396^{+0.088}_{-0.106}$       | $1.01^{+0.03}_{-0.02} \times 10^{-10}$             | $8.60^{+0.19}_{-0.21} \times 10^{-11}$               | 481.0 / 282 |
| 37.722                    | $0.38^{+0.01}_{-0.02}$                          | $29.5^{+0.3}_{-0.4}$     | $0.614^{+0.032}_{-0.024}$        | $1.499^{+0.068}_{-0.056}$       | $2.80^{+0.04}_{-0.03} \times 10^{-10}$             | $9.04^{+0.20}_{-0.27} \times 10^{-11}$               | 327.7 / 294 |
| 37.924                    | $0.36^{+0.02}_{-0.05}$                          | $33.7^{+1.3}_{-1.4}$     | $0.598^{+0.031}_{-0.038}$        | $1.385^{+0.043}_{-0.042}$       | $1.37^{+0.02}_{-0.03} \times 10^{-10}$             | $8.90^{+0.22}_{-0.21} \times 10^{-11}$               | 447.8 / 280 |
| 38.197                    | $0.42^{+0.01}_{-0.04}$                          | $32.6^{+1.3}_{-0.7}$     | $0.683^{+0.029}_{-0.030}$        | $1.534^{+0.087}_{-0.070}$       | $2.07^{+0.03}_{-0.02} \times 10^{-10}$             | $8.72^{+0.22}_{-0.21} \times 10^{-11}$               | 378.8 / 290 |
| 38.789                    | $0.36^{+0.04}_{-0.03}$                          | $42.9^{+3.1}_{-1.8}$     | $0.577^{+0.070}_{-0.074}$        | $1.511^{+0.091}_{-0.097}$       | $1.70^{+0.06}_{-0.04} \times 10^{-10}$             | $7.75^{+0.25}_{-0.37} \times 10^{-11}$               | 296.4 / 246 |
| 39.048                    | $0.28^{+0.02}_{-0.06}$                          | $44.2^{+6.2}_{-0.3}$     | $0.708^{+0.039}_{-0.032}$        | $1.560^{+0.084}_{-0.063}$       | $1.29^{+0.03}_{-0.02} \times 10^{-10}$             | $8.43^{+0.20}_{-0.30} \times 10^{-11}$               | 418.0 / 276 |
| 39.313                    | $0.31^{+0.02}_{-0.08}$                          | $46.9^{+0.5}_{-0.6}$     | $0.658^{+0.046}_{-0.048}$        | $1.447^{+0.056}_{-0.051}$       | $1.32^{+0.02}_{-0.02} \times 10^{-10}$             | $8.56^{+0.23}_{-0.48} \times 10^{-11}$               | 404.5 / 272 |
| 39.648                    | $0.41^{+0.03}_{-0.02}$                          | $42.7^{+4.9}_{-1.8}$     | $0.544^{+0.038}_{-0.040}$        | $1.295^{+0.055}_{-0.042}$       | $9.68^{+0.07}_{-0.07} \times 10^{-10}$             | $8.58^{+0.24}_{-0.23} \times 10^{-11}$               | 355.6 / 247 |
| 40.042                    | $0.75^{+0.04}_{-0.08}$                          | $44.8^{+2.7}_{-2.3}$     | $0.541^{+0.060}_{-0.099}$        | $1.157^{+0.255}_{-0.138}$       | $1.80^{+0.01}_{-0.01} \times 10^{-9}$              | $1.05^{+0.06}_{-0.25} \times 10^{-10}$               | 303.0 / 212 |
| 40.186                    | $0.29^{+0.01}_{-0.02}$                          | $35.0^{+0.3}_{-0.5}$     | $0.655^{+0.044}_{-0.036}$        | $1.584^{+0.117}_{-0.103}$       | $3.77^{+0.05}_{-0.05} \times 10^{-10}$             | $7.67^{+0.25}_{-0.37} \times 10^{-11}$               | 278.1 / 236 |
| 40.582                    | $0.32^{+0.01}_{-0.04}$                          | $41.2^{+4.4}_{-0.8}$     | $0.576^{+0.032}_{-0.030}$        | $1.549^{+0.100}_{-0.070}$       | $6.39^{+0.05}_{-0.06} \times 10^{-10}$             | $7.93^{+0.33}_{-0.17} \times 10^{-11}$               | 338.0 / 249 |
| 40.843                    | $0.29^{+0.04}_{-0.09}$                          | $66.5^{+17.2}_{-0.2}$    | $0.619^{+0.048}_{-0.046}$        | $1.585^{+0.167}_{-0.130}$       | $8.29^{+0.10}_{-0.09} \times 10^{-10}$             | $7.59^{+0.58}_{-0.77} \times 10^{-11}$               | 281.5 / 220 |
| 41.437                    | $0.31^{+0.03}_{-0.02}$                          | $52.7^{+3.8}_{-0.3}$     | $0.597^{+0.077}_{-0.041}$        | $1.366^{+0.074}_{-0.067}$       | $1.35^{+0.01}_{-0.01} \times 10^{-9}$              | $8.02^{+0.45}_{-0.36} \times 10^{-11}$               | 365.7 / 252 |
| 41.639                    | $0.44^{+0.02}_{-0.08}$                          | $39.7^{+4.3}_{-0.3}$     | $0.618^{+0.061}_{-0.048}$        | $1.281^{+0.083}_{-0.064}$       | $1.32^{+0.01}_{-0.01} \times 10^{-9}$              | $7.53^{+0.33}_{-0.30} \times 10^{-11}$               | 319.7 / 258 |
| 42.436                    | $0.35^{+0.02}_{-0.09}$                          | $40.0^{+4.5}_{-3.0}$     | $0.473^{+0.045}_{-0.059}$        | $1.811^{+0.272}_{-0.205}$       | $1.47^{+0.01}_{-0.01} \times 10^{-9}$              | $8.03^{+0.37}_{-0.41} \times 10^{-11}$               | 199.8 / 229 |
| 42.569                    | $0.36^{+0.03}_{-0.05}$                          | $43.8^{+7.0}_{-1.7}$     | $0.513^{+0.071}_{-0.077}$        | $1.448^{+0.213}_{-0.140}$       | $5.86^{+0.10}_{-0.10} \times 10^{-10}$             | $6.13^{+0.34}_{-0.53} \times 10^{-11}$               | 235.8 / 204 |
| 42.902                    | $0.39^{+0.04}_{-0.03}$                          | $52.6^{+3.8}_{-0.4}$     | $0.570^{+0.034}_{-0.035}$        | $1.468^{+0.147}_{-0.098}$       | $1.09^{+0.01}_{-0.01} \times 10^{-9}$              | $7.80^{+0.35}_{-0.27} \times 10^{-11}$               | 297.5 / 253 |
| 43.249                    | $0.36^{+0.01}_{-0.05}$                          | $44.3^{+2.7}_{-4.2}$     | $0.597^{+0.115}_{-0.080}$        | $1.216^{+0.062}_{-0.051}$       | $1.15^{+0.01}_{-0.01} \times 10^{-9}$              | $6.76^{+0.35}_{-0.32} \times 10^{-11}$               | 311.7 / 238 |
| 43.627                    | $0.19^{+0.01}_{-0.03}$                          | $49.5^{+0.1}_{-0.1}$     | $0.554^{+0.051}_{-0.033}$        | $1.596^{+0.118}_{-0.104}$       | $4.40^{+0.10}_{-0.07} \times 10^{-10}$             | $7.03^{+0.64}_{-0.63} \times 10^{-11}$               | 283.5 / 244 |
| 43.83                     | $0.23^{+0.01}_{-0.02}$                          | $44.9^{+2.2}_{-1.9}$     | $0.525^{+0.041}_{-0.039}$        | $1.715^{+0.153}_{-0.102}$       | $7.66^{+0.06}_{-0.07} \times 10^{-10}$             | $7.52^{+0.28}_{-0.39} \times 10^{-11}$               | 275.1 / 235 |
| 44.423                    | $0.65^{+0.05}_{-0.03}$                          | $46.2^{+5.2}_{-2.2}$     | $0.635^{+0.040}_{-0.052}$        | —                               | $2.36^{+0.02}_{-0.02} \times 10^{-9}$              | $8.03^{+0.48}_{-0.45} \times 10^{-11}$               | 205.1 / 196 |
| 44.823                    | $0.46^{+0.03}_{-0.06}$                          | $58.1^{+6.8}_{-0.1}$     | $0.487^{+0.057}_{-0.057}$        | $1.120^{+0.108}_{-0.098}$       | $2.51^{+0.01}_{-0.02} \times 10^{-9}$              | $7.89^{+0.48}_{-0.48} \times 10^{-11}$               | 277.1 / 210 |
| 44.491                    | $0.28^{+0.01}_{-0.01}$                          | $52.0^f$                 | $0.601^{+0.047}_{-0.052}$        | $1.556^{+0.206}_{-0.121}$       | $2.26^{+0.01}_{-0.01} \times 10^{-9}$              | $7.52^{+0.48}_{-0.39} \times 10^{-11}$               | 261.0 / 238 |

Continued on next page

Table 2 – continued from previous page

| $T_{\text{mid}}$<br>(day) | $N_{\text{H}}$<br>( $10^{22} \text{ cm}^{-2}$ ) | $kT_{\text{BB}}$<br>(eV) | APEC $kT_{\text{cool}}$<br>(keV) | APEC $kT_{\text{hot}}$<br>(keV) | BB Flux<br>( $\text{erg cm}^{-2} \text{ s}^{-1}$ ) | APEC Flux<br>( $\text{erg cm}^{-2} \text{ s}^{-1}$ ) | Cstat/dof   |
|---------------------------|-------------------------------------------------|--------------------------|----------------------------------|---------------------------------|----------------------------------------------------|------------------------------------------------------|-------------|
| 45.17                     | $0.38^{+0.02}_{-0.03}$                          | $59.6^{+9.6}_{-0.4}$     | $0.519^{+0.045}_{-0.022}$        | $1.621^{+0.467}_{-0.287}$       | $2.54^{+0.02}_{-0.01} \times 10^{-9}$              | $8.49^{+0.45}_{-0.51} \times 10^{-11}$               | 231.1 / 190 |
| 45.493                    | $0.39^{+0.01}_{-0.05}$                          | $55.3^{+7.0}_{-1.5}$     | $0.489^{+0.050}_{-0.041}$        | $1.367^{+0.170}_{-0.160}$       | $2.45^{+0.01}_{-0.01} \times 10^{-9}$              | $8.00^{+0.40}_{-0.47} \times 10^{-11}$               | 290.0 / 197 |
| 45.835                    | $0.40^{+0.01}_{-0.01}$                          | $53.0^f$                 | $0.546^{+0.088}_{-0.090}$        | $1.218^{+0.129}_{-0.096}$       | $2.46^{+0.01}_{-0.01} \times 10^{-9}$              | $6.97^{+0.55}_{-0.54} \times 10^{-11}$               | 195.4 / 187 |
| 46.164                    | $0.45^{+0.02}_{-0.07}$                          | $50.7^{+4.5}_{-1.3}$     | $0.551^{+0.056}_{-0.049}$        | $1.549^{+0.611}_{-0.299}$       | $2.33^{+0.02}_{-0.02} \times 10^{-9}$              | $8.01^{+0.43}_{-0.53} \times 10^{-11}$               | 282.4 / 191 |
| 46.812                    | $0.41^{+0.02}_{-0.05}$                          | $55.4^{+2.5}_{-3.0}$     | $0.461^{+0.067}_{-0.071}$        | $1.519^{+0.205}_{-0.164}$       | $2.08^{+0.01}_{-0.02} \times 10^{-9}$              | $6.20^{+0.67}_{-0.27} \times 10^{-11}$               | 247.3 / 182 |
| 47.159                    | $0.31^{+0.02}_{-0.02}$                          | $79.6^{+18.4}_{-25.6}$   | $0.485^{+0.071}_{-0.086}$        | $1.304^{+0.065}_{-0.093}$       | $2.70^{+0.02}_{-0.02} \times 10^{-9}$              | $7.45^{+0.48}_{-0.50} \times 10^{-11}$               | 208.6 / 186 |
| 47.485                    | $0.34^{+0.03}_{-0.05}$                          | $70.4^{+13.6}_{-13.3}$   | $0.537^{+0.049}_{-0.048}$        | $2.372^{+0.441}_{-0.883}$       | $2.12^{+0.01}_{-0.02} \times 10^{-9}$              | $7.73^{+0.73}_{-0.83} \times 10^{-11}$               | 193.2 / 186 |
| 48.155                    | $0.26^{+0.01}_{-0.02}$                          | $65.9^{+8.4}_{-8.4}$     | $0.514^{+0.049}_{-0.043}$        | $1.632^{+0.463}_{-0.230}$       | $1.22^{+0.01}_{-0.01} \times 10^{-9}$              | $6.02^{+0.33}_{-0.32} \times 10^{-11}$               | 317.2 / 220 |
| 48.479                    | $0.23^{+0.01}_{-0.01}$                          | $55.0^f$                 | $0.546^{+0.049}_{-0.070}$        | $1.253^{+0.192}_{-0.113}$       | $2.11^{+0.02}_{-0.02} \times 10^{-9}$              | $7.18^{+0.48}_{-0.46} \times 10^{-11}$               | 195.4 / 187 |
| 48.819                    | $0.43^{+0.02}_{-0.04}$                          | $43.2^{+4.1}_{-4.1}$     | $0.527^{+0.046}_{-0.025}$        | $1.245^{+0.091}_{-0.083}$       | $1.64^{+0.01}_{-0.01} \times 10^{-9}$              | $6.26^{+0.26}_{-0.16} \times 10^{-11}$               | 268.0 / 217 |
| 49.15                     | $0.07^{+0.04}_{-0.03}$                          | $79.8^{+24.4}_{-18.5}$   | $0.511^{+0.039}_{-0.037}$        | $1.597^{+0.140}_{-0.109}$       | $1.46^{+0.01}_{-0.01} \times 10^{-9}$              | $7.22^{+0.30}_{-0.17} \times 10^{-11}$               | 276.3 / 216 |
| 49.467                    | $0.45^{+0.03}_{-0.03}$                          | $45.9^{+3.2}_{-0.8}$     | $0.496^{+0.058}_{-0.058}$        | $1.057^{+0.082}_{-0.082}$       | $9.83^{+0.11}_{-0.13} \times 10^{-10}$             | $5.16^{+0.58}_{-0.48} \times 10^{-11}$               | 270.5 / 217 |
| 49.799                    | $0.49^{+0.01}_{-0.02}$                          | $58.2^{+5.6}_{-0.1}$     | $0.551^{+0.036}_{-0.021}$        | $1.050^{+0.169}_{-0.109}$       | $6.26^{+0.11}_{-0.11} \times 10^{-10}$             | $5.94^{+0.56}_{-0.53} \times 10^{-11}$               | 165.5 / 171 |
| 50.145                    | $0.36^{+0.01}_{-0.01}$                          | $51.0^f$                 | $0.479^{+0.051}_{-0.056}$        | $1.111^{+0.236}_{-0.090}$       | $1.69^{+0.01}_{-0.01} \times 10^{-9}$              | $6.41^{+0.48}_{-0.47} \times 10^{-11}$               | 264.3 / 224 |
| 50.464                    | $0.36^{+0.03}_{-0.14}$                          | $44.4^{+4.7}_{-1.9}$     | $0.585^{+0.164}_{-0.112}$        | $1.280^{+0.298}_{-0.130}$       | $6.23^{+0.14}_{-0.12} \times 10^{-10}$             | $3.30^{+0.78}_{-0.52} \times 10^{-11}$               | 122.8 / 143 |
| 50.802                    | $0.35^{+0.01}_{-0.07}$                          | $44.3^{+9.1}_{-2.1}$     | $0.568^{+0.029}_{-0.047}$        | —                               | $6.27^{+0.12}_{-0.11} \times 10^{-10}$             | $4.82^{+0.54}_{-0.61} \times 10^{-11}$               | 157.6 / 152 |
| 51.14                     | $0.40^{+0.01}_{-0.01}$                          | $44.0^f$                 | $0.721^{+0.036}_{-0.039}$        | —                               | $6.99^{+0.09}_{-0.09} \times 10^{-10}$             | $5.92^{+0.51}_{-0.40} \times 10^{-11}$               | 204.6 / 176 |
| 52.529                    | $0.27^{+0.10}_{-0.01}$                          | $41.3^{+0.6}_{-1.3}$     | $0.455^{+0.142}_{-0.086}$        | $1.434^{+0.359}_{-0.244}$       | $5.15^{+0.10}_{-0.12} \times 10^{-10}$             | $4.02^{+1.26}_{-0.53} \times 10^{-11}$               | 101.2 / 139 |
| 52.662                    | $0.25^{+0.06}_{-0.06}$                          | $46.3^{+4.9}_{-2.5}$     | $0.491^{+0.091}_{-0.089}$        | $1.538^{+0.568}_{-0.220}$       | $5.44^{+0.08}_{-0.07} \times 10^{-10}$             | $5.03^{+0.41}_{-0.39} \times 10^{-11}$               | 237.4 / 212 |
| 52.735                    | $0.25^{+0.07}_{-0.01}$                          | $50.9^{+3.9}_{-2.6}$     | $0.514^{+0.068}_{-0.054}$        | $1.453^{+0.149}_{-0.105}$       | $5.43^{+0.12}_{-0.10} \times 10^{-10}$             | $7.27^{+0.36}_{-0.38} \times 10^{-11}$               | 313.7 / 212 |
| 52.735                    | $0.25^{+0.07}_{-0.01}$                          | $50.9^{+3.9}_{-2.6}$     | $0.514^{+0.068}_{-0.054}$        | $1.453^{+0.149}_{-0.105}$       | $5.43^{+0.12}_{-0.10} \times 10^{-10}$             | $7.27^{+0.36}_{-0.38} \times 10^{-11}$               | 313.7 / 212 |
| 52.794                    | $0.20^{+0.02}_{-0.02}$                          | $49.0^f$                 | $0.665^{+0.177}_{-0.442}$        | $1.485^{+0.439}_{-0.216}$       | $5.00^{+0.10}_{-0.11} \times 10^{-10}$             | $4.42^{+0.51}_{-0.51} \times 10^{-11}$               | 106.2 / 140 |
| 52.918                    | $0.56^{+0.01}_{-0.03}$                          | $37.2^{+4.2}_{-0.3}$     | $0.548^{+0.042}_{-0.042}$        | $1.900^{+0.100}_{-0.373}$       | $6.91^{+0.11}_{-0.10} \times 10^{-10}$             | $6.42^{+0.10}_{-0.20} \times 10^{-11}$               | 356.9 / 216 |
| 55.575                    | $0.43^{+0.01}_{-0.01}$                          | $46.0^f$                 | $0.546^{+0.017}_{-0.011}$        | $1.391^{+0.152}_{-0.243}$       | $1.02^{+0.01}_{-0.01} \times 10^{-9}$              | $5.12^{+0.11}_{-0.12} \times 10^{-11}$               | 440.2 / 236 |
| 55.656                    | $0.42^{+0.03}_{-0.04}$                          | $54.2^{+5.0}_{-0.5}$     | $0.434^{+0.041}_{-0.030}$        | $1.502^{+0.365}_{-0.208}$       | $1.55^{+0.01}_{-0.01} \times 10^{-9}$              | $5.24^{+0.18}_{-0.16} \times 10^{-11}$               | 361.4 / 208 |
| 56.651                    | $0.44^{+0.01}_{-0.01}$                          | $48.0^f$                 | $0.457^{+0.015}_{-0.019}$        | $1.389^{+0.188}_{-0.091}$       | $1.54^{+0.01}_{-0.01} \times 10^{-9}$              | $5.58^{+0.19}_{-0.18} \times 10^{-11}$               | 226.9 / 208 |
| 57.515                    | $0.36^{+0.01}_{-0.01}$                          | $46.0^f$                 | $0.457^{+0.047}_{-0.036}$        | $1.350^{+0.150}_{-0.124}$       | $1.44^{+0.01}_{-0.01} \times 10^{-9}$              | $4.98^{+0.27}_{-0.27} \times 10^{-11}$               | 338.8 / 213 |
| 58.561                    | $0.41^{+0.02}_{-0.04}$                          | $45.6^{+1.0}_{-3.9}$     | $0.508^{+0.028}_{-0.027}$        | $1.214^{+0.133}_{-0.113}$       | $8.97^{+0.06}_{-0.06} \times 10^{-10}$             | $3.47^{+0.19}_{-0.26} \times 10^{-11}$               | 370.0 / 217 |
| 60.831                    | $0.29^{+0.01}_{-0.01}$                          | $45.0^f$                 | $0.536^{+0.034}_{-0.035}$        | $1.541^{+0.246}_{-0.170}$       | $8.64^{+0.05}_{-0.05} \times 10^{-10}$             | $3.67^{+0.18}_{-0.01} \times 10^{-11}$               | 311.0 / 218 |
| 61.563                    | $0.33^{+0.03}_{-0.05}$                          | $44.5^{+3.5}_{-0.7}$     | $0.524^{+0.047}_{-0.041}$        | $1.524^{+0.665}_{-0.440}$       | $2.29^{+0.03}_{-0.04} \times 10^{-10}$             | $2.88^{+0.22}_{-0.20} \times 10^{-11}$               | 250.7 / 217 |
| 63.886                    | $0.04^{+0.02}_{-0.01}$                          | $52.4^{+1.6}_{-1.4}$     | $0.515^{+0.037}_{-0.038}$        | $1.672^{+0.213}_{-0.175}$       | $1.83^{+0.03}_{-0.03} \times 10^{-10}$             | $3.02^{+0.16}_{-0.20} \times 10^{-11}$               | 216.0 / 200 |
| 64.614                    | $0.20^{+0.05}_{-0.04}$                          | $47.3^{+5.3}_{-0.8}$     | $0.512^{+0.017}_{-0.057}$        | $1.340^{+0.165}_{-0.167}$       | $2.16^{+0.05}_{-0.05} \times 10^{-10}$             | $2.59^{+0.25}_{-0.24} \times 10^{-11}$               | 155.2 / 147 |
| 65.545                    | $0.14^{+0.03}_{-0.05}$                          | $53.4^{+4.1}_{-0.9}$     | $0.543^{+0.044}_{-0.049}$        | $1.349^{+0.125}_{-0.113}$       | $2.17^{+0.07}_{-0.08} \times 10^{-10}$             | $2.71^{+0.24}_{-0.43} \times 10^{-11}$               | 125.2 / 129 |
| 66.656                    | $0.22^{+0.02}_{-0.01}$                          | $50.6^{+11.9}_{-3.3}$    | $0.561^{+0.058}_{-0.054}$        | $1.730^{+0.315}_{-0.447}$       | $2.14^{+0.07}_{-0.06} \times 10^{-10}$             | $1.99^{+0.33}_{-0.13} \times 10^{-11}$               | 163.2 / 138 |
| 67.006                    | $0.21^{+0.04}_{-0.09}$                          | $44.6^{+7.2}_{-2.2}$     | $0.219^{+0.661}_{-0.086}$        | $0.669^{+0.133}_{-0.112}$       | $1.85^{+0.03}_{-0.03} \times 10^{-10}$             | $2.40^{+0.17}_{-0.18} \times 10^{-11}$               | 219.4 / 211 |
| 67.271                    | $0.13^{+0.01}_{-0.01}$                          | $49.6^{+3.7}_{-1.5}$     | $0.685^{+0.076}_{-0.094}$        | $2.059^{+2.829}_{-0.540}$       | $1.71^{+0.03}_{-0.01} \times 10^{-10}$             | $2.45^{+0.17}_{-0.11} \times 10^{-11}$               | 214.4 / 192 |
| 69.393                    | $0.11^{+0.03}_{-0.03}$                          | $52.5^{+3.3}_{-1.7}$     | $0.544^{+0.022}_{-0.025}$        | $1.533^{+0.187}_{-0.133}$       | $1.76^{+0.03}_{-0.03} \times 10^{-10}$             | $2.46^{+0.25}_{-0.27} \times 10^{-11}$               | 196.6 / 173 |
| 69.594                    | $0.20^{+0.03}_{-0.03}$                          | $49.1^{+5.2}_{-0.6}$     | $0.617^{+0.058}_{-0.050}$        | $1.813^{+1.283}_{-0.459}$       | $1.27^{+0.05}_{-0.05} \times 10^{-10}$             | $1.71^{+0.28}_{-0.30} \times 10^{-11}$               | 96.8 / 109  |
| 70.655                    | $0.05^{+0.01}_{-0.01}$                          | $65.3^{+14.1}_{-0.3}$    | $0.525^{+0.043}_{-0.047}$        | $1.446^{+0.182}_{-0.134}$       | $1.12^{+0.02}_{-0.02} \times 10^{-10}$             | $2.35^{+0.11}_{-0.25} \times 10^{-11}$               | 203.8 / 192 |
| 72.573                    | $0.38^{+0.09}_{-0.15}$                          | $50.3^{+15.2}_{-10.8}$   | $0.457^{+0.151}_{-0.130}$        | $0.964^{+0.510}_{-0.964}$       | $1.16^{+0.02}_{-0.02} \times 10^{-10}$             | $1.92^{+0.11}_{-0.12} \times 10^{-11}$               | 177.3 / 171 |
| 72.58                     | $0.27^{+0.02}_{-0.02}$                          | $57.0^f$                 | $0.568^{+0.040}_{-0.050}$        | $1.719^{+0.538}_{-0.326}$       | $1.03^{+0.02}_{-0.02} \times 10^{-10}$             | $1.96^{+0.15}_{-0.15} \times 10^{-11}$               | 174.0 / 173 |
| 73.966                    | $0.25^{+0.02}_{-0.01}$                          | $57.0^f$                 | $0.542^{+0.078}_{-0.074}$        | $1.357^{+0.739}_{-0.265}$       | $1.12^{+0.02}_{-0.02} \times 10^{-10}$             | $2.14^{+0.23}_{-0.22} \times 10^{-11}$               | 209.0 / 215 |
| 74.638                    | $0.04^{+0.03}_{-0.04}$                          | $63.3^{+18.8}_{-15.2}$   | $0.616^{+0.055}_{-0.059}$        | $1.635^{+0.787}_{-0.349}$       | $1.01^{+0.04}_{-0.06} \times 10^{-10}$             | $1.68^{+1.05}_{-0.63} \times 10^{-11}$               | 97.3 / 105  |
| 75.567                    | $0.14^{+0.01}_{-0.01}$                          | $58.4^{+1.9}_{-0.3}$     | $0.547^{+0.045}_{-0.038}$        | $1.546^{+0.335}_{-0.185}$       | $8.97^{+0.23}_{-0.18} \times 10^{-11}$             | $1.57^{+0.08}_{-0.16} \times 10^{-11}$               | 167.9 / 170 |
| 76.688                    | $0.04^{+0.03}_{-0.02}$                          | $68.6^{+7.6}_{-10.9}$    | $0.585^{+0.228}_{-0.178}$        | $1.980^{+3.694}_{-0.640}$       | $7.37^{+0.26}_{-0.24} \times 10^{-11}$             | $1.59^{+0.14}_{-0.20} \times 10^{-11}$               | 122.5 / 142 |
| 76.695                    | $0.18^{+0.03}_{-0.03}$                          | $60.0^f$                 | $0.681^{+0.081}_{-0.081}$        | $1.457^{+0.017}_{-0.445}$       | $9.24^{+0.27}_{-0.26} \times 10^{-11}$             | $1.85^{+0.25}_{-0.25} \times 10^{-11}$               | 133.0 / 148 |
| 77.625                    | $0.16^{+0.03}_{-0.04}$                          | $49.7^{+4.6}_{-0.8}$     | $0.566^{+0.056}_{-0.098}$        | $0.980^{+0.129}_{-0.129}$       | $7.04^{+0.15}_{-0.15} \times 10^{-11}$             | $1.45^{+0.07}_{-0.18} \times 10^{-11}$               | 147.4 / 158 |
| 78.753                    | $0.13^{+0.03}_{-0.06}$                          | $48.9^{+13.1}_{-2.7}$    | $0.645^{+0.049}_{-0.046}$        | $1.443^{+0.533}_{-0.321}$       | $8.32^{+0.17}_{-0.17} \times 10^{-11}$             | $1.50^{+0.08}_{-0.09} \times 10^{-11}$               | 162.5 / 173 |
| 79.676                    | $0.26^{+0.03}_{-0.03}$                          | $53.0^f$                 | $0.610^{+0.082}_{-0.078}$        | $1.861^{+1.689}_{-1.053}$       | $7.26^{+0.24}_{-0.23} \times 10^{-11}$             | $1.52^{+0.14}_{-0.20} \times 10^{-11}$               | 125.0 / 143 |
| 80.941                    | $0.11^{+0.02}_{-0.05}$                          | $56.4^{+6.6}_{-16.0}$    | $0.724^{+0.050}_{-0.054}$        | $1.538^{+0.422}_{-0.249}$       | $7.19^{+0.15}_{-0.14} \times 10^{-11}$             | $1.35^{+0.07}_{-0.08} \times 10^{-11}$               | 186.8 / 169 |
| 81.674                    | $0.17^{+0.06}_{-0.01}$                          | $56.2^{+9.8}_{-6.0}$     | $0.757^{+0.043}_{-0.076}$        | $1.193^{+0.385}_{-0.268}$       | $4.80^{+0.99}_{-1.08} \times 10^{-11}$             | $3.09^{+0.95}_{-1.08} \times 10^{-11}$               | 124.7 / 137 |
